# Supplementary material for: Differential Invariants of Linear Symplectic Actions
Source: arXiv:2010.08024 ancillary file (2020-11-15)
Supplement: Supplementary file 1 [file Computations4D.pdf]

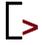

## Curves in 4-dimensions

**>** `with(DifferentialGeometry) : with(Tensor) : with(JetCalculus) : with(Tools) :`

**>** `DGsetup([t], [x, y, z], M, 4) :`

**M >** `Preferences("JetNotation", "JetNotation1") :`

**M >** `ω d evalDG(dt &w dy[ ] C dx[ ] &w dz[ ]`  
$$\omega d dt Y dy[ ] C dx[ ] Y dz[ ] \quad (1.1)$$

**Invariant vector v0**

**M >** `v0 d evalDG(t D_t C x[ ] D_x[ ] C y[ ] D_y[ ] C z[ ] D_z[ ]`  
$$v0 d t D_t C x[ ] D_x[ ] C y[ ] D_y[ ] C z[ ] D_z[ ] \quad (1.2)$$

**w1 corresponds the derivative of v0**

**M >** `w1 d evalDG(D_t C x[1] D_x[ ] C y[1] D_y[ ] C z[1] D_z[ ]`  
$$w1 d D_t C x_1 D_x[ ] C y_1 D_y[ ] C z_1 D_z[ ] \quad (1.3)$$

**here k1 corresponds to 1/β**

**M >** `v1 d evalDG(`
$$\frac{w1}{k1}$$
`)`  
$$v1 d \frac{D_t}{k1} C \frac{x_1 D_x[ ]}{k1} C \frac{y_1 D_y[ ]}{k1} C \frac{z_1 D_z[ ]}{k1} \quad (1.4)$$

**solve the normalization criterion to determine k1.**

**M >** `tmp1 d solve(Hook([v0, v1], ω) K 1, k1) :`

**substitute back into v1, thus giving v1 uniquely**

**M >** `v1 d subs(k1=tmp1, v1)`

**v1 d** 
$$\frac{D_t}{t y_1 C x[ ] z_1 K z[ ] x_1 K y[ ]} C \frac{x_1 D_x[ ]}{t y_1 C x[ ] z_1 K z[ ] x_1 K y[ ]}$$
  
$$C \frac{y_1 D_y[ ]}{t y_1 C x[ ] z_1 K z[ ] x_1 K y[ ]} C \frac{z_1 D_z[ ]}{t y_1 C x[ ] z_1 K z[ ] x_1 K y[ ]} \quad (1.5)$$

**input the derivative of the vector v0**

**M >** `w2 d evalDG(x[1, 1] D_x[ ] C y[1, 1] D_y[ ] C z[1, 1] D_z[ ] ) :`

**input the chain rule relation with v2**

**M >** `v2 d evalDG(`
$$\frac{w2 K k2 v1}{tmp1^2}$$
`)`  
**v2 d** 
$$k \frac{k2 D_t}{(t y_1 C x[ ] z_1 K x_1 z[ ] K y[ ] )^3}$$
  
$$K \frac{(K t x_{1,1} y_1 K x[ ] x_{1,1} z_1 C x_1 x_{1,1} z[ ] C k2 x_1 C x_{1,1} y[ ] ) D_x[ ]}{(t y_1 C x[ ] z_1 K x_1 z[ ] K y[ ] )^3}$$
  
$$K \frac{(K t y_{1,1} y_{1,1} K x[ ] y_{1,1} z_1 C x_1 y_{1,1} z[ ] C k2 y_1 C y[ ] y_{1,1} ) D_y[ ]}{(t y_1 C x[ ] z_1 K x_1 z[ ] K y[ ] )^3}$$
  
$$K \frac{(K t y_{1,1} z_{1,1} K x[ ] z_{1,1} z_1 C x_1 z[ ] z_{1,1} C k2 z_1 C y[ ] z_{1,1} ) D_z[ ]}{(t y_1 C x[ ] z_1 K x_1 z[ ] K y[ ] )^3} \quad (1.6)$$

**solve to obtain k2 and input it to get v2 uniquely**

**M >** `tmp2 d solve(Hook([v0, v2], ω), k2) :`

**M** > v2 d subs(k2=tmp2, v2) :

we can then calculate the first invariant by computing  $\omega(v1, v2)$

**M** > I<sub>2</sub> d Hook([v1, v2],  $\omega$ )

$$I_2 \text{ d } \frac{x_1 z_{1,1} K x_{1,1} z_1 C y_{1,1}}{(t y_1 C x[ ] z_1 K x_1 z[ ] K y[ ])^3} \quad (1.7)$$

same story, take the next derivative of v0, solve the chain rule relation and normalize to find k3 and substitute back into v3 to obtain v3 uniquely

**M** > w3 d evalDG(x[1, 1, 1] D\_x[ ] C y[1, 1, 1] D\_y[ ] C z[1, 1, 1] D\_z[ ] ) :

**M** > v3 d evalDG $\left(\frac{(w3 K 3 tmp1 tmp2 v2 K k3 v1)}{tmp1^3}\right)$  :

**M** > tmp3 d solve(Hook([v0, v3],  $\omega$ ), k3) :

then v3 is uniquely determined

**M** > v3 d simplify(subs(k3=tmp3, v3)) :

can now calculate more invariants, in fact two more

**M** > I<sub>3a</sub> d Hook([v1, v3],  $\omega$ ); I<sub>3b</sub> d Hook([v2, v3],  $\omega$ )

$$I_{3a} \text{ d } \frac{1}{(t y_1 C x[ ] z_1 K x_1 z[ ] K y[ ])^5} (t x_1 y_1 z_{1,1,1} K 3 t x_1 y_{1,1} z_{1,1} C 3 t x_{1,1} y_{1,1} z_1$$

$$K t x_{1,1,1} y_1 z_1 C x[ ] x_1 z_1 z_{1,1,1} K 3 x[ ] x_1 z_{1,1}^2 C 3 x[ ] x_{1,1} z_1 z_{1,1} K x[ ] x_{1,1,1} z_1^2$$

$$K x_1^2 z[ ] z_{1,1,1} C 3 x_1 x_{1,1} z[ ] z_{1,1} C x_1 x_{1,1,1} z[ ] z_1 K 3 x_{1,1}^2 z[ ] z_1 C t y_1 y_{1,1,1}$$

$$K 3 t y_{1,1}^2 K 3 x[ ] y_{1,1} z_{1,1} C y_{1,1,1} x[ ] z_1 K x_1 y[ ] z_{1,1,1} K y_{1,1,1} z[ ] x_1$$

$$C 3 x_{1,1} y_{1,1} z[ ] C x_{1,1,1} y[ ] z_1 K y[ ] y_{1,1,1})$$

$$I_{3b} \text{ d } k \frac{1}{(t y_1 C x[ ] z_1 K x_1 z[ ] K y[ ])^6} (t x_1 y_{1,1} z_{1,1,1} K t x_1 y_{1,1,1} z_{1,1} K t x_{1,1} y_1 z_{1,1,1} \quad (1.8)$$

$$C t x_{1,1} y_{1,1,1} z_1 C t x_{1,1,1} y_1 z_{1,1} K t x_{1,1,1} y_{1,1} z_1 K x[ ] y_{1,1} z_{1,1,1} C x[ ] y_{1,1,1} z_{1,1}$$

$$C x_{1,1} y[ ] z_{1,1,1} K x_{1,1} y_{1,1,1} z[ ] K x_{1,1,1} y[ ] z_{1,1} C x_{1,1,1} y_{1,1} z[ ] )$$

continue the same procedure again

**M** > w4 d evalDG(x[1, 1, 1, 1] D\_x[ ] C y[1, 1, 1, 1] D\_y[ ] C z[1, 1, 1, 1] D\_z[ ] ) :

**M** > v4 d evalDG $\left(\frac{w4 K 6 tmp1^2 tmp2 v3 K (4 tmp1 tmp3 C 3 tmp2^2) v2 K k4 v1}{tmp1^4}\right)$  :

**M** > tmp4 d solve(Hook([v0, v4],  $\omega$ ), k4) :

this gives ut v4 uniquely

**M** > v4 d subs(k4=tmp4, v4) :

we can then compute the final invariants

**M** > I<sub>4a</sub> d Hook([v1, v4],  $\omega$ )

$$I_{4a} \text{ d } \frac{1}{(t y_1 C x[ ] z_1 K x_1 z[ ] K y[ ])^7} (t^2 x_1 y_1^2 z_{1,1,1,1,1} K 6 t^2 x_1 y_1 y_{1,1} z_{1,1,1}$$

$$K 4 t^2 x_1 y_1 y_{1,1,1} z_{1,1} C 15 t^2 x_1 y_1^2 z_{1,1} C 4 t^2 x_{1,1} y_1 y_{1,1,1} z_1 K 15 t^2 x_{1,1} y_{1,1}^2 z_1$$

$$C 6 t^2 x_{1,1,1} y_1 y_{1,1} z_1 K t^2 x_{1,1,1,1} y_1^2 z_1 C 2 t x[ ] x_1 y_1 z_1 z_{1,1,1,1}$$

$$K 10 t x[ ] x_1 y_1 z_{1,1} z_{1,1,1} K 6 t x[ ] x_1 y_{1,1} z_1 z_{1,1,1} C 30 t x[ ] x_1 y_{1,1} z_{1,1}^2$$

$$\begin{aligned}
& K 4 t x [ ] x_1 y_{1,1,1} z_1 z_{1,1} C 4 t x [ ] x_{1,1} y_1 z_1 z_{1,1} K 30 t x [ ] x_{1,1} y_{1,1} z_1 z_{1,1} \\
& C 4 t x [ ] x_{1,1} y_{1,1} z_1^2 C 6 t x [ ] x_{1,1,1} y_1 z_1 z_{1,1} C 6 t x [ ] x_{1,1,1} y_{1,1} z_1^2 \\
& K 2 t x [ ] x_{1,1,1,1} y_1 z_1^2 K 2 t x_1^2 y_1 z [ ] z_{1,1,1,1} C 6 t x_1^2 y_{1,1} z [ ] z_{1,1,1} C 4 t \\
& x_1^2 y_{1,1,1} z [ ] z_{1,1} C 6 t x_1 x_{1,1} y_1 z [ ] z_{1,1,1} K 30 t x_1 x_{1,1} y_{1,1} z [ ] z_{1,1} \\
& K 4 t x_1 x_{1,1} y_{1,1} z [ ] z_1 C 4 t x_1 x_{1,1,1} y_1 z [ ] z_{1,1} K 6 t x_1 x_{1,1,1} y_{1,1} z [ ] z_1 \\
& C 2 t x_1 x_{1,1,1,1} y_1 z [ ] z_1 C 30 t x_{1,1}^2 y_{1,1} z [ ] z_1 K 10 t x_{1,1} x_{1,1,1} y_1 z [ ] z_1 C x [ ]^2 x_1 \\
& z_1^2 z_{1,1,1,1} K 10 x [ ]^2 x_1 z_1 z_{1,1} z_{1,1,1} C 15 x [ ]^2 x_1 z_1^3 C 4 x [ ]^2 x_{1,1} z_{1,1}^2 z_{1,1,1} \\
& K 15 x [ ]^2 x_{1,1} z_1 z_{1,1}^2 C 6 x [ ]^2 x_{1,1,1} z_{1,1}^2 K x [ ]^2 x_{1,1,1,1} z_1^3 K 2 x [ ] \\
& x_1^2 z [ ] z_1 z_{1,1,1,1} C 10 x [ ] x_1^2 z [ ] z_{1,1} z_{1,1,1} C 2 x [ ] x_1 x_{1,1} z [ ] z_1 z_{1,1,1} \\
& K 30 x [ ] x_1 x_{1,1} z [ ] z_{1,1}^2 K 2 x [ ] x_1 x_{1,1,1} z [ ] z_1 z_{1,1} C 2 x [ ] x_1 x_{1,1,1,1} z [ ] z_1^2 \\
& C 30 x [ ] x_1^2 z [ ] z_1 z_{1,1} K 10 x [ ] x_{1,1} x_{1,1,1} z [ ] z_1^2 C x_1^3 z [ ]^2 z_{1,1,1,1} K 6 \\
& x_1^2 x_{1,1} z [ ]^2 z_{1,1,1} K 4 x_1^2 x_{1,1,1} z [ ]^2 z_{1,1} K x_1^2 x_{1,1,1,1} z [ ]^2 z_1 C 15 x_1 x_1^2 z [ ]^2 z_{1,1} \\
& C 10 x_1 x_{1,1} x_{1,1,1} z [ ]^2 z_1 K 15 x_1^3 z [ ]^2 z_1 C t^2 y_1^2 y_{1,1,1,1} K 10 t^2 y_1 y_{1,1} y_{1,1,1} \\
& C 15 t^2 y_1^3 K 4 t x [ ] y_1 y_{1,1} z_{1,1} K 6 t x [ ] y_1 y_{1,1,1} z_{1,1} C 2 t x [ ] y_1 y_{1,1,1,1} z_1 \\
& C 30 t x [ ] y_1^2 z_{1,1} K 10 t x [ ] y_{1,1} y_{1,1,1} z_1 K 2 t x_1 y [ ] y_1 z_{1,1,1,1} \\
& C 6 t x_1 y [ ] y_{1,1} z_{1,1,1} C 4 t x_1 y [ ] y_{1,1,1} z_{1,1} K 2 t x_1 y_1 y_{1,1,1,1} z [ ] \\
& C 10 t x_1 y_{1,1} y_{1,1,1} z [ ] K 4 t x_{1,1} y [ ] y_{1,1,1} z_1 C 6 t x_{1,1} y_1 y_{1,1,1} z [ ] K 30 t x_{1,1} \\
& y_1^2 z [ ] K 6 t x_{1,1,1} y [ ] y_{1,1} z_1 C 4 t x_{1,1,1} y_1 y_{1,1} z [ ] C 2 t x_{1,1,1,1} y [ ] y_1 z_1 \\
& K 4 x [ ]^2 y_{1,1} z_1 z_{1,1,1} C 15 x [ ]^2 y_{1,1} z_{1,1}^2 K 6 x [ ]^2 y_{1,1,1} z_1 z_{1,1} C x [ ]^2 y_{1,1,1,1} z_1^2 \\
& K 2 x [ ] x_1 y [ ] z_1 z_{1,1,1,1} C 10 x [ ] x_1 y [ ] z_{1,1} z_{1,1,1} C 4 x [ ] x_1 y_{1,1} z [ ] z_{1,1,1} \\
& C 6 x [ ] x_1 y_{1,1,1} z [ ] z_{1,1} K 2 x [ ] x_1 y_{1,1,1,1} z [ ] z_1 K 4 x [ ] x_{1,1} y [ ] z_1 z_{1,1,1} \\
& K 30 x [ ] x_{1,1} y_{1,1} z [ ] z_{1,1} C 6 x [ ] x_{1,1} y_{1,1,1} z [ ] z_1 K 6 x [ ] x_{1,1,1} y [ ] z_1 z_{1,1} \\
& C 4 x [ ] x_{1,1,1} y_{1,1} z [ ] z_1 C 2 x [ ] x_{1,1,1,1} y [ ] z_1^2 C 2 x_1^2 y [ ] z [ ] z_{1,1,1,1} C \\
& x_1^2 y_{1,1,1,1} z [ ]^2 K 6 x_1 x_{1,1} y [ ] z [ ] z_{1,1,1} K 6 x_1 x_{1,1} y_{1,1,1} z [ ]^2 \\
& K 4 x_1 x_{1,1,1} y [ ] z [ ] z_{1,1} K 4 x_1 x_{1,1,1} y_{1,1} z [ ]^2 K 2 x_1 x_{1,1,1,1} y [ ] z [ ] z_1 C 15 \\
& x_1^2 y_{1,1} z [ ]^2 C 10 x_{1,1} x_{1,1,1} y [ ] z [ ] z_1 K 2 t y [ ] y_1 y_{1,1,1,1} C 10 t y [ ] y_{1,1} y_{1,1,1} \\
& C 4 x [ ] y [ ] y_{1,1} z_{1,1,1} C 6 x [ ] y [ ] y_{1,1,1} z_{1,1} K 2 x [ ] y [ ] y_{1,1,1,1} z_1 \\
& C x_1 y [ ]^2 z_{1,1,1,1} C 2 x_1 y [ ] y_{1,1,1,1} z [ ] K 6 x_{1,1} y [ ] y_{1,1,1} z [ ] \\
& K 4 x_{1,1,1} y [ ] y_{1,1} z [ ] K x_{1,1,1,1} y [ ]^2 z_1 C y [ ]^2 y_{1,1,1,1} )
\end{aligned}$$

**M** >  $I_{4b} \text{ d Hook}([v2, v4], \omega)$

$$I_{4b} \text{ d k } \frac{1}{(t y_1 C x [ ] z_1 K x_1 z [ ] K y [ ])^8} (t^2 x_1 y_1 y_{1,1} z_{1,1,1,1} K t^2 x_1 y_1 y_{1,1,1,1} z_{1,1}$$

**(1.10)**

$$\begin{aligned}
& K 6 t^2 x_1 y_1^2 z_1 z_1 z_1 z_1 C 6 t^2 x_1 y_1 y_1 y_1 z_1 z_1 K t^2 x_1 y_1^2 z_1 z_1 z_1 z_1 \\
& C 6 t^2 x_1 y_1 y_1 z_1 z_1 C t^2 x_1 y_1 y_1 z_1 z_1 K 6 t^2 x_1 y_1 y_1 z_1 z_1 \\
& K 6 t^2 x_1 y_1 y_1 z_1 z_1 C 6 t^2 x_1 y_1^2 z_1 z_1 C t^2 x_1 y_1^2 z_1 z_1 K t^2 x_1 y_1 y_1 z_1 z_1 \\
& C t x [ ] x_1 y_1 z_1 z_1 z_1 z_1 K 6 t x [ ] x_1 y_1 z_1 z_1 z_1 z_1 C 6 t x [ ] x_1 y_1 z_1^2 z_1 z_1 \\
& K t x [ ] x_1 y_1 z_1 z_1 z_1 z_1 K t x [ ] x_1 y_1 z_1 z_1 z_1 z_1 C 6 t x [ ] x_1 y_1 z_1 z_1 z_1 z_1 \\
& K 6 t x [ ] x_1 y_1 z_1 z_1 z_1 C t x [ ] x_1 y_1 z_1 z_1 z_1 K 6 t x [ ] x_1 y_1 z_1^2 z_1 z_1 \\
& C 6 t x [ ] x_1 y_1 z_1 z_1 z_1 C t x [ ] x_1 y_1 z_1 z_1 z_1 K t x [ ] x_1 y_1 z_1^2 z_1 z_1 K t \\
& x_1^2 y_1 z [ ] z_1 z_1 z_1 z_1 C t x_1^2 y_1 z [ ] z_1 z_1 C t x_1 x_1 y_1 z [ ] z_1 z_1 z_1 z_1 \\
& C 6 t x_1 x_1 y_1 z [ ] z_1 z_1 z_1 K 6 t x_1 x_1 y_1 z [ ] z_1 z_1 K t x_1 x_1 y_1 z [ ] z_1 z_1 z_1 z_1 \\
& K t x_1 x_1 y_1 z [ ] z_1 z_1 C t x_1 x_1 y_1 z [ ] z_1 z_1 K 6 t x_1^2 y_1 z [ ] z_1 z_1 z_1 C 6 t \\
& x_1^2 y_1 z [ ] z_1 z_1 C 6 t x_1 x_1 y_1 z [ ] z_1 z_1 K 6 t x_1 x_1 y_1 z [ ] z_1 z_1 \\
& K t x [ ] y_1 y_1 z_1 z_1 z_1 C t x [ ] y_1 y_1 z_1 z_1 z_1 C 6 t x [ ] y_1^2 z_1 z_1 z_1 \\
& K 6 t x [ ] y_1 y_1 z_1 z_1 z_1 K t x_1 y [ ] y_1 z_1 z_1 z_1 C t x_1 y [ ] y_1 z_1 z_1 z_1 \\
& C 2 t x_1 y [ ] y_1 z_1 z_1 z_1 z_1 K 6 t x_1 y [ ] y_1 z_1 z_1 z_1 K t x_1 y [ ] y_1 z_1 z_1 z_1 \\
& K t x_1 y_1 y_1 z_1 z_1 z_1 C 6 t x_1 y_1 y_1 z_1 z_1 z_1 C 6 t x_1 y_1 z_1 z_1 z_1 K 6 t x_1 y_1 z_1 z_1 z_1 \\
& y_1^2 z [ ] K 2 t x_1 y_1 z_1 z_1 z_1 C t x_1 y_1 z_1 z_1 z_1 C t x_1 y_1 y_1 z_1 z_1 z_1 \\
& K x [ ]^2 y_1 z_1 z_1 z_1 z_1 C 6 x [ ]^2 y_1 z_1 z_1 z_1 z_1 K 6 x [ ]^2 y_1 z_1 z_1 z_1 z_1 \\
& C x [ ]^2 y_1 z_1 z_1 z_1 z_1 C x [ ] x_1 y_1 z [ ] z_1 z_1 z_1 z_1 K x [ ] x_1 y_1 z [ ] z_1 z_1 z_1 z_1 \\
& C x [ ] x_1 y [ ] z_1 z_1 z_1 z_1 z_1 K 6 x [ ] x_1 y [ ] z_1 z_1 z_1 z_1 z_1 K 6 x [ ] x_1 y_1 z [ ] z_1 z_1 z_1 z_1 \\
& C 12 x [ ] x_1 y_1 z [ ] z_1 z_1 z_1 z_1 z_1 K x [ ] x_1 y_1 z [ ] z_1 z_1 z_1 z_1 z_1 C 6 x [ ] x_1 y [ ] z_1^2 z_1 z_1 z_1 \\
& K 6 x [ ] x_1 y_1 z [ ] z_1 z_1 z_1 z_1 z_1 K x [ ] x_1 y_1 z [ ] z_1 z_1 z_1 z_1 C x [ ] x_1 y_1 z [ ] z_1 z_1 z_1 z_1 \\
& K x_1 x_1 y [ ] z [ ] z_1 z_1 z_1 z_1 z_1 C x_1 x_1 y_1 z [ ]^2 z_1 z_1 z_1 z_1 C x_1 x_1 y_1 z [ ] z_1 z_1 z_1 z_1 \\
& K x_1 x_1 y_1 z [ ]^2 C 6 x_1^2 y [ ] z [ ] z_1 z_1 z_1 z_1 z_1 K 6 x_1^2 y_1 z [ ]^2 z_1 z_1 z_1 z_1 z_1 \\
& K 6 x_1 x_1 y_1 z [ ] z [ ] z_1 z_1 z_1 z_1 z_1 C 6 x_1 x_1 y_1 z [ ]^2 C x [ ] y [ ] y_1 z_1 z_1 z_1 z_1 \\
& K x [ ] y [ ] y_1 z_1 z_1 z_1 z_1 K x_1 y [ ]^2 z_1 z_1 z_1 z_1 z_1 C x_1 y [ ] y_1 z_1 z_1 z_1 z_1 \\
& C x_1 y [ ]^2 z_1 z_1 z_1 z_1 z_1 K x_1 y [ ] y_1 z [ ] z_1 z_1 z_1 z_1 z_1
\end{aligned}$$

**M** >  $I_{4c} \text{d Hook}([v3, v4], \omega)$

$$I_{4c} \text{d} K \frac{1}{(t y_1 C x [ ] z_1 K x_1 z [ ] K y [ ])^{10}} (t^3 x_1 y_1^2 y_1 z_1 z_1 z_1 z_1 z_1 K t^3 x_1 y_1^2 y_1 z_1 z_1 z_1 z_1 z_1) \quad (1.11)$$

$$\begin{aligned}
& K 3 t^3 x_1 y_1 y_1^2 z_1 z_1 z_1 z_1 z_1 C 4 t^3 x_1 y_1 y_1 y_1 z_1 z_1 z_1 z_1 C 3 t^3 x_1 y_1 y_1 y_1 z_1 z_1 z_1 z_1 \\
& K 4 t^3 x_1 y_1 y_1^2 z_1 z_1 z_1 z_1 C 3 t^3 x_1 y_1^3 z_1 z_1 z_1 z_1 K 3 t^3 x_1 y_1^2 y_1 z_1 z_1 z_1 z_1 C 3 t^3 x_1 y_1^2 y_1 z_1 z_1 z_1 z_1 z_1 \\
& K 4 t^3 x_1 y_1^2 y_1 z_1 z_1 z_1 z_1 z_1 K 3 t^3 x_1 y_1 y_1^2 z_1 z_1 z_1 z_1 z_1
\end{aligned}$$

$K 3 t^3 x_{1,1} y_1 y_{1,1} y_{1,1,1,1} z_1 C 4 t^3 x_{1,1} y_1 y_{1,1,1,1}^2 z_1 C 3 t^3 x_{1,1} y_{1,1}^2 y_{1,1,1,1} z_1 K t^3 x_{1,1,1,1}$   
 $y_1^3 z_{1,1,1,1} C 4 t^3 x_{1,1,1,1} y_1^2 y_{1,1,1,1} z_1 C t^3 x_{1,1,1,1} y_1^2 y_{1,1,1,1} z_1 C 3 t^3 x_{1,1,1,1} y_1 y_1^2 z_1$   
 $K 4 t^3 x_{1,1,1,1} y_1 y_{1,1} y_{1,1,1,1} z_1 K 3 t^3 x_{1,1,1,1} y_1^3 z_1 C t^3 x_{1,1,1,1} y_1^3 z_{1,1,1} K 3 t^3 x_{1,1,1,1}$   
 $y_1^2 y_{1,1} z_{1,1} K t^3 x_{1,1,1,1} y_1^2 y_{1,1,1,1} z_1 C 3 t^3 x_{1,1,1,1} y_1 y_1^2 z_1$   
 $K 3 t^2 x[ ] x_1 y_1 y_{1,1} z_{1,1} z_{1,1,1,1} C 4 t^2 x[ ] x_1 y_1 y_{1,1} z_{1,1,1,1}^2$   
 $C 2 t^2 x[ ] x_1 y_1 y_{1,1,1} z_1 z_{1,1,1,1} K 4 t^2 x[ ] x_1 y_1 y_{1,1,1} z_{1,1} z_{1,1,1}$   
 $K 2 t^2 x[ ] x_1 y_1 y_{1,1,1,1} z_1 z_{1,1,1} C 3 t^2 x[ ] x_1 y_1 y_{1,1,1,1} z_{1,1}^2 K 3 t^2 x[ ] x_1$   
 $y_{1,1}^2 z_1 z_{1,1,1,1} C 6 t^2 x[ ] x_1 y_1^2 z_{1,1} z_{1,1,1,1} C 4 t^2 x[ ] x_1 y_{1,1} y_{1,1,1} z_1 z_{1,1,1}$   
 $K 6 t^2 x[ ] x_1 y_{1,1} y_{1,1,1,1} z_{1,1}^2 C 3 t^2 x[ ] x_1 y_{1,1} y_{1,1,1,1} z_1 z_{1,1} K 4 t^2 x[ ] x_1$   
 $y_{1,1,1}^2 z_1 z_{1,1} C 3 t^2 x[ ] x_{1,1} y_1^2 z_{1,1} z_{1,1,1,1} K 4 t^2 x[ ] x_{1,1} y_1^2 z_{1,1,1}^2$   
 $C 3 t^2 x[ ] x_{1,1} y_1 y_{1,1} z_1 z_{1,1,1,1} K 6 t^2 x[ ] x_{1,1} y_1 y_{1,1} z_{1,1} z_{1,1,1}$   
 $K 3 t^2 x[ ] x_{1,1} y_1 y_{1,1,1,1} z_1 z_{1,1} C 6 t^2 x[ ] x_{1,1} y_{1,1} y_{1,1,1} z_1 z_{1,1}$   
 $K 3 t^2 x[ ] x_{1,1} y_{1,1} y_{1,1,1,1} z_1^2 C 4 t^2 x[ ] x_{1,1} y_{1,1,1}^2 z_1^2 K 2 t^2 x[ ] x_{1,1,1} y_1^2 z_1 z_{1,1,1,1}$   
 $C 4 t^2 x[ ] x_{1,1,1} y_1^2 z_{1,1} z_{1,1,1} K 4 t^2 x[ ] x_{1,1,1} y_1 y_{1,1} z_1 z_{1,1,1}$   
 $C 6 t^2 x[ ] x_{1,1,1} y_1 y_{1,1} z_{1,1}^2 C 4 t^2 x[ ] x_{1,1,1} y_1 y_{1,1,1} z_1 z_{1,1}$   
 $C 2 t^2 x[ ] x_{1,1,1} y_1 y_{1,1,1,1} z_1^2 K 6 t^2 x[ ] x_{1,1,1} y_1^2 z_1 z_{1,1}$   
 $K 4 t^2 x[ ] x_{1,1,1} y_{1,1} y_{1,1,1} z_1^2 C 2 t^2 x[ ] x_{1,1,1,1} y_1^2 z_1 z_{1,1,1} K 3 t^2 x[ ] x_{1,1,1,1} y_1^2 z_{1,1}^2$   
 $K 2 t^2 x[ ] x_{1,1,1,1} y_1 y_{1,1,1} z_1^2 C 3 t^2 x[ ] x_{1,1,1,1} y_1^2 z_1^2 K 2 t^2 x_1^2 y_1 y_{1,1,1} z[ ] z_{1,1,1,1}$   
 $C 2 t^2 x_1^2 y_1 y_{1,1,1,1} z[ ] z_{1,1,1} C 3 t^2 x_1^2 y_1^2 z[ ] z_{1,1,1,1} K 4 t^2 x_1^2 y_{1,1} y_{1,1,1} z[ ] z_{1,1,1}$   
 $K 3 t^2 x_1^2 y_{1,1} y_{1,1,1,1} z[ ] z_{1,1} C 4 t^2 x_1^2 y_{1,1,1}^2 z[ ] z_{1,1} C 4 t^2 x_1 x_{1,1} y_1 y_{1,1,1} z[ ] z_{1,1,1}$   
 $K 3 t^2 x_1 x_{1,1} y_1 y_{1,1,1,1} z[ ] z_{1,1} K 6 t^2 x_1 x_{1,1} y_1^2 z[ ] z_{1,1,1}$   
 $C 6 t^2 x_1 x_{1,1} y_{1,1} y_{1,1,1} z[ ] z_{1,1} C 3 t^2 x_1 x_{1,1} y_{1,1} y_{1,1,1,1} z[ ] z_1 K 4 t^2 x_1 x_{1,1}$   
 $y_{1,1,1}^2 z[ ] z_1 C 2 t^2 x_1 x_{1,1,1} y_1^2 z[ ] z_{1,1,1,1} K 4 t^2 x_1 x_{1,1,1} y_1 y_{1,1} z[ ] z_{1,1,1}$   
 $K 2 t^2 x_1 x_{1,1,1} y_1 y_{1,1,1,1} z[ ] z_1 C 4 t^2 x_1 x_{1,1,1} y_{1,1} y_{1,1,1} z[ ] z_1 K 2 t^2 x_1 x_{1,1,1,1}$   
 $y_1^2 z[ ] z_{1,1,1} C 3 t^2 x_1 x_{1,1,1,1} y_1 y_{1,1} z[ ] z_{1,1} C 2 t^2 x_1 x_{1,1,1,1} y_1 y_{1,1,1} z[ ] z_1$   
 $K 3 t^2 x_1 x_{1,1,1,1} y_1^2 z[ ] z_1 K 3 t^2 x_{1,1}^2 y_1^2 z[ ] z_{1,1,1,1} C 6 t^2 x_{1,1}^2 y_1 y_{1,1} z[ ] z_{1,1,1}$   
 $C 3 t^2 x_{1,1}^2 y_1 y_{1,1,1,1} z[ ] z_1 K 6 t^2 x_{1,1}^2 y_{1,1} y_{1,1,1} z[ ] z_1 C 4 t^2 x_{1,1} x_{1,1,1} y_1^2 z[ ] z_{1,1,1}$   
 $K 6 t^2 x_{1,1} x_{1,1,1} y_1 y_{1,1} z[ ] z_{1,1} K 4 t^2 x_{1,1} x_{1,1,1} y_1 y_{1,1,1} z[ ] z_1 C 6 t^2 x_{1,1} x_{1,1,1}$   
 $y_{1,1}^2 z[ ] z_1 C 3 t^2 x_{1,1} x_{1,1,1,1} y_1^2 z[ ] z_{1,1} K 3 t^2 x_{1,1} x_{1,1,1,1} y_1 y_{1,1} z[ ] z_1 K 4 t^2 x_{1,1,1}^2$   
 $y_1^2 z[ ] z_{1,1} C 4 t^2 x_{1,1,1}^2 y_1 y_{1,1} z[ ] z_1 K 3 t x[ ]^2 x_1 y_{1,1} z_1 z_{1,1} z_{1,1,1,1}$   
 $C 4 t x[ ]^2 x_1 y_{1,1} z_1 z_{1,1,1} C 3 t x[ ]^2 x_1 y_{1,1} z_{1,1} z_{1,1,1} C t x[ ]^2 x_1 y_{1,1,1} z_{1,1,1,1}$   
 $K 4 t x[ ]^2 x_1 y_{1,1,1} z_1 z_{1,1} z_{1,1,1} K 3 t x[ ]^2 x_1 y_{1,1,1} z_{1,1}^3 K t x[ ]^2 x_1 y_{1,1,1,1} z_{1,1}^2 z_{1,1,1}$

$$\begin{aligned}
& C3tx[ ]^2 x_1 y_{1,1,1,1} z_1 z_{1,1}^2 C3tx[ ]^2 x_{1,1} y_1 z_1 z_{1,1} z_{1,1,1,1} K4tx[ ]^2 x_{1,1} y_1 z_1 z_{1,1,1}^2 \\
& K3tx[ ]^2 x_{1,1} y_1 z_{1,1}^2 z_{1,1,1} C4tx[ ]^2 x_{1,1} y_{1,1} z_1 z_{1,1}^2 C3tx[ ]^2 x_{1,1} y_{1,1} z_1 z_{1,1}^2 \\
& K3tx[ ]^2 x_{1,1} y_{1,1,1,1} z_1 z_{1,1}^2 Ktx[ ]^2 x_{1,1} y_1 z_1 z_{1,1,1,1} \\
& C4tx[ ]^2 x_{1,1} y_1 z_1 z_{1,1} z_{1,1,1} C3tx[ ]^2 x_{1,1} y_1 z_1^3 K4tx[ ]^2 x_{1,1} y_{1,1} z_1 z_{1,1}^2 \\
& K3tx[ ]^2 x_{1,1} y_{1,1} z_1 z_{1,1}^2 Ctx[ ]^2 x_{1,1} y_{1,1,1,1} z_1^3 Ctx[ ]^2 x_{1,1,1,1} y_1 z_1 z_{1,1}^2 \\
& K3tx[ ]^2 x_{1,1,1,1} y_1 z_1 z_{1,1}^2 C3tx[ ]^2 x_{1,1,1,1} y_{1,1} z_1 z_{1,1}^2 Ktx[ ]^2 x_{1,1,1,1} y_{1,1} z_1^3 \\
& C3tx[ ] x_1^2 y_{1,1} z[ ] z_{1,1} z_{1,1,1,1} K4tx[ ] x_1^2 y_{1,1} z[ ] z_{1,1,1,1}^2 K2tx[ ] \\
& x_1^2 y_{1,1,1,1} z[ ] z_1 z_{1,1,1,1} C4tx[ ] x_1^2 y_{1,1,1,1} z[ ] z_{1,1} z_{1,1,1,1} C2tx[ ] \\
& x_1^2 y_{1,1,1,1} z[ ] z_1 z_{1,1,1,1} K3tx[ ] x_1^2 y_{1,1,1,1} z[ ] z_{1,1}^2 \\
& K3tx[ ] x_1 x_{1,1} y_1 z[ ] z_{1,1} z_{1,1,1,1} C4tx[ ] x_1 x_{1,1} y_1 z[ ] z_{1,1,1,1}^2 \\
& C3tx[ ] x_1 x_{1,1} y_{1,1} z[ ] z_1 z_{1,1,1,1} K6tx[ ] x_1 x_{1,1} y_{1,1} z[ ] z_{1,1} z_{1,1,1,1} \\
& K4tx[ ] x_1 x_{1,1} y_{1,1} z[ ] z_1 z_{1,1,1,1} C6tx[ ] x_1 x_{1,1} y_{1,1} z[ ] z_{1,1}^2 \\
& C2tx[ ] x_1 x_{1,1,1,1} y_1 z[ ] z_1 z_{1,1,1,1} K4tx[ ] x_1 x_{1,1,1,1} y_1 z[ ] z_{1,1} z_{1,1,1,1} \\
& C4tx[ ] x_1 x_{1,1,1,1} y_{1,1} z[ ] z_1 z_{1,1} K2tx[ ] x_1 x_{1,1,1,1} y_{1,1} z[ ] z_{1,1}^2 \\
& K2tx[ ] x_1 x_{1,1,1,1} y_1 z[ ] z_1 z_{1,1,1,1} C3tx[ ] x_1 x_{1,1,1,1} y_1 z[ ] z_{1,1}^2 \\
& K3tx[ ] x_1 x_{1,1,1,1} y_{1,1} z[ ] z_1 z_{1,1} C2tx[ ] x_1 x_{1,1,1,1} y_{1,1} z[ ] z_{1,1}^2 K3tx[ ] \\
& x_{1,1}^2 y_1 z[ ] z_1 z_{1,1,1,1} C6tx[ ] x_{1,1}^2 y_1 z[ ] z_{1,1} z_{1,1,1,1} K6tx[ ] x_{1,1}^2 y_{1,1,1,1} z[ ] z_1 z_{1,1} \\
& C3tx[ ] x_{1,1}^2 y_{1,1,1,1} z[ ] z_{1,1}^2 C4tx[ ] x_{1,1} x_{1,1,1,1} y_1 z[ ] z_1 z_{1,1,1,1} \\
& K6tx[ ] x_{1,1} x_{1,1,1,1} y_1 z[ ] z_{1,1}^2 C6tx[ ] x_{1,1} x_{1,1,1,1} y_{1,1} z[ ] z_1 z_{1,1} \\
& K4tx[ ] x_{1,1} x_{1,1,1,1} y_{1,1} z[ ] z_{1,1}^2 C3tx[ ] x_{1,1} x_{1,1,1,1} y_1 z[ ] z_1 z_{1,1} \\
& K3tx[ ] x_{1,1} x_{1,1,1,1} y_{1,1} z[ ] z_{1,1}^2 K4tx[ ] x_{1,1}^2 y_1 z[ ] z_1 z_{1,1} C4tx[ ] \\
& x_{1,1,1,1}^2 y_{1,1} z[ ] z_{1,1}^2 Ctx_1^3 y_{1,1,1,1} z[ ]^2 z_{1,1,1,1} Ktx_1^3 y_{1,1,1,1} z[ ]^2 z_{1,1,1,1} K3t \\
& x_1^2 x_{1,1} y_{1,1} z[ ]^2 z_{1,1,1,1} C3tx_1^2 x_{1,1} y_{1,1,1,1} z[ ]^2 z_{1,1} Ktx_1^2 x_{1,1} y_1 z[ ]^2 z_{1,1,1,1} \\
& C4tx_1^2 x_{1,1,1,1} y_{1,1} z[ ]^2 z_{1,1,1,1} K4tx_1^2 x_{1,1,1,1} y_{1,1} z[ ]^2 z_{1,1} Ct \\
& x_1^2 x_{1,1,1,1} y_{1,1,1,1} z[ ]^2 z_1 Ctx_1^2 x_{1,1,1,1} y_1 z[ ]^2 z_{1,1,1,1} Ktx_1^2 x_{1,1,1,1} y_{1,1} z[ ]^2 z_1 \\
& C3tx_1 x_{1,1}^2 y_1 z[ ]^2 z_{1,1,1,1} C3tx_1 x_{1,1}^2 y_{1,1} z[ ]^2 z_{1,1,1,1} K3tx_1 x_{1,1}^2 y_{1,1} z[ ]^2 z_{1,1} \\
& K3tx_1 x_{1,1}^2 y_{1,1,1,1} z[ ]^2 z_1 K4tx_1 x_{1,1} x_{1,1,1,1} y_1 z[ ]^2 z_{1,1,1,1} \\
& C4tx_1 x_{1,1} x_{1,1,1,1} y_{1,1} z[ ]^2 z_1 K3tx_1 x_{1,1} x_{1,1,1,1} y_1 z[ ]^2 z_{1,1} \\
& C3tx_1 x_{1,1} x_{1,1,1,1} y_{1,1} z[ ]^2 z_1 C4tx_1 x_{1,1}^2 y_1 z[ ]^2 z_{1,1} K4tx_1 x_{1,1}^2 y_{1,1} z[ ]^2 z_1 \\
& K3tx_1^3 y_1 z[ ]^2 z_{1,1,1,1} C3tx_1^3 y_{1,1,1,1} z[ ]^2 z_1 C3tx_1^2 x_{1,1} y_1 z[ ]^2 z_{1,1} K3t \\
& x_{1,1}^2 x_{1,1,1,1} y_{1,1} z[ ]^2 z_1 K^2 x[ ] y_1^2 y_{1,1,1,1} z_{1,1,1,1} C^2 x[ ] y_1^2 y_{1,1,1,1} z_{1,1,1,1} \\
& C3^2 x[ ] y_1 y_{1,1}^2 z_{1,1,1,1} K4^2 x[ ] y_1 y_{1,1} y_{1,1,1,1} z_{1,1,1,1} K3^2 x[ ] y_1 y_{1,1} y_{1,1,1,1} z_{1,1}
\end{aligned}$$

$$\begin{aligned}
& C4 \ell^2 x[ ] y_1 y_{1,1}^2 z_{1,1} K3 \ell^2 x[ ] y_{1,1}^3 z_{1,1} C3 \ell^2 x[ ] y_{1,1}^2 y_{1,1} z_{1,1} \\
& K2 \ell^2 x_1 y[ ] y_1 y_{1,1} z_{1,1} C2 \ell^2 x_1 y[ ] y_1 y_{1,1} z_{1,1} C3 \ell^2 x_1 y[ ] y_{1,1}^2 z_{1,1} \\
& K4 \ell^2 x_1 y[ ] y_{1,1} y_{1,1} z_{1,1} K3 \ell^2 x_1 y[ ] y_{1,1} y_{1,1} z_{1,1} C4 \ell^2 x_1 y[ ] y_{1,1}^2 z_{1,1} \\
& K6 \ell^2 x_{1,1} y[ ] y_1 y_{1,1} z_{1,1} C8 \ell^2 x_{1,1} y[ ] y_1 y_{1,1} z_{1,1} C3 \ell^2 x_{1,1} y[ ] y_{1,1}^2 z_{1,1} \\
& C3 \ell^2 x_{1,1} y[ ] y_{1,1} y_{1,1} z_{1,1} K4 \ell^2 x_{1,1} y[ ] y_{1,1}^2 z_{1,1} C3 \ell^2 x_{1,1} y_1 y_{1,1} y_{1,1} z[ ] \\
& K4 \ell^2 x_{1,1} y_1 y_{1,1}^2 z[ ] K3 \ell^2 x_{1,1} y_{1,1}^2 y_{1,1} z[ ] C3 \ell^2 x_{1,1} y[ ] y_{1,1}^2 z_{1,1} \\
& K8 \ell^2 x_{1,1,1} y[ ] y_1 y_{1,1} z_{1,1} K2 \ell^2 x_{1,1,1} y[ ] y_1 y_{1,1} z_{1,1} K3 \ell^2 x_{1,1,1} y[ ] y_{1,1}^2 z_{1,1} \\
& C4 \ell^2 x_{1,1,1} y[ ] y_{1,1} y_{1,1} z_{1,1} K \ell^2 x_{1,1,1} y_{1,1}^2 y_{1,1} z[ ] C4 \ell^2 x_{1,1,1} y_1 y_{1,1} y_{1,1} z[ ] \\
& C3 \ell^2 x_{1,1,1} y_{1,1}^3 z[ ] K3 \ell^2 x_{1,1,1,1} y[ ] y_{1,1}^2 z_{1,1} C6 \ell^2 x_{1,1,1,1} y[ ] y_1 y_{1,1} z_{1,1} \\
& C2 \ell^2 x_{1,1,1,1} y[ ] y_1 y_{1,1} z_{1,1} K3 \ell^2 x_{1,1,1,1} y[ ] y_{1,1}^2 z_{1,1} C \ell^2 x_{1,1,1,1} y_{1,1}^2 y_{1,1} z[ ] \\
& K3 \ell^2 x_{1,1,1,1} y_1 y_{1,1}^2 z[ ] C3 tx[ ] y_1 y_{1,1} z_{1,1} z_{1,1,1} K4 tx[ ] y_1 y_{1,1} z_{1,1}^2 \\
& K2 tx[ ] y_1 y_{1,1} z_{1,1} z_{1,1,1} C4 tx[ ] y_1 y_{1,1} z_{1,1} z_{1,1,1} \\
& C2 tx[ ] y_1 y_{1,1,1} z_{1,1} z_{1,1,1} K3 tx[ ] y_1 y_{1,1,1} z_{1,1}^2 C3 tx[ ] y_{1,1}^2 z_{1,1} z_{1,1,1} \\
& K6 tx[ ] y_{1,1}^2 z_{1,1} z_{1,1,1} K4 tx[ ] y_{1,1} y_{1,1} z_{1,1} z_{1,1,1} C6 tx[ ] y_{1,1} y_{1,1} z_{1,1}^2 \\
& K3 tx[ ] y_{1,1} y_{1,1,1} z_{1,1} z_{1,1} C4 tx[ ] y_{1,1}^2 z_{1,1} z_{1,1} \\
& C3 tx[ ] x_1 y[ ] y_{1,1} z_{1,1} z_{1,1,1} K4 tx[ ] x_1 y[ ] y_{1,1} z_{1,1}^2 \\
& K2 tx[ ] x_1 y[ ] y_{1,1,1} z_{1,1} z_{1,1,1} C4 tx[ ] x_1 y[ ] y_{1,1,1} z_{1,1} z_{1,1,1} \\
& C2 tx[ ] x_1 y[ ] y_{1,1,1,1} z_{1,1} z_{1,1} K3 tx[ ] x_1 y[ ] y_{1,1,1,1} z_{1,1}^2 \\
& C2 tx[ ] x_1 y_1 y_{1,1} z[ ] z_{1,1,1} K2 tx[ ] x_1 y_1 y_{1,1,1} z[ ] z_{1,1,1} K3 tx[ ] x_1 \\
& y_{1,1}^2 z[ ] z_{1,1,1,1} C4 tx[ ] x_1 y_{1,1} y_{1,1} z[ ] z_{1,1,1} C3 tx[ ] x_1 y_{1,1} y_{1,1,1} z[ ] z_{1,1} \\
& K4 tx[ ] x_1 y_{1,1}^2 z[ ] z_{1,1} K6 tx[ ] x_{1,1} y[ ] y_1 z_{1,1} z_{1,1,1} C8 tx[ ] x_{1,1} y[ ] y_1 \\
& z_{1,1,1}^2 K3 tx[ ] x_{1,1} y[ ] y_{1,1} z_{1,1} z_{1,1,1} C6 tx[ ] x_{1,1} y[ ] y_{1,1} z_{1,1} z_{1,1,1} \\
& C3 tx[ ] x_{1,1} y[ ] y_{1,1,1,1} z_{1,1} z_{1,1} K3 tx[ ] x_{1,1} y_1 y_{1,1} z[ ] z_{1,1,1,1} \\
& K4 tx[ ] x_{1,1} y_1 y_{1,1} z[ ] z_{1,1,1} C6 tx[ ] x_{1,1} y_1 y_{1,1,1} z[ ] z_{1,1} C6 tx[ ] x_{1,1} \\
& y_{1,1}^2 z[ ] z_{1,1,1} K12 tx[ ] x_{1,1} y_{1,1} y_{1,1} z[ ] z_{1,1} C3 tx[ ] x_{1,1} y_{1,1} y_{1,1,1} z[ ] z_{1,1} \\
& K4 tx[ ] x_{1,1} y_{1,1}^2 z[ ] z_{1,1} C4 tx[ ] x_{1,1,1} y[ ] y_1 z_{1,1} z_{1,1,1} \\
& K8 tx[ ] x_{1,1,1} y[ ] y_1 z_{1,1} z_{1,1,1} C4 tx[ ] x_{1,1,1} y[ ] y_{1,1} z_{1,1} z_{1,1,1} \\
& K6 tx[ ] x_{1,1,1} y[ ] y_{1,1} z_{1,1}^2 K4 tx[ ] x_{1,1,1} y[ ] y_{1,1,1} z_{1,1} z_{1,1} \\
& K2 tx[ ] x_{1,1,1} y[ ] y_{1,1,1,1} z_{1,1}^2 C8 tx[ ] x_{1,1,1} y_1 y_{1,1} z[ ] z_{1,1,1} \\
& K4 tx[ ] x_{1,1,1} y_1 y_{1,1} z[ ] z_{1,1} K2 tx[ ] x_{1,1,1} y_1 y_{1,1,1} z[ ] z_{1,1} C6 tx[ ] x_{1,1,1} \\
& y_{1,1}^2 z[ ] z_{1,1} C4 tx[ ] x_{1,1,1} y_{1,1} y_{1,1} z[ ] z_{1,1} K4 tx[ ] x_{1,1,1,1} y[ ] y_1 z_{1,1} z_{1,1,1} \\
& C6 tx[ ] x_{1,1,1,1} y[ ] y_1 z_{1,1}^2 C2 tx[ ] x_{1,1,1,1} y[ ] y_{1,1,1} z_{1,1}^2
\end{aligned}$$

$$\begin{aligned}
& K 3 t x [ ] x_{1,1,1,1} y_1 y_{1,1} z [ ] z_{1,1} C 2 t x [ ] x_{1,1,1,1} y_1 y_{1,1} z [ ] z_{1,1} K 3 t x [ ] x_{1,1,1,1} \\
& y_{1,1}^2 z [ ] z_{1,1} C 2 t x_{1,1}^2 y [ ] y_{1,1,1} z [ ] z_{1,1,1,1} K 2 t x_{1,1}^2 y [ ] y_{1,1,1,1} z [ ] z_{1,1,1} \\
& K 4 t x_1 x_{1,1} y [ ] y_{1,1,1} z [ ] z_{1,1,1} C 3 t x_1 x_{1,1} y [ ] y_{1,1,1,1} z [ ] z_{1,1} \\
& K 3 t x_1 x_{1,1} y_{1,1} y_{1,1,1,1} z [ ]^2 C 4 t x_1 x_{1,1} y_{1,1}^2 z [ ]^2 \\
& K 4 t x_1 x_{1,1,1} y [ ] y_{1,1} z [ ] z_{1,1,1,1} C 4 t x_1 x_{1,1,1} y [ ] y_{1,1} z [ ] z_{1,1,1} \\
& C 2 t x_1 x_{1,1,1} y [ ] y_{1,1,1,1} z [ ] z_{1,1} C 2 t x_1 x_{1,1,1} y_1 y_{1,1,1,1} z [ ]^2 \\
& K 4 t x_1 x_{1,1,1} y_{1,1} y_{1,1,1} z [ ]^2 C 4 t x_1 x_{1,1,1,1} y [ ] y_{1,1} z [ ] z_{1,1,1} \\
& K 3 t x_1 x_{1,1,1,1} y [ ] y_{1,1} z [ ] z_{1,1} K 2 t x_1 x_{1,1,1,1} y [ ] y_{1,1,1} z [ ] z_{1,1} \\
& K 2 t x_1 x_{1,1,1,1} y_1 y_{1,1,1} z [ ]^2 C 3 t x_1 x_{1,1,1,1} y_{1,1}^2 z [ ]^2 C 6 t x_{1,1}^2 y [ ] y_{1,1} z [ ] z_{1,1,1,1} \\
& K 6 t x_{1,1}^2 y [ ] y_{1,1} z [ ] z_{1,1,1} K 3 t x_{1,1}^2 y [ ] y_{1,1,1,1} z [ ] z_{1,1} K 3 t x_{1,1}^2 y_1 y_{1,1,1,1} z [ ]^2 \\
& C 6 t x_{1,1}^2 y_{1,1} y_{1,1,1} z [ ]^2 K 8 t x_{1,1} x_{1,1,1} y [ ] y_{1,1} z [ ] z_{1,1,1} \\
& C 6 t x_{1,1} x_{1,1,1} y [ ] y_{1,1} z [ ] z_{1,1} C 4 t x_{1,1} x_{1,1,1} y [ ] y_{1,1,1} z [ ] z_{1,1} \\
& C 4 t x_{1,1} x_{1,1,1} y_1 y_{1,1,1} z [ ]^2 K 6 t x_{1,1} x_{1,1,1} y_{1,1}^2 z [ ]^2 \\
& K 6 t x_{1,1} x_{1,1,1,1} y [ ] y_{1,1} z [ ] z_{1,1} C 3 t x_{1,1} x_{1,1,1,1} y [ ] y_{1,1} z [ ] z_{1,1} \\
& C 3 t x_{1,1} x_{1,1,1,1} y_1 y_{1,1} z [ ]^2 C 8 t x_{1,1,1,1}^2 y [ ] y_{1,1} z [ ] z_{1,1} K 4 t x_{1,1,1,1}^2 y [ ] y_{1,1} z [ ] z_{1,1} \\
& K 4 t x_{1,1,1,1}^2 y_1 y_{1,1} z [ ]^2 C 3 x [ ]^3 y_{1,1} z_{1,1} z_{1,1,1,1} K 4 x [ ]^3 y_{1,1} z_{1,1} z_{1,1,1}^2 \\
& K 3 x [ ]^3 y_{1,1} z_{1,1}^2 z_{1,1,1} K x [ ]^3 y_{1,1,1} z_{1,1,1,1}^2 C 4 x [ ]^3 y_{1,1,1} z_{1,1} z_{1,1,1} \\
& C 3 x [ ]^3 y_{1,1,1} z_{1,1}^3 C x [ ]^3 y_{1,1,1,1} z_{1,1,1}^2 K 3 x [ ]^3 y_{1,1,1,1} z_{1,1} z_{1,1}^2 \\
& K 3 x [ ]^2 x_1 y_{1,1} z [ ] z_{1,1} z_{1,1,1,1} C 4 x [ ]^2 x_1 y_{1,1} z [ ] z_{1,1,1}^2 \\
& C 2 x [ ]^2 x_1 y_{1,1,1} z [ ] z_{1,1} z_{1,1,1,1} K 4 x [ ]^2 x_1 y_{1,1,1} z [ ] z_{1,1} z_{1,1,1} \\
& K 2 x [ ]^2 x_1 y_{1,1,1,1} z [ ] z_{1,1} z_{1,1,1} C 3 x [ ]^2 x_1 y_{1,1,1,1} z [ ] z_{1,1}^2 \\
& K 3 x [ ]^2 x_{1,1} y [ ] z_{1,1} z_{1,1,1,1} C 4 x [ ]^2 x_{1,1} y [ ] z_{1,1} z_{1,1,1}^2 C 3 x [ ]^2 x_{1,1} y [ ] \\
& z_{1,1} z_{1,1,1} K 3 x [ ]^2 x_{1,1} y_{1,1} z [ ] z_{1,1} z_{1,1,1,1} C 6 x [ ]^2 x_{1,1} y_{1,1} z [ ] z_{1,1} z_{1,1,1} \\
& K 4 x [ ]^2 x_{1,1} y_{1,1,1} z [ ] z_{1,1} z_{1,1,1} K 9 x [ ]^2 x_{1,1} y_{1,1,1} z [ ] z_{1,1}^2 \\
& C 6 x [ ]^2 x_{1,1} y_{1,1,1,1} z [ ] z_{1,1} z_{1,1} C x [ ]^2 x_{1,1,1} y [ ] z_{1,1} z_{1,1,1,1} \\
& K 4 x [ ]^2 x_{1,1,1} y [ ] z_{1,1} z_{1,1,1,1} K 3 x [ ]^2 x_{1,1,1} y [ ] z_{1,1}^3 \\
& C 8 x [ ]^2 x_{1,1,1} y_{1,1} z [ ] z_{1,1} z_{1,1,1} C 3 x [ ]^2 x_{1,1,1} y_{1,1} z [ ] z_{1,1}^2 \\
& K 4 x [ ]^2 x_{1,1,1} y_{1,1,1} z [ ] z_{1,1} z_{1,1} K x [ ]^2 x_{1,1,1} y_{1,1,1,1} z [ ] z_{1,1}^2 K x [ ]^2 x_{1,1,1,1} y [ ] \\
& z_{1,1} z_{1,1,1} C 3 x [ ]^2 x_{1,1,1,1} y [ ] z_{1,1} z_{1,1}^2 K 3 x [ ]^2 x_{1,1,1,1} y_{1,1} z [ ] z_{1,1} z_{1,1} \\
& C x [ ]^2 x_{1,1,1,1} y_{1,1,1} z [ ] z_{1,1}^2 K x [ ]^2 x_{1,1,1,1} y_{1,1,1} z [ ] z_{1,1,1,1} C x [ ]^2 x_{1,1,1,1} y_{1,1,1} z [ ] z_{1,1,1,1} \\
& C 3 x [ ] x_1 x_{1,1} y [ ] z [ ] z_{1,1} z_{1,1,1,1} K 4 x [ ] x_1 x_{1,1} y [ ] z [ ] z_{1,1,1,1}^2 \\
& C 3 x [ ] x_1 x_{1,1} y_{1,1} z [ ] z_{1,1,1,1} C 4 x [ ] x_1 x_{1,1} y_{1,1,1} z [ ] z_{1,1,1,1}
\end{aligned}$$

$K 6 x[ ] x_1 x_{1,1} y_{1,1,1,1} z[ ]^2 z_{1,1} K 2 x[ ] x_1 x_{1,1} y[ ] z[ ] z_{1,1} z_{1,1,1,1}$   
 $C 4 x[ ] x_1 x_{1,1} y[ ] z[ ] z_{1,1} z_{1,1,1,1} K 8 x[ ] x_1 x_{1,1} y_{1,1} z[ ]^2 z_{1,1,1}$   
 $C 4 x[ ] x_1 x_{1,1} y_{1,1,1,1} z[ ]^2 z_{1,1} C 2 x[ ] x_1 x_{1,1} y_{1,1,1,1} z[ ]^2 z_{1,1}$   
 $C 2 x[ ] x_1 x_{1,1,1,1} y[ ] z[ ] z_{1,1} z_{1,1,1,1} K 3 x[ ] x_1 x_{1,1,1,1} y[ ] z[ ] z_{1,1}^2$   
 $C 3 x[ ] x_1 x_{1,1,1,1} y_{1,1} z[ ]^2 z_{1,1} K 2 x[ ] x_1 x_{1,1,1,1} y_{1,1} z[ ]^2 z_{1,1} C 3 x[ ]$   
 $x_{1,1}^2 y[ ] z[ ] z_{1,1} z_{1,1,1,1} K 6 x[ ] x_{1,1}^2 y[ ] z[ ] z_{1,1} z_{1,1,1,1} K 3 x[ ] x_{1,1}^2 y_{1,1} z[ ]^2 z_{1,1,1}$   
 $C 9 x[ ] x_{1,1}^2 y_{1,1,1,1} z[ ]^2 z_{1,1} K 3 x[ ] x_{1,1}^2 y_{1,1,1,1} z[ ]^2 z_{1,1}$   
 $K 4 x[ ] x_{1,1} x_{1,1,1,1} y[ ] z[ ] z_{1,1} z_{1,1,1,1} C 6 x[ ] x_{1,1} x_{1,1,1,1} y[ ] z[ ] z_{1,1}^2$   
 $K 6 x[ ] x_{1,1} x_{1,1,1,1} y_{1,1} z[ ]^2 z_{1,1} C 4 x[ ] x_{1,1} x_{1,1,1,1} y_{1,1} z[ ]^2 z_{1,1}$   
 $K 3 x[ ] x_{1,1} x_{1,1,1,1} y[ ] z[ ] z_{1,1} z_{1,1,1,1} C 3 x[ ] x_{1,1} x_{1,1,1,1} y_{1,1} z[ ]^2 z_{1,1} C 4 x[ ]$   
 $x_{1,1,1,1}^2 y[ ] z[ ] z_{1,1} z_{1,1,1,1} K 4 x[ ] x_{1,1,1,1}^2 y_{1,1} z[ ]^2 z_{1,1} C x_{1,1,1,1}^2 y[ ] z[ ]^2 z_{1,1,1,1} K$   
 $x_{1,1,1,1}^2 x_{1,1,1,1} y_{1,1,1,1} z[ ]^3 K x_{1,1,1,1}^2 y[ ] z[ ]^2 z_{1,1,1,1} C x_{1,1,1,1}^2 y_{1,1,1,1} z[ ]^3 K 3 x_{1,1,1,1}$   
 $x_{1,1,1,1}^2 y[ ] z[ ]^2 z_{1,1,1,1,1} C 3 x_{1,1,1,1}^2 y_{1,1,1,1,1} z[ ]^3 C 4 x_{1,1,1,1} x_{1,1,1,1} y[ ] z[ ]^2 z_{1,1,1,1}$   
 $K 4 x_{1,1,1,1} x_{1,1,1,1} y_{1,1,1,1} z[ ]^3 C 3 x_{1,1,1,1} x_{1,1,1,1} y[ ] z[ ]^2 z_{1,1,1,1}$   
 $K 3 x_{1,1,1,1} x_{1,1,1,1} y_{1,1,1,1} z[ ]^3 K 4 x_{1,1,1,1}^2 y[ ] z[ ]^2 z_{1,1,1,1} C 4 x_{1,1,1,1}^2 y_{1,1,1,1} z[ ]^3 C 3$   
 $x_{1,1,1,1}^3 y[ ] z[ ]^2 z_{1,1,1,1} K 3 x_{1,1,1,1}^3 y_{1,1,1,1} z[ ]^3 K 3 x_{1,1,1,1}^2 y[ ] z[ ]^2 z_{1,1,1,1} C 3$   
 $x_{1,1,1,1}^2 x_{1,1,1,1} y_{1,1,1,1} z[ ]^3 C 2 t x[ ] y[ ] y_{1,1,1,1} z_{1,1,1,1} K 2 t x[ ] y[ ] y_{1,1,1,1} z_{1,1,1,1}$   
 $K 3 t x[ ] y[ ] y_{1,1,1,1}^2 z_{1,1,1,1} C 4 t x[ ] y[ ] y_{1,1,1,1} z_{1,1,1,1}$   
 $C 3 t x[ ] y[ ] y_{1,1,1,1} z_{1,1,1,1} K 4 t x[ ] y[ ] y_{1,1,1,1}^2 z_{1,1,1,1} C t x_{1,1,1,1} y[ ]^2 y_{1,1,1,1} z_{1,1,1,1}$   
 $K t x_{1,1,1,1} y[ ]^2 y_{1,1,1,1} z_{1,1,1,1} C 3 t x_{1,1,1,1} y[ ]^2 y_{1,1,1,1} z_{1,1,1,1} K 4 t x_{1,1,1,1} y[ ]^2 y_{1,1,1,1} z_{1,1,1,1}$   
 $K 3 t x_{1,1,1,1} y[ ] y_{1,1,1,1} z_{1,1,1,1} z[ ] C 4 t x_{1,1,1,1} y[ ] y_{1,1,1,1}^2 z[ ] K 3 t x_{1,1,1,1} y[ ]^2 y_{1,1,1,1,1}$   
 $C 4 t x_{1,1,1,1} y[ ]^2 y_{1,1,1,1} z_{1,1,1,1} C t x_{1,1,1,1} y[ ]^2 y_{1,1,1,1} z_{1,1,1,1} C 2 t x_{1,1,1,1} y[ ] y_{1,1,1,1} z[ ]$   
 $K 4 t x_{1,1,1,1} y[ ] y_{1,1,1,1} z[ ] C 3 t x_{1,1,1,1} y[ ]^2 y_{1,1,1,1} z_{1,1,1,1} K 3 t x_{1,1,1,1} y[ ]^2 y_{1,1,1,1} z_{1,1,1,1}$   
 $K t x_{1,1,1,1} y[ ]^2 y_{1,1,1,1} z_{1,1,1,1} K 2 t x_{1,1,1,1} y[ ] y_{1,1,1,1} z[ ] C 3 t x_{1,1,1,1} y[ ] y_{1,1,1,1}^2 z[ ]$   
 $K 3 x[ ]^2 y[ ] y_{1,1} z_{1,1} z_{1,1,1,1} C 4 x[ ]^2 y[ ] y_{1,1} z_{1,1,1,1}^2 C 2 x[ ]^2 y[ ] y_{1,1,1,1} z_{1,1,1,1,1}$   
 $K 4 x[ ]^2 y[ ] y_{1,1,1,1} z_{1,1,1,1} K 2 x[ ]^2 y[ ] y_{1,1,1,1} z_{1,1,1,1} C 3 x[ ]^2 y[ ] y_{1,1,1,1,1}$   
 $z_{1,1}^2 K 2 x[ ] x_1 y[ ] y_{1,1,1,1} z[ ] z_{1,1,1,1,1} C 2 x[ ] x_1 y[ ] y_{1,1,1,1,1} z[ ] z_{1,1,1,1}$   
 $C 3 x[ ] x_{1,1} y[ ]^2 z_{1,1} z_{1,1,1,1} K 4 x[ ] x_{1,1} y[ ]^2 z_{1,1,1,1}^2$   
 $C 3 x[ ] x_{1,1} y[ ] y_{1,1} z[ ] z_{1,1,1,1,1} C 4 x[ ] x_{1,1} y[ ] y_{1,1,1,1} z[ ] z_{1,1,1,1}$   
 $K 6 x[ ] x_{1,1} y[ ] y_{1,1,1,1} z[ ] z_{1,1} K 2 x[ ] x_{1,1,1,1} y[ ]^2 z_{1,1} z_{1,1,1,1,1}$   
 $C 4 x[ ] x_{1,1,1,1} y[ ]^2 z_{1,1} z_{1,1,1,1} K 8 x[ ] x_{1,1,1,1} y[ ] y_{1,1} z[ ] z_{1,1,1,1}$   
 $C 4 x[ ] x_{1,1,1,1} y[ ] y_{1,1,1,1} z[ ] z_{1,1} C 2 x[ ] x_{1,1,1,1} y[ ] y_{1,1,1,1} z[ ] z_{1,1}$

$$\begin{aligned}
& C 2 x [ ] x_{1,1,1,1} y [ ]^2 z_{1,1,1} K 3 x [ ] x_{1,1,1,1} y [ ]^2 z_{1,1}^2 \\
& C 3 x [ ] x_{1,1,1,1} y [ ] y_{1,1} z [ ] z_{1,1} K 2 x [ ] x_{1,1,1,1} y [ ] y_{1,1} z [ ] z_{1,1} \\
& C 2 x_1 x_{1,1,1,1} y [ ]^2 z [ ] z_{1,1,1,1} K 2 x_1 x_{1,1,1,1} y [ ] y_{1,1,1,1} z [ ]^2 \\
& K 2 x_1 x_{1,1,1,1} y [ ]^2 z [ ] z_{1,1,1} C 2 x_1 x_{1,1,1,1} y [ ] y_{1,1,1} z [ ]^2 K 3 \\
& x_{1,1}^2 y [ ]^2 z [ ] z_{1,1,1,1} C 3 x_{1,1}^2 y [ ] y_{1,1,1,1} z [ ]^2 C 4 x_{1,1} x_{1,1,1,1} y [ ]^2 z [ ] z_{1,1,1} \\
& K 4 x_{1,1} x_{1,1,1,1} y [ ] y_{1,1,1} z [ ]^2 C 3 x_{1,1} x_{1,1,1,1} y [ ]^2 z [ ] z_{1,1} \\
& K 3 x_{1,1} x_{1,1,1,1} y [ ] y_{1,1} z [ ]^2 K 4 x_{1,1,1,1}^2 y [ ]^2 z [ ] z_{1,1} C 4 x_{1,1,1,1}^2 y [ ] y_{1,1} z [ ]^2 \\
& K x [ ] y [ ]^2 y_{1,1,1} z_{1,1,1,1} C x [ ] y [ ]^2 y_{1,1,1,1} z_{1,1,1} C x_{1,1,1,1} y [ ]^3 z_{1,1,1,1} \\
& K x_{1,1,1,1} y [ ]^2 y_{1,1,1,1} z [ ] K x_{1,1,1,1} y [ ]^3 z_{1,1,1} C x_{1,1,1,1} y [ ]^2 y_{1,1,1} z [ ]
\end{aligned}$$

M >

## Hypersurfaces in 4-dimensions

M > restart with(DifferentialGeometry) : with(Tensor) : with(JetCalculus) :  
with(Tools) :

M > DGsetup([x, y, z], [u], M, 3) :

M > Preferences("JetNotation", "JetNotation1") :

M > ω d evalDG(dx &w dz C dy &w du [ ])

$$\omega d \quad dx \ Y dz \ C dy \ Y du [ ] \quad (2.1)$$

This time too, we have the invariant vector v0

M > v0 d evalDG(x D\_x C y D\_y C z D\_z C u [ ] D\_u [ ])

$$v0 d \quad x D_x C y D_y C z D_z C u [ ] D_u [ ] \quad (2.2)$$

Input a non-canonical basis for T\_pM and use this to compute a non-canonical basis for the orthogonal complement with respect to ω

M > X d evalDG(D\_x C u [1] D\_u [ ] ) : Y d evalDG(D\_y C u [2] D\_u [ ] ) : Z  
d evalDG(D\_z C u [3] D\_u [ ] ) :

M > solve( { Hook( [X, evalDG(a D\_x C b D\_y C c D\_z C d D\_u [ ] ) ], ω ), Hook( [Y,  
evalDG(a D\_x C b D\_y C c D\_z C d D\_u [ ] ) ], ω ), Hook( [Z, evalDG(a D\_x  
C b D\_y C c D\_z C d D\_u [ ] ) ], ω ) }, {a, b, c, d} )

$$\{a = k u_3 b, b = b, c = u_1 b, d = u_2 b\} \quad (2.3)$$

Take b = 1, this gives the vector

M > w1 d evalDG(k u [3] D\_x C D\_y C u [1] D\_z C u [2] D\_u [ ] ) :

which can used to do normalization, obtaining the first invariant horizontal vector

M > tmp1 d solve(Hook([v0, k1 w1], ω) K 1, k1) :

M > v1 d evalDG(tmp1 w1)

$$v1 d \quad k \frac{u_3 D_x}{x u_1 C y u_2 C z u_3 K u [ ]} C \frac{D_y}{x u_1 C y u_2 C z u_3 K u [ ]} \quad (2.4)$$

$$C \frac{u_1 D_z}{x u_1 C y u_2 C z u_3 K u [ ]} C \frac{u_2 D_u [ ]}{x u_1 C y u_2 C z u_3 K u [ ]}$$

Next, take a representative q = -u + u(x,y,z) for the hypersurface and compute its differential

M > dq d evalDG(k du [ ] C u [1] dx C u [2] dy C u [3] dz) :

The symmetric differential and the differentiaial shares the same scaling factor, which we know compute

**M** > tmp2 d solve(Hook(k2 v0, dq) K 1, k2)

$$\text{tmp2 d } \frac{1}{x u_1 C y u_2 C z u_3 K u[ ]} \quad (2.5)$$

hence the symmetric differential is

**M** > Q d evalDG(tmp2 ( u[1, 1] dx &s dx C 2 u[1, 2] dx &s dy C 2 u[1, 3] dx &s dz C u[2, 2] dy &s dy C 2 u[2, 3] dy &s dz C u[3, 3] dz &s dz ))

$$\begin{aligned} Q d & \frac{u_{1,1} dx}{x u_1 C y u_2 C z u_3 K u[ ]} dx C \frac{u_{1,2} dx}{x u_1 C y u_2 C z u_3 K u[ ]} dy \\ & C \frac{u_{1,3} dx}{x u_1 C y u_2 C z u_3 K u[ ]} dz C \frac{u_{1,2} dy}{x u_1 C y u_2 C z u_3 K u[ ]} dx \\ & C \frac{u_{2,2} dy}{x u_1 C y u_2 C z u_3 K u[ ]} dy C \frac{u_{2,3} dy}{x u_1 C y u_2 C z u_3 K u[ ]} dz \\ & C \frac{u_{1,3} dz}{x u_1 C y u_2 C z u_3 K u[ ]} dx C \frac{u_{2,3} dz}{x u_1 C y u_2 C z u_3 K u[ ]} dy \\ & C \frac{u_{3,3} dz}{x u_1 C y u_2 C z u_3 K u[ ]} dz \end{aligned} \quad (2.6)$$

which gives the first invariant as

**M** > I2a d Hook([v1, v1], Q)

$$I_{2a} d \frac{u_1^2 u_{3,3} K 2 u_1 u_3 u_{1,3} C u_3^2 u_{1,1} C 2 u_1 u_{2,3} K 2 u_3 u_{1,2} C u_{2,2}}{(x u_1 C y u_2 C z u_3 K u[ ])^3} \quad (2.7)$$

Input more information we have gathered

**M** > α d Hook(v0, ω)

$$\alpha d k z dx K u[ ] dy C x dz C y du[ ] \quad (2.8)$$

**M** > β d convert(ContractIndices(Q &t v1, [[1, 3]]), DGform)

$$\begin{aligned} \beta d & \frac{(u_1 u_{1,3} K u_3 u_{1,1} C u_{1,2}) dx}{(x u_1 C y u_2 C z u_3 K u[ ])^2} C \frac{(u_1 u_{2,3} K u_3 u_{1,2} C u_{2,2}) dy}{(x u_1 C y u_2 C z u_3 K u[ ])^2} \\ & C \frac{(u_1 u_{3,3} K u_3 u_{1,3} C u_{2,3}) dz}{(x u_1 C y u_2 C z u_3 K u[ ])^2} \end{aligned} \quad (2.9)$$

using α and β we can find the missing invariant horizontal vectors needed. Pick a basis for T\_{p}M and use it to construct a basis for ker α

**M** > W d evalDG(a X C b Y C c Z) :

**M** > tmp3 d solve(Hook(W, α), {a, b, c})

$$\text{tmp3 d } \left\{ a = k \frac{b y u_2 C c y u_3 K u[ ] b C x c}{y u_1 K z}, b = b, c = c \right\} \quad (2.10)$$

**M** > W1 d evalDG(K(y u[1] K z) DGsimplify(eval(eval(W, tmp3), {b = 1, c = 0}))) :

**M** > W2 d evalDG(K(y u[1] K z) DGsimplify(eval(eval(W, tmp3), {b = 0, c = 1}))) :

using this basis we can take a general vector in ker α

**M** > w2 d evalDG(a W1 C b W2) : w3 d evalDG(c W1 C d W2) :

then we solve and fix a,b,c,d by the conditions we have described in the paper

**M** > tmp4 d solve({Hook([v1, w3], Q), Hook([w2, w3], Q), Hook([v1, w2], Q) K 1, Hook([w2, w3], ω) K 1}, {a, b, c, d}) :

this gives the final vectors

**M** > v2 d subs(tmp4, w2) : v3 d subs(tmp4, w3) :

which can know be used to compute our remaining invariants

**M** > I<sub>2b</sub> d Hook([v2, v2], Q); I<sub>2c</sub> d Hook([v3, v3], Q)

$$I_{2b} d \left( (x u_1 C y u_2 C z u_3 K u [ ] )^3 \left( y^2 u_1^2 u_{2,2} u_{3,3} K y^2 u_1^2 u_{2,3}^2 K 2 y^2 u_1 u_2 u_{1,2} u_{3,3} C 2 y^2 u_1 u_2 u_{1,3} u_{2,3} C 2 y^2 u_1 u_3 u_{1,2} u_{2,3} K 2 y^2 u_1 u_3 u_{1,3} u_{2,2} C y^2 u_2^2 u_{1,1} u_{3,3} K y^2 u_2^2 u_{1,3}^2 K 2 y^2 u_2 u_3 u_{1,1} u_{2,3} C 2 y^2 u_2 u_3 u_{1,2} u_{1,3} C y^2 u_3^2 u_{1,1} u_{2,2} K y^2 u_3^2 u_{1,2}^2 C 2 x y u_1 u_{1,2} u_{2,3} K 2 x y u_1 u_{1,3} u_{2,2} K 2 x y u_2 u_{1,1} u_{2,3} C 2 x y u_2 u_{1,2} u_{1,3} C 2 x y u_3 u_{1,1} u_{2,2} K 2 x y u_3 u_{1,2}^2 K 2 y z u_1 u_{2,2} u_{3,3} C 2 y z u_1 u_{2,3}^2 C 2 y z u_2 u_{1,2} u_{3,3} K 2 y z u_2 u_{1,3} u_{2,3} K 2 y z u_3 u_{1,2} u_{2,3} C 2 y z u_3 u_{1,3} u_{2,2} C 2 y u [ ] u_1 u_{1,2} u_{3,3} K 2 y u [ ] u_1 u_{1,3} u_{2,3} K 2 y u [ ] u_2 u_{1,1} u_{3,3} C 2 y u [ ] u_2 u_{1,3}^2 C 2 y u [ ] u_3 u_{1,1} u_{2,3} K 2 y u [ ] u_3 u_{1,2} u_{1,3} C x^2 u_{1,1} u_{2,2} K x^2 u_{1,2}^2 K 2 x z u_{1,2} u_{2,3} C 2 x z u_{1,3} u_{2,2} C 2 x u [ ] u_{1,1} u_{2,3} K 2 x u [ ] u_{1,2} u_{1,3} C z^2 u_{2,2} u_{3,3} K z^2 u_{2,3}^2 K 2 z u [ ] u_{1,2} u_{3,3} C 2 z u [ ] u_{1,3} u_{2,3} C u [ ]^2 u_{1,1} u_{3,3} K u [ ]^2 u_{1,3}^2 \right) / \left( y^2 u_1^4 u_{2,2} u_{3,3}^2 K y^2 u_1^4 u_{2,3}^2 u_{3,3} K 2 y^2 u_1^3 u_2 u_{1,2} u_{3,3}^2 C 2 y^2 u_1^3 u_2 u_{1,3} u_{2,3} u_{3,3} C 2 y^2 u_1^3 u_3 u_{1,2} u_{2,3} u_{3,3} K 4 y^2 u_1^3 u_3 u_{1,3} u_{2,2} u_{3,3} C 2 y^2 u_1^3 u_3 u_{1,3} u_{2,3}^2 C y^2 u_1^2 u_2^2 u_{1,1} u_{3,3}^2 K y^2 u_1^2 u_2^2 u_{1,3}^2 u_{3,3} K 2 y^2 u_1^2 u_2 u_3 u_{1,1} u_{2,3} u_{3,3} C 6 y^2 u_1^2 u_2 u_3 u_{1,2} u_{1,3} u_{3,3} K 4 y^2 u_1^2 u_2 u_3 u_{1,3}^2 u_{2,3} C 2 y^2 u_1^2 u_3^2 u_{1,1} u_{2,2} u_{3,3} K y^2 u_1^2 u_3^2 u_{1,1} u_{2,3}^2 K y^2 u_1^2 u_3^2 u_{1,2}^2 u_{3,3} K 4 y^2 u_1^2 u_3^2 u_{1,2} u_{1,3} u_{2,3} C 4 y^2 u_1^2 u_3^2 u_{1,3}^2 u_{2,2} K 2 y^2 u_1 u_2^2 u_3 u_{1,1} u_{1,3} u_{3,3} C 2 y^2 u_1 u_2^2 u_3 u_{1,3}^3 K 2 y^2 u_1 u_2 u_3^2 u_{1,1} u_{1,2} u_{3,3} C 6 y^2 u_1 u_2 u_3^2 u_{1,1} u_{1,3} u_{2,3} K 4 y^2 u_1 u_2 u_3^2 u_{1,2} u_{1,3}^2 C 2 y^2 u_1 u_3^3 u_{1,2} u_{1,3} C 2 y^2 u_1 u_3^3 u_{1,1} u_{1,2} u_{2,3} K 4 y^2 u_1 u_3^3 u_{1,1} u_{1,3} u_{2,2} C 2 y^2 u_2 u_3^3 u_{1,1} u_{1,2} u_{1,3} C y^2 u_3^4 u_{1,1}^2 u_{2,2} K y^2 u_3^4 u_{1,1} u_{1,2}^2 C 2 x y u_1^3 u_{1,2} u_{2,3} u_{3,3} K 2 x y u_1^3 u_{1,3} u_{2,2} u_{3,3} K 2 x y u_1^2 u_2 u_{1,1} u_{2,3} u_{3,3} C 2 x y u_1^2 u_2 u_{1,2} u_{1,3} u_{3,3} C 2 x y u_1^2 u_3 u_{1,1} u_{2,2} u_{3,3} K 2 x y u_1^2 u_3 u_{1,2}^2 u_{3,3} K 4 x y u_1^2 u_3 u_{1,2} u_{1,3} u_{2,3} C 4 x y u_1^2 u_3 u_{1,3}^2 u_{2,2} C 4 x y u_1 u_2 u_3 u_{1,1} u_{1,3} u_{2,3} K 4 x y u_1 u_2 u_3 u_{1,2} u_{1,3}^2 C 2 x y u_1 u_2^2 u_{1,1} u_{1,2} u_{2,3} K 6 x y u_1 u_3^2 u_{1,1} u_{1,3} u_{2,2} C 4 x y u_1 u_3^2 u_{1,2} u_{1,3} K 2 x y u_2 u_3^2 u_{1,1} u_{2,3} C 2 x y u_2 u_3^2 u_{1,1} u_{1,2} u_{1,3} C 2 x y u_3^3 u_{1,1} u_{1,2} K 2 x y u_3^3 u_{1,1} u_{1,2}^2 C 2 y^2 u_1^3 u_{2,2} u_{2,3} u_{3,3} K 2 y^2 u_1^3 u_{2,3}^2 K 4 y^2 u_1^2 u_2 u_{1,2} u_{2,3} u_{3,3} C 4 y^2 u_1^2 u_2 u_{1,3} u_{2,3}^2 K 2 y^2 u_1^2 u_3 u_{1,2} u_{2,2} u_{3,3} C 6 y^2 u_1^2 u_3 u_{1,2} u_{2,3}^2 K 4 y^2 u_1^2 u_3 u_{1,3} u_{2,2} u_{2,3} C 2 y^2 u_1 u_2^2 u_{1,1} u_{2,3} u_{3,3} K 2 y^2 u_1 u_2^2 u_{1,3}^2 u_{2,3} K 4 y^2 u_1 u_2 u_3 u_{1,1} u_{2,3}^2 C 4 y^2 u_1 u_2 u_3 u_{1,2}^2 u_{3,3} \right)$$

$$\begin{aligned}
& C 2 y^2 u_1 u_3^2 u_{1,1} u_{2,2} u_{2,3} K 6 y^2 u_1 u_3^2 u_{1,2}^2 u_{2,3} C 4 y^2 u_1 u_3^2 u_{1,2} u_{1,3} u_{2,2} K 2 y^2 \\
& u_2^2 u_3 u_{1,1} u_{1,2} u_{3,3} C 2 y^2 u_2^2 u_3 u_{1,2} u_{1,3}^2 C 4 y^2 u_2 u_3^2 u_{1,1} u_{1,2} u_{2,3} K 4 y^2 u_2 u_3^2 \\
& u_{1,2}^2 u_{1,3} K 2 y^2 u_3^3 u_{1,1} u_{1,2} u_{2,2} C 2 y^2 u_3^3 u_{1,2}^2 K 2 y z u_1^3 u_{2,2} u_{2,3}^2 C 2 y z u_1^3 u_{2,3}^2 u_{3,3} \\
& C 2 y z u_1^2 u_2 u_{1,2} u_{2,3}^2 K 2 y z u_1^2 u_2 u_{1,3} u_{2,3} u_{3,3} K 2 y z u_1^2 u_3 u_{1,2} u_{2,3} u_{3,3} C 6 y z \\
& u_1^2 u_3 u_{1,3} u_{2,2} u_{3,3} K 4 y z u_1^2 u_3 u_{1,3} u_{2,3}^2 K 4 y z u_1 u_2 u_3 u_{1,2} u_{1,3} u_{3,3} \\
& C 4 y z u_1 u_2 u_3 u_{1,3}^2 u_{2,3} K 2 y z u_1 u_3^2 u_{1,1} u_{2,2} u_{3,3} C 2 y z u_1 u_3^2 u_{1,1} u_{2,3}^2 C 4 y z u_1 \\
& u_3^2 u_{1,2} u_{1,3} u_{2,3} K 4 y z u_1 u_3^2 u_{1,3}^2 u_{2,2} C 2 y z u_2 u_3^2 u_{1,1} u_{1,2} u_{3,3} K 2 y z u_2 \\
& u_3^2 u_{1,1} u_{1,3} u_{2,3} K 2 y z u_3^3 u_{1,1} u_{1,2} u_{2,3} C 2 y z u_3^3 u_{1,1} u_{1,3} u_{2,2} C 2 y u [ ] u_1^3 u_{1,2} \\
& u_{3,3}^2 K 2 y u [ ] u_1^3 u_{1,3} u_{2,3} u_{3,3} K 2 y u [ ] u_1^2 u_2 u_{1,1} u_{3,3}^2 C 2 y u [ ] u_1^2 u_2 u_{1,3}^2 u_{3,3} \\
& C 2 y u [ ] u_1^2 u_3 u_{1,1} u_{2,3} u_{3,3} K 6 y u [ ] u_1^2 u_3 u_{1,2} u_{1,3} u_{3,3} C 4 y u [ ] u_1^2 u_3 u_{1,3}^2 u_{2,3} \\
& C 4 y u [ ] u_1 u_2 u_3 u_{1,1} u_{1,3} u_{3,3} K 4 y u [ ] u_1 u_2 u_3 u_{1,3}^3 C 2 y u [ ] u_1 u_3^2 u_{1,1} u_{1,2} u_{3,3} \\
& K 6 y u [ ] u_1 u_3^2 u_{1,1} u_{1,3} u_{2,3} C 4 y u [ ] u_1 u_3^2 u_{1,2} u_{1,3}^2 K 2 y u [ ] u_2 u_3^2 u_{1,1}^2 u_{3,3} \\
& C 2 y u [ ] u_2 u_3^2 u_{1,1} u_{1,3}^2 C 2 y u [ ] u_3^3 u_{1,1}^2 u_{2,3} K 2 y u [ ] u_3^3 u_{1,1} u_{1,2} u_{1,3} C x^2 \\
& u_1^2 u_{1,1} u_{2,3}^2 K 2 x^2 u_1^2 u_{1,2} u_{1,3} u_{2,3} C x^2 u_1^2 u_{1,3}^2 u_{2,2} K 2 x^2 u_1 u_3 u_{1,1} u_{1,3} u_{2,2} \\
& C 2 x^2 u_1 u_3 u_{1,2}^2 u_{1,3} C u_{2,2} u_{1,1}^2 u_3^2 x^2 K u_{1,2}^2 u_{1,1} u_3^2 x^2 C 4 x y u_1^2 u_{1,2} u_{2,3}^2 K 4 x y \\
& u_1^2 u_{1,3} u_{2,2} u_{2,3} K 2 x y u_1 u_2 u_{1,1} u_{2,2} u_{3,3} K 2 x y u_1 u_2 u_{1,1} u_{2,3}^2 C 2 x y u_1 u_2 \\
& u_{1,2}^2 u_{3,3} C 2 x y u_1 u_2 u_{1,3}^2 u_{2,2} C 4 x y u_1 u_3 u_{1,1} u_{2,2} u_{2,3} K 8 x y u_1 u_3 u_{1,2}^2 u_{2,3} \\
& C 4 x y u_1 u_3 u_{1,2} u_{1,3} u_{2,2} C 4 x y u_2 u_3 u_{1,1} u_{1,2} u_{2,3} K 4 x y u_2 u_3 u_{1,2}^2 u_{1,3} K 4 x y \\
& u_3^2 u_{1,1} u_{1,2} u_{2,2} C 4 x y u_3^2 u_{1,2}^3 K 2 x z u_1^2 u_{1,2} u_{2,3} u_{3,3} C 2 x z u_1^2 u_{1,3} u_{2,2} u_{3,3} \\
& K 2 x z u_1 u_3 u_{1,1} u_{2,2} u_{3,3} C 2 x z u_1 u_3 u_{1,1} u_{2,3}^2 C 2 x z u_1 u_3 u_{1,2}^2 u_{3,3} K 2 x z u_1 u_3 \\
& u_{1,3}^2 u_{2,2} K 2 x z u_3^2 u_{1,1} u_{1,2} u_{2,3} C 2 x z u_3^2 u_{1,1} u_{1,3} u_{2,2} C 2 x u [ ] u_1^2 u_{1,1} u_{2,3} u_{3,3} \\
& K 2 x u [ ] u_1^2 u_{1,2} u_{1,3} u_{3,3} K 4 x u [ ] u_1 u_3 u_{1,1} u_{1,3} u_{2,3} C 4 x u [ ] u_1 u_3 u_{1,2} u_{1,3}^2 \\
& C 2 u_{2,3} u_{1,1}^2 u_3^2 u [ ] x K 2 u_{1,3} u_{1,2} u_{1,1} u_3^2 u [ ] x C y^2 u_1^2 u_{2,2}^2 u_{3,3} K y^2 u_1^2 u_{2,2}^2 u_{2,3}^2 \\
& K 2 y^2 u_1 u_2 u_{1,2} u_{2,2} u_{3,3} C 2 y^2 u_1 u_2 u_{1,3} u_{2,2} u_{2,3} C 2 y^2 u_1 u_3 u_{1,2} u_{2,2} u_{2,3} \\
& K 2 y^2 u_1 u_3 u_{1,3} u_{2,2}^2 C y^2 u_2^2 u_{1,1} u_{2,3}^2 C y^2 u_2^2 u_{1,2}^2 u_{3,3} K 2 y^2 u_2^2 u_{1,2} u_{1,3} u_{2,3} \\
& K 2 y^2 u_2 u_3 u_{1,1} u_{2,2} u_{2,3} C 2 y^2 u_2 u_3 u_{1,2} u_{1,3} u_{2,2} C y^2 u_3^2 u_{1,1} u_{2,2}^2 K y^2 u_3^2 u_{1,2}^2 u_{2,2}^2 \\
& K 4 y z u_1^2 u_{2,2} u_{2,3} u_{3,3} C 4 y z u_1^2 u_{2,3}^3 C 4 y z u_1 u_2 u_{1,2} u_{2,3} u_{3,3} K 4 y z u_1 u_2 u_{1,3} \\
& u_{2,3}^2 C 4 y z u_1 u_3 u_{1,2} u_{2,2} u_{3,3} K 8 y z u_1 u_3 u_{1,2} u_{2,3}^2 C 4 y z u_1 u_3 u_{1,3} u_{2,2} u_{2,3} \\
& K 2 y z u_2 u_3 u_{1,1} u_{2,2} u_{3,3} C 2 y z u_2 u_3 u_{1,1} u_{2,3}^2 K 2 y z u_2 u_3 u_{1,2}^2 u_{3,3} C 2 y z u_2 u_3 \\
& u_{1,3}^2 u_{2,2} C 4 y z u_3^2 u_{1,2}^2 u_{2,3} K 4 y z u_3^2 u_{1,2} u_{1,3} u_{2,2} C 4 y u [ ] u_1^2 u_{1,2} u_{2,3} u_{3,3} \\
& K 4 y u [ ] u_1^2 u_{1,3} u_{2,3}^2 K 4 y u [ ] u_1 u_2 u_{1,1} u_{2,3} u_{3,3} C 4 y u [ ] u_1 u_2 u_{1,3}^2 u_{2,3} \\
& C 4 y u [ ] u_1 u_3 u_{1,1} u_{2,3}^2 K 4 y u [ ] u_1 u_3 u_{1,2}^2 u_{3,3} C 4 y u [ ] u_2 u_3 u_{1,1} u_{1,2} u_{3,3}
\end{aligned}$$

$$\begin{aligned}
& K 4 y u [ ] u_2 u_3 u_{1,2} u_{1,3}^2 K 4 y u [ ] u_3^2 u_{1,1} u_{1,2} u_{2,3} C 4 y u [ ] u_3^2 u_{1,2}^2 u_{1,3} C z^2 \\
& u_1^2 u_{2,2} u_{3,3}^2 K z^2 u_1^2 u_{2,3}^2 u_{3,3} K 2 z^2 u_1 u_3 u_{1,3} u_{2,2} u_{3,3} C 2 z^2 u_1 u_3 u_{1,3} u_{2,3}^2 C z^2 u_3^2 \\
& u_{1,2}^2 u_{3,3} K 2 z^2 u_3^2 u_{1,2} u_{1,3} u_{2,3} C z^2 u_3^2 u_{1,3}^2 u_{2,2} K 2 z u [ ] u_1^2 u_{1,2} u_{3,3}^2 C 2 z u [ ] \\
& u_1^2 u_{1,3} u_{2,3} u_{3,3} C 4 z u [ ] u_1 u_3 u_{1,2} u_{1,3} u_{3,3} K 4 z u [ ] u_1 u_3 u_{1,3}^2 u_{2,3} K 2 z u [ ] \\
& u_3^2 u_{1,1} u_{1,2} u_{3,3} C 2 z u [ ] u_3^2 u_{1,1} u_{1,3} u_{2,3} C u [ ]^2 u_1^2 u_{1,1} u_{3,3}^2 K u [ ]^2 u_1^2 u_{1,3}^2 u_{3,3} \\
& K 2 u [ ]^2 u_1 u_3 u_{1,1} u_{1,3} u_{3,3} C 2 u [ ]^2 u_1 u_3 u_{1,3}^3 C u_{3,3} u_{1,1}^2 u_3^2 u [ ]^2 K u_{1,3}^2 u_{1,1} \\
& u_3^2 u [ ]^2 C 2 x^2 u_1 u_{1,1} u_{2,2} u_{2,3} K 2 x^2 u_1 u_{1,2}^2 u_{2,3} K 2 u_{2,2} u_{1,2} u_{1,1} u_3 x^2 C 2 \\
& u_{1,2}^3 u_3 x^2 C 2 x y u_1 u_{1,2} u_{2,2} u_{2,3} K 2 x y u_1 u_{1,3} u_{2,2}^2 K 2 x y u_2 u_{1,1} u_{2,2} u_{2,3} \\
& C 2 x y u_2 u_{1,2} u_{1,3} u_{2,2} C 2 x y u_3 u_{1,1} u_{2,2}^2 K 2 x y u_3 u_{1,2}^2 u_{2,2} K 4 x z u_1 u_{1,2} u_{2,3}^2 \\
& C 4 x z u_1 u_{1,3} u_{2,2} u_{2,3} C 4 x z u_3 u_{1,2}^2 u_{2,3} K 4 x z u_3 u_{1,2} u_{1,3} u_{2,2} \\
& C 2 x u [ ] u_1 u_{1,1} u_{2,2} u_{3,3} C 2 x u [ ] u_1 u_{1,1} u_{2,3}^2 K 2 x u [ ] u_1 u_{1,2}^2 u_{3,3} K 2 x u [ ] u_1 \\
& u_{1,3}^2 u_{2,2} K 4 u_{2,3} u_{1,2} u_{1,1} u_3 u [ ] x C 4 u_{1,3} u_{1,2}^2 u_3 u [ ] x K 2 y z u_1 u_{2,2}^2 u_{3,3} \\
& C 2 y z u_1 u_{2,2} u_{2,3}^2 C 2 y z u_2 u_{1,2} u_{2,2} u_{3,3} K 2 y z u_2 u_{1,3} u_{2,2} u_{2,3} \\
& K 2 y z u_3 u_{1,2} u_{2,2} u_{2,3} C 2 y z u_3 u_{1,3} u_{2,2}^2 C 2 y u [ ] u_1 u_{1,2} u_{2,2} u_{3,3} \\
& K 2 y u [ ] u_1 u_{1,3} u_{2,2} u_{2,3} K 2 y u [ ] u_2 u_{1,1} u_{2,3}^2 K 2 y u [ ] u_2 u_{1,2}^2 u_{3,3} \\
& C 4 y u [ ] u_2 u_{1,2} u_{1,3} u_{2,3} C 2 y u [ ] u_3 u_{1,1} u_{2,2} u_{2,3} K 2 y u [ ] u_3 u_{1,2} u_{1,3} u_{2,2} \\
& C 2 z^2 u_1 u_{2,2} u_{2,3} u_{3,3} K 2 z^2 u_1 u_{2,3}^3 K 2 z^2 u_3 u_{1,2} u_{2,2} u_{3,3} C 2 z^2 u_3 u_{1,2} u_{2,3}^2 \\
& K 4 z u [ ] u_1 u_{1,2} u_{2,3} u_{3,3} C 4 z u [ ] u_1 u_{1,3} u_{2,3}^2 C 2 z u [ ] u_3 u_{1,1} u_{2,2} u_{3,3} \\
& K 2 z u [ ] u_3 u_{1,1} u_{2,3}^2 C 2 z u [ ] u_3 u_{1,2}^2 u_{3,3} K 2 z u [ ] u_3 u_{1,3}^2 u_{2,2} \\
& C 2 u [ ]^2 u_1 u_{1,1} u_{2,3} u_{3,3} K 2 u [ ]^2 u_1 u_{1,3}^2 u_{2,3} K 2 u_{3,3} u_{1,2} u_{1,1} u_3 u [ ]^2 C 2 \\
& u_{1,3}^2 u_{1,2} u_3 u [ ]^2 C u_{2,2}^2 u_{1,1} x^2 K u_{2,2} u_{1,2}^2 x^2 K 2 x z u_{1,2} u_{2,2} u_{2,3} C 2 x z u_{1,3} u_{2,2}^2 \\
& C 2 u_{2,3} u_{2,2} u_{1,1} u [ ] x K 2 u_{2,2} u_{1,3} u_{1,2} u [ ] x C z^2 u_{2,2}^2 u_{3,3} K z^2 u_{2,2} u_{2,3}^2 \\
& K 2 z u [ ] u_{1,2} u_{2,2} u_{3,3} C 2 z u [ ] u_{1,3} u_{2,2} u_{2,3} C u_{2,3}^2 u_{1,1} u [ ]^2 C u_{3,3} u_{1,2}^2 u [ ]^2 \\
& K 2 u_{2,3} u_{1,3} u_{1,2} u [ ]^2)
\end{aligned}$$

$$\begin{aligned}
I_{2c} d & (y^2 u_1^4 u_{2,2} u_{3,3}^2 K y^2 u_1^4 u_{2,3}^2 u_{3,3} K 2 y^2 u_1^3 u_2 u_{1,2} u_{3,3}^2 C 2 y^2 u_1^3 u_2 u_{1,3} u_{2,3} u_{3,3} \\
& C 2 y^2 u_1^3 u_3 u_{1,2} u_{2,3} u_{3,3} K 4 y^2 u_1^3 u_3 u_{1,3} u_{2,2} u_{3,3} C 2 y^2 u_1^3 u_3 u_{1,3} u_{2,3}^2 C y^2 u_1^2 \\
& u_{2,2}^2 u_{1,1} u_{3,3}^2 K y^2 u_1^2 u_{2,2}^2 u_{3,3}^2 K 2 y^2 u_1^2 u_2 u_3 u_{1,1} u_{2,3} u_{3,3} C 6 y^2 \\
& u_1^2 u_2 u_3 u_{1,2} u_{1,3} u_{3,3} K 4 y^2 u_1^2 u_2 u_3 u_{1,3}^2 u_{2,3} C 2 y^2 u_1^2 u_3^2 u_{1,1} u_{2,2} u_{3,3} K y^2 u_1^2 \\
& u_3^2 u_{1,1} u_{2,3}^2 K y^2 u_1^2 u_3^2 u_{1,2}^2 u_{3,3} K 4 y^2 u_1^2 u_3^2 u_{1,2} u_{1,3} u_{2,3} C 4 y^2 u_1^2 u_3^2 u_{1,3}^2 u_{2,2} \\
& K 2 y^2 u_1 u_2^2 u_3 u_{1,1} u_{1,3} u_{3,3} C 2 y^2 u_1 u_2^2 u_3 u_{1,3}^3 K 2 y^2 u_1 u_2 u_3^2 u_{1,1} u_{1,2} u_{3,3} \\
& C 6 y^2 u_1 u_2 u_3^2 u_{1,1} u_{1,3} u_{2,3} K 4 y^2 u_1 u_2 u_3^2 u_{1,2} u_{1,3}^2 C 2 y^2 u_1 u_3^3 u_{1,1} u_{1,2} u_{2,3} \\
& K 4 y^2 u_1 u_3^3 u_{1,1} u_{1,3} u_{2,2} C 2 y^2 u_1 u_3^3 u_{1,2}^2 u_{1,3} C y^2 u_2^2 u_3^2 u_{1,1} u_{3,3} K y^2 u_2^2 u_3^2 u_{1,1}
\end{aligned} \tag{2.11}$$

$$\begin{aligned}
& u_{1,3}^2 K 2 y^2 u_2 u_3^3 u_{1,1}^2 u_{2,3} C 2 y^2 u_2 u_3^3 u_{1,1} u_{1,2} u_{1,3} C y^2 u_3^4 u_{1,1}^2 u_{2,2} K y^2 u_3^4 u_{1,1} u_{1,2}^2 \\
& C 2 x y u_1^3 u_{1,2} u_{2,3} u_{3,3} K 2 x y u_1^3 u_{1,3} u_{2,2} u_{3,3} K 2 x y u_1^2 u_2 u_{1,1} u_{2,3} u_{3,3} C 2 x y \\
& u_1^2 u_2 u_{1,2} u_{1,3} u_{3,3} C 2 x y u_1^2 u_3 u_{1,1} u_{2,2} u_{3,3} K 2 x y u_1^2 u_3 u_{1,2}^2 u_{3,3} K 4 x y \\
& u_1^2 u_3 u_{1,2} u_{1,3} u_{2,3} C 4 x y u_1^2 u_3 u_{1,3}^2 u_{2,2} C 4 x y u_1 u_2 u_3 u_{1,1} u_{1,3} u_{2,3} \\
& K 4 x y u_1 u_2 u_3 u_{1,2} u_{1,3}^2 C 2 x y u_1 u_3^2 u_{1,1} u_{1,2} u_{2,3} K 6 x y u_1 u_3^2 u_{1,1} u_{1,3} u_{2,2} \\
& C 4 x y u_1 u_3^2 u_{1,2}^2 u_{1,3} K 2 x y u_2 u_3^2 u_{1,1}^2 u_{2,3} C 2 x y u_2 u_3^2 u_{1,1} u_{1,2} u_{1,3} C 2 x y u_3^3 \\
& u_{1,1}^2 u_{2,2} K 2 x y u_3^3 u_{1,1} u_{1,2}^2 C 2 y^2 u_1^3 u_{2,2} u_{2,3} u_{3,3} K 2 y^2 u_1^3 u_{2,3}^3 K 4 y^2 \\
& u_1^2 u_2 u_{1,2} u_{2,3} u_{3,3} C 4 y^2 u_1^2 u_2 u_{1,3} u_{2,3}^2 K 2 y^2 u_1^2 u_3 u_{1,2} u_{2,2} u_{3,3} C 6 y^2 u_1^2 u_3 u_{1,2} \\
& u_{2,3}^2 K 4 y^2 u_1^2 u_3 u_{1,3} u_{2,2} u_{2,3} C 2 y^2 u_1 u_2^2 u_{1,1} u_{2,3} u_{3,3} K 2 y^2 u_1 u_2^2 u_{1,3}^2 u_{2,3} \\
& K 4 y^2 u_1 u_2 u_3 u_{1,1} u_{2,3}^2 C 4 y^2 u_1 u_2 u_3 u_{1,2}^2 u_{3,3} C 2 y^2 u_1 u_3^2 u_{1,1} u_{2,2} u_{2,3} K 6 y^2 u_1 \\
& u_3^2 u_{1,2}^2 u_{2,3} C 4 y^2 u_1 u_3^2 u_{1,2} u_{1,3} u_{2,2} K 2 y^2 u_2^2 u_3 u_{1,1} u_{1,2} u_{3,3} C 2 y^2 u_2^2 u_3 u_{1,2} u_{1,3}^2 \\
& C 4 y^2 u_2 u_3^2 u_{1,1} u_{1,2} u_{2,3} K 4 y^2 u_2 u_3^2 u_{1,2}^2 u_{1,3} K 2 y^2 u_3^3 u_{1,1} u_{1,2} u_{2,2} C 2 y^2 u_3^3 u_{1,2}^3 \\
& K 2 y z u_1^3 u_{2,2} u_{2,3}^2 C 2 y z u_1^3 u_{2,3}^2 u_{3,3} C 2 y z u_1^2 u_2 u_{1,2} u_{3,3}^2 K 2 y z \\
& u_1^2 u_2 u_{1,3} u_{2,3} u_{3,3} K 2 y z u_1^2 u_3 u_{1,2} u_{2,3} u_{3,3} C 6 y z u_1^2 u_3 u_{1,3} u_{2,2} u_{3,3} K 4 y z \\
& u_1^2 u_3 u_{1,3} u_{2,3}^2 K 4 y z u_1 u_2 u_3 u_{1,2} u_{1,3} u_{3,3} C 4 y z u_1 u_2 u_3 u_{1,3}^2 u_{2,3} K 2 y z u_1 \\
& u_3^2 u_{1,1} u_{2,2} u_{3,3} C 2 y z u_1 u_3^2 u_{1,1} u_{2,3}^2 C 4 y z u_1 u_3^2 u_{1,2} u_{1,3} u_{2,3} K 4 y z u_1 u_3^2 \\
& u_{1,3}^2 u_{2,2} C 2 y z u_2 u_3^2 u_{1,1} u_{1,2} u_{3,3} K 2 y z u_2 u_3^2 u_{1,1} u_{1,3} u_{2,3} K 2 y z u_3^3 u_{1,1} u_{1,2} u_{2,3} \\
& C 2 y z u_3^3 u_{1,1} u_{1,3} u_{2,2} C 2 y u [ ] u_1^3 u_{1,2} u_{2,3}^2 K 2 y u [ ] u_1^3 u_{1,3} u_{2,3} u_{3,3} K 2 y u [ ] \\
& u_1^2 u_2 u_{1,1} u_{2,3}^2 C 2 y u [ ] u_1^2 u_2 u_{1,3}^2 u_{3,3} C 2 y u [ ] u_1^2 u_3 u_{1,1} u_{2,3} u_{3,3} K 6 y u [ ] \\
& u_1^2 u_3 u_{1,2} u_{1,3} u_{3,3} C 4 y u [ ] u_1^2 u_3 u_{1,3}^2 u_{2,3} C 4 y u [ ] u_1 u_2 u_3 u_{1,1} u_{1,3} u_{3,3} \\
& K 4 y u [ ] u_1 u_2 u_3 u_{1,3}^3 C 2 y u [ ] u_1 u_3^2 u_{1,1} u_{1,2} u_{3,3} K 6 y u [ ] u_1 u_3^2 u_{1,1} u_{1,3} u_{2,3} \\
& C 4 y u [ ] u_1 u_3^2 u_{1,2} u_{1,3}^2 K 2 y u [ ] u_2 u_3^2 u_{1,1}^2 u_{3,3} C 2 y u [ ] u_2 u_3^2 u_{1,1} u_{1,3}^2 \\
& C 2 y u [ ] u_3^3 u_{1,1} u_{2,3} K 2 y u [ ] u_3^3 u_{1,1} u_{1,2} u_{1,3} C x^2 u_1^2 u_{1,1} u_{2,3}^2 K 2 x^2 \\
& u_1^2 u_{1,2} u_{1,3} u_{2,3} C x^2 u_1^2 u_{1,3}^2 u_{2,2} K 2 x^2 u_1 u_3 u_{1,1} u_{1,3} u_{2,2} C 2 x^2 u_1 u_3 u_{1,2}^2 u_{1,3} \\
& C u_{2,2} u_{1,1}^2 u_3^2 x^2 K u_{1,2}^2 u_{1,1} u_3^2 x^2 C 4 x y u_1^2 u_{1,2} u_{2,3}^2 K 4 x y u_1^2 u_{1,3} u_{2,2} u_{2,3} \\
& K 2 x y u_1 u_2 u_{1,1} u_{2,2} u_{3,3} K 2 x y u_1 u_2 u_{1,1} u_{2,3}^2 C 2 x y u_1 u_2 u_{1,2}^2 u_{3,3} C 2 x y u_1 u_2 \\
& u_{1,3}^2 u_{2,2} C 4 x y u_1 u_3 u_{1,1} u_{2,2} u_{2,3} K 8 x y u_1 u_3 u_{1,2}^2 u_{2,3} C 4 x y u_1 u_3 u_{1,2} u_{1,3} u_{2,2} \\
& C 4 x y u_2 u_3 u_{1,1} u_{1,2} u_{2,3} K 4 x y u_2 u_3 u_{1,2}^2 u_{1,3} K 4 x y u_3^2 u_{1,1} u_{1,2} u_{2,2} C 4 x y u_3^2 \\
& u_{1,2}^3 K 2 x z u_1^2 u_{1,2} u_{2,3} u_{3,3} C 2 x z u_1^2 u_{1,3} u_{2,2} u_{3,3} K 2 x z u_1 u_3 u_{1,1} u_{2,2} u_{3,3} \\
& C 2 x z u_1 u_3 u_{1,1} u_{2,3}^2 C 2 x z u_1 u_3 u_{1,2}^2 u_{3,3} K 2 x z u_1 u_3 u_{1,3}^2 u_{2,2} K 2 x z \\
& u_3^2 u_{1,1} u_{1,2} u_{2,3} C 2 x z u_3^2 u_{1,1} u_{1,3} u_{2,2} C 2 x u [ ] u_1^2 u_{1,1} u_{2,3} u_{3,3} K 2 x u [ ] \\
& u_1^2 u_{1,2} u_{1,3} u_{3,3} K 4 x u [ ] u_1 u_3 u_{1,1} u_{1,3} u_{2,3} C 4 x u [ ] u_1 u_3 u_{1,2} u_{1,3}^2 C 2 u_{2,3} u_{1,1}^2
\end{aligned}$$

$$\begin{aligned}
& u_3^2 u[ ] x K 2 u_{1,3} u_{1,2} u_{1,1} u_3^2 u[ ] x C y^2 u_1^2 u_{2,2}^2 u_{3,3} K y^2 u_1^2 u_{2,2}^2 u_{2,3}^2 \\
& K 2 y^2 u_1 u_2 u_{1,2} u_{2,2} u_{3,3} C 2 y^2 u_1 u_2 u_{1,3} u_{2,2} u_{2,3} C 2 y^2 u_1 u_3 u_{1,2} u_{2,2} u_{2,3} \\
& K 2 y^2 u_1 u_3 u_{1,3} u_{2,2}^2 C y^2 u_2^2 u_{1,1} u_{2,3}^2 C y^2 u_2^2 u_{1,2}^2 u_{3,3} K 2 y^2 u_2^2 u_{1,2} u_{1,3} u_{2,3} \\
& K 2 y^2 u_2 u_3 u_{1,1} u_{2,2} u_{2,3} C 2 y^2 u_2 u_3 u_{1,2} u_{1,3} u_{2,2} C y^2 u_3^2 u_{1,1} u_{2,2}^2 K y^2 u_3^2 u_{1,2}^2 u_{2,2} \\
& K 4 y z u_1^2 u_{2,2} u_{2,3} u_{3,3} C 4 y z u_1^2 u_{2,3}^3 C 4 y z u_1 u_2 u_{1,2} u_{2,3} u_{3,3} K 4 y z u_1 u_2 u_{1,3} \\
& u_{2,3}^2 C 4 y z u_1 u_3 u_{1,2} u_{2,2} u_{3,3} K 8 y z u_1 u_3 u_{1,2} u_{2,3}^2 C 4 y z u_1 u_3 u_{1,3} u_{2,2} u_{2,3} \\
& K 2 y z u_2 u_3 u_{1,1} u_{2,2} u_{3,3} C 2 y z u_2 u_3 u_{1,1} u_{2,3}^2 K 2 y z u_2 u_3 u_{1,2}^2 u_{3,3} C 2 y z u_2 u_3 \\
& u_{1,3}^2 u_{2,2} C 4 y z u_3^2 u_{1,2}^2 u_{2,3} K 4 y z u_3^2 u_{1,2} u_{1,3} u_{2,2} C 4 y u[ ] u_1^2 u_{1,2} u_{2,3} u_{3,3} \\
& K 4 y u[ ] u_1^2 u_{1,3} u_{2,3}^2 K 4 y u[ ] u_1 u_2 u_{1,1} u_{2,3} u_{3,3} C 4 y u[ ] u_1 u_2 u_{1,3}^2 u_{2,3} \\
& C 4 y u[ ] u_1 u_3 u_{1,1} u_{2,3}^2 K 4 y u[ ] u_1 u_3 u_{1,2}^2 u_{3,3} C 4 y u[ ] u_2 u_3 u_{1,1} u_{1,2} u_{3,3} \\
& K 4 y u[ ] u_2 u_3 u_{1,2} u_{1,3}^2 K 4 y u[ ] u_3^2 u_{1,1} u_{1,2} u_{2,3} C 4 y u[ ] u_3^2 u_{1,2}^2 u_{1,3} C z^2 \\
& u_1^2 u_{2,2} u_{3,3}^2 K z^2 u_1^2 u_{2,3}^2 u_{3,3} K 2 z^2 u_1 u_3 u_{1,3} u_{2,2} u_{3,3} C 2 z^2 u_1 u_3 u_{1,3} u_{2,3}^2 C z^2 u_3^2 \\
& u_{1,2}^2 u_{3,3} K 2 z^2 u_3^2 u_{1,2} u_{1,3} u_{2,3} C z^2 u_3^2 u_{1,3}^2 u_{2,2} K 2 z u[ ] u_1^2 u_{1,2} u_{2,3}^2 C 2 z u[ ] \\
& u_1^2 u_{1,3} u_{2,3} u_{3,3} C 4 z u[ ] u_1 u_3 u_{1,2} u_{1,3} u_{3,3} K 4 z u[ ] u_1 u_3 u_{1,3}^2 u_{2,3} K 2 z u[ ] \\
& u_3^2 u_{1,1} u_{1,2} u_{3,3} C 2 z u[ ] u_3^2 u_{1,1} u_{1,3} u_{2,3} C u[ ]^2 u_1^2 u_{1,1} u_{2,3}^2 K u[ ]^2 u_1^2 u_{1,3}^2 u_{3,3} \\
& K 2 u[ ]^2 u_1 u_3 u_{1,1} u_{1,3} u_{3,3} C 2 u[ ]^2 u_1 u_3 u_{1,3}^3 C u_{3,3} u_{1,1}^2 u_3^2 u[ ]^2 K u_{1,3}^2 u_{1,1} \\
& u_3^2 u[ ]^2 C 2 x^2 u_1 u_{1,1} u_{2,2} u_{2,3} K 2 x^2 u_1 u_{1,2}^2 u_{2,3} K 2 u_{2,2} u_{1,2} u_{1,1} u_3 x^2 C 2 \\
& u_{1,2}^3 u_3 x^2 C 2 x y u_1 u_{1,2} u_{2,2} u_{2,3} K 2 x y u_1 u_{1,3} u_{2,2}^2 K 2 x y u_2 u_{1,1} u_{2,2} u_{2,3} \\
& C 2 x y u_2 u_{1,2} u_{1,3} u_{2,2} C 2 x y u_3 u_{1,1} u_{2,2}^2 K 2 x y u_3 u_{1,2}^2 u_{2,2} K 4 x z u_1 u_{1,2} u_{2,3}^2 \\
& C 4 x z u_1 u_{1,3} u_{2,2} u_{2,3} C 4 x z u_3 u_{1,2}^2 u_{2,3} K 4 x z u_3 u_{1,2} u_{1,3} u_{2,2} \\
& C 2 x u[ ] u_1 u_{1,1} u_{2,2} u_{3,3} C 2 x u[ ] u_1 u_{1,1} u_{2,3}^2 K 2 x u[ ] u_1 u_{1,2}^2 u_{3,3} K 2 x u[ ] u_1 \\
& u_{1,3}^2 u_{2,2} K 4 u_{2,3} u_{1,2} u_{1,1} u_3 u[ ] x C 4 u_{1,3} u_{1,2}^2 u_3 u[ ] x K 2 y z u_1 u_{2,2}^2 u_{3,3} \\
& C 2 y z u_1 u_{2,2} u_{2,3}^2 C 2 y z u_2 u_{1,2} u_{2,2} u_{3,3} K 2 y z u_2 u_{1,3} u_{2,2} u_{2,3} \\
& K 2 y z u_3 u_{1,2} u_{2,2} u_{2,3} C 2 y z u_3 u_{1,3} u_{2,2}^2 C 2 y u[ ] u_1 u_{1,2} u_{2,2} u_{3,3} \\
& K 2 y u[ ] u_1 u_{1,3} u_{2,2} u_{2,3} K 2 y u[ ] u_2 u_{1,1} u_{2,3}^2 K 2 y u[ ] u_2 u_{1,2}^2 u_{3,3} \\
& C 4 y u[ ] u_2 u_{1,2} u_{1,3} u_{2,3} C 2 y u[ ] u_3 u_{1,1} u_{2,2} u_{2,3} K 2 y u[ ] u_3 u_{1,2} u_{1,3} u_{2,2} \\
& C 2 z^2 u_1 u_{2,2} u_{2,3} u_{3,3} K 2 z^2 u_1 u_{2,3}^3 K 2 z^2 u_3 u_{1,2} u_{2,2} u_{3,3} C 2 z^2 u_3 u_{1,2} u_{2,3}^2 \\
& K 4 z u[ ] u_1 u_{1,2} u_{2,3} u_{3,3} C 4 z u[ ] u_1 u_{1,3} u_{2,3}^2 C 2 z u[ ] u_3 u_{1,1} u_{2,2} u_{3,3} \\
& K 2 z u[ ] u_3 u_{1,1} u_{2,3}^2 C 2 z u[ ] u_3 u_{1,2}^2 u_{3,3} K 2 z u[ ] u_3 u_{1,3}^2 u_{2,2} \\
& C 2 u[ ]^2 u_1 u_{1,1} u_{2,3} u_{3,3} K 2 u[ ]^2 u_1 u_{1,3}^2 u_{2,3} K 2 u_{3,3} u_{1,2} u_{1,1} u_3 u[ ]^2 C 2 \\
& u_{1,3}^2 u_{1,2} u_3 u[ ]^2 C u_{2,2}^2 u_{1,1} x^2 K u_{2,2} u_{1,2}^2 x^2 K 2 x z u_{1,2} u_{2,2} u_{2,3} C 2 x z u_{1,3} u_{2,2}^2 \\
& C 2 u_{2,3} u_{2,2} u_{1,1} u[ ] x K 2 u_{2,2} u_{1,3} u_{1,2} u[ ] x C z^2 u_{2,2}^2 u_{3,3} K z^2 u_{2,2} u_{2,3}^2
\end{aligned}$$

$$\frac{\left( \frac{2}{3} u_1^2 u_2^2 u_3^2 + \frac{2}{3} u_1^2 u_2 u_3^2 + \frac{2}{3} u_1 u_2^2 u_3^2 + \frac{2}{3} u_1^2 u_2^2 u_3 \right) \left( \frac{2}{3} u_1^2 u_2^2 u_3^2 + \frac{2}{3} u_1^2 u_2 u_3^2 + \frac{2}{3} u_1 u_2^2 u_3^2 + \frac{2}{3} u_1^2 u_2^2 u_3 \right)}{\left( \frac{2}{3} u_1^2 u_2^2 u_3^2 + \frac{2}{3} u_1^2 u_2 u_3^2 + \frac{2}{3} u_1 u_2^2 u_3^2 + \frac{2}{3} u_1^2 u_2^2 u_3 \right) \left( \frac{2}{3} u_1^2 u_2^2 u_3^2 + \frac{2}{3} u_1^2 u_2 u_3^2 + \frac{2}{3} u_1 u_2^2 u_3^2 + \frac{2}{3} u_1^2 u_2^2 u_3 \right)}$$

M >

## Surfaces in 4-dimensions

M > restart with(DifferentialGeometry) : with(Tensor) : with(JetCalculus) :  
with(Tools) :

M > DGsetup([t, s], [x, y], M, 4) :

M > Preferences("JetNotation", "JetNotation1") :

M > ω d evalDG(dt &w dx[ ] C ds &w dy[ ])

$$\omega d dt Y dx[ ] C ds Y dy[ ] \quad (3.1)$$

M > v0 d evalDG(t D\_t C s D\_s C x[ ] D\_x[ ] C y[ ] D\_y[ ])

$$v0 d t D_t C s D_s C x[ ] D_x[ ] C y[ ] D_y[ ] \quad (3.2)$$

Insert a non-canonical basis on the tangent space

M > X d evalDG(D\_t C x[1] D\_x[ ] C y[1] D\_y[ ]); Y d evalDG(D\_s C x[2] D\_x[ ]  
C y[2] D\_y[ ])

$$X d D_t C x_1 D_x[ ] C y_1 D_y[ ]$$

$$Y d D_s C x_2 D_x[ ] C y_2 D_y[ ] \quad (3.3)$$

Take an arbitrary vector

M > W<sup>t</sup> d evalDG(a D\_t C b D\_s C c D\_x[ ] C d D\_y[ ])

$$W^t d a D_t C b D_s C c D_x[ ] C d D_y[ ] \quad (3.4)$$

use it to compute a basis for the orthogonal complement of T<sub>{p}</sub>M with respect to ω

M > tmp1 d solve({Hook([X, W<sup>t</sup>], ω), Hook([Y, W<sup>t</sup>], ω)}, {a, b, c, d}) :

M > Wtmp d subs(tmp1, W<sup>t</sup>) :

M > X<sup>t</sup> d DGsimplify(eval(Wtmp, {a=1, b=0})) : Y<sup>t</sup> d DGsimplify(eval(Wtmp,  
{a=0, b=1})) :

using these we can compute a canonical basis for T<sub>{p}</sub>M

M > v1 d evalDG\left(\frac{y[2] s C x[2] t K y[ ]}{x[2] K y[1]} D\_t C \left(\frac{K y[1] s K x[1] t C x[ ]}{x[2] K y[1]}\right) D\_s

$$C \left(\frac{(K y[1] s C x[ ] x[2] C x[1] (y[2] s K y[ ]))}{x[2] K y[1]}\right) D_x[ ]$$

$$C \left(\frac{(x[2] t K y[ ] y[1] K y[2] (x[1] t K x[ ]))}{x[2] K y[1]}\right) D_y[ ] \Big)$$

$$v1 d \frac{(y_2 s C x_2 t K y[ ] ) D_t}{x_2 K y_1} K \frac{(y_1 s C x_1 t K x[ ] ) D_s}{x_2 K y_1}$$

$$C \frac{(s x_1 y_2 K s x_2 y_1 C x[ ] x_2 K x_1 y[ ] ) D_x[ ]}{x_2 K y_1}$$

(3.5)

$$K \frac{(tx_1 y_2 K tx_2 y_1 K x[ ] y_2 C y[ ] y_1) D_{-y[ ]}}{x_2 K y_1}$$

$$\begin{aligned} \mathbf{M} > v2 \text{ d } evalDG \left( \left( \frac{ky[2] s K y[1] t C y[ ]}{x[2] K y[1]} \right) D_{-t} C \left( \frac{x[2] s C x[1] t K x[ ]}{x[2] K y[1]} \right) D_{-s} \right. \\ & C \left( \frac{(x[2] s K x[ ] ) y[1] K x[1] (y[2] s K y[ ] )}{x[2] K y[1]} \right) D_{-x[ ]} \\ & \left. C \left( \frac{(ky[1] t C y[ ] ) x[2] C y[2] \$ (x[1] t K x[ ] )}{x[2] K y[1]} \right) D_{-y[ ]} \right) \end{aligned}$$

$$v2 \text{ d } K \frac{(y_2 s C t y_1 K y[ ] ) D_{-t}}{x_2 K y_1} C \frac{(x_2 s C x_1 t K x[ ] ) D_{-s}}{x_2 K y_1} \quad (3.6)$$

$$K \frac{(s x_1 y_2 K s x_2 y_1 C x[ ] y_1 K x_1 y[ ] ) D_{-x[ ]}}{x_2 K y_1}$$

$$C \frac{(t x_1 y_2 K t x_2 y_1 K x[ ] y_2 C x_2 y[ ] ) D_{-y[ ]}}{x_2 K y_1}$$

Arbitrary vectors in  $T_{\{p\}\Sigma}$  and  $T_{\{p\}\Sigma}^{\dagger}$  to be determined a quadratic form expression in the basis  $d^2 f$  and  $d^2 g$

$$\mathbf{M} > w1tmp \text{ d } evalDG(k1 X C k2 Y) : w2tmp \text{ d } evalDG(l1 X^{\dagger} C l2 Y^{\dagger}) :$$

$$\mathbf{M} > H1 \text{ d } evalDG(x[1, 1] dt \& s dt C 2 x[1, 2] dt \& s ds C x[2, 2] ds \& s ds) : H2 \\ \text{ d } evalDG(y[1, 1] dt \& s dt C 2 y[1, 2] dt \& s ds C y[2, 2] ds \& s ds) :$$

$$\mathbf{M} > Q1 \text{ d } evalDG(a H1 C b H2)$$

$$Q1 \text{ d } (a x_{1,1} C b y_{1,1}) dt dt C (a x_{1,2} C b y_{1,2}) dt ds C (a x_{1,2} C b y_{1,2}) ds dt \\ C (a x_{2,2} C b y_{2,2}) ds ds \quad (3.7)$$

Fix Q1 up to scale by  $Q(v1, v1) = 0$ .

$$\mathbf{M} > tmp1 \text{ d } solve(Hook([v1, v1], Q1), \{a\}) :$$

$$\mathbf{M} > Q1 \text{ d } subs(tmp1, Q1) :$$

We can now determine w1tmp uniquely as the second null-like vector to Q1

$$\mathbf{M} > tmp2 \text{ d } solve(\{Hook([v1, w1tmp], \omega) K 1, Hook([w1tmp, w1tmp], Q1)\}, \{k1, k2\}) :$$

$$\mathbf{M} > w1 \text{ d } subs(tmp2, w1tmp) :$$

Having obtained w1 uniquely we can fix Q1

$$\mathbf{M} > tmp3 \text{ d } solve(\{Hook([v1, w1], Q1) K 1\}, \{b\}) :$$

$$\mathbf{M} > Q1 \text{ d } subs(tmp3, Q1) :$$

Next, we find the corresponding 1-form

$$\mathbf{M} > df \text{ d } evalDG(dx[ ] K x[1] dt K x[2] ds); dg \text{ d } evalDG(dy[ ] K y[1] dt K y[2] ds) \\ df \text{ d } kx_1 dt K x_2 ds C dx[ ] \\ dg \text{ d } ky_1 dt K y_2 ds C dy[ ] \quad (3.8)$$

$$\mathbf{M} > \sigma1 \text{ d } evalDG(a df C b dg)$$

$$\sigma1 \text{ d } k(a x_1 C b y_1) dt K (a x_2 C b y_2) ds C a dx[ ] C b dy[ ] \quad (3.9)$$

Recall that the 1-form corresponding to the quadratic form has the same coefficients, hence we substitute these into  $\sigma1$ , determining it uniquely.

$$\mathbf{M} > \sigma1 \text{ d } subs(tmp3, subs(tmp1, \sigma1)) :$$

Now we can compute our first invariant

$$\mathbf{M} > I_{2a} \text{ d } Hook(v2, \sigma1) :$$

To find the remaining invariants we start with the 1-form and determine its quadratic form. This again boils down to just finding the coefficients

$$\begin{aligned} \mathbf{M} > \sigma_2 \text{ d evalDG}(c \text{ df} \text{ C } d \text{ dg}) \\ \sigma_2 \text{ d } \mathbb{K}(c x_1 \text{ C } d y_1) \text{ dt } \mathbb{K}(c x_2 \text{ C } d y_2) \text{ ds } \text{ C } c \text{ dx} [ ] \text{ C } d \text{ dy} [ ] \end{aligned} \quad (3.10)$$

The vector w2tmp is not determined, so the first thing to do is find it

$$\mathbf{M} > \text{tmp4} \text{ d solve}(\{\text{Hook}([v_2, w2tmp], \omega) \mathbb{K} 1, \text{Hook}(w2tmp, \sigma_1)\}, \{l_1, l_2\}) :$$

$$\mathbf{M} > w_2 \text{ d subs}(\text{tmp4}, w2tmp) :$$

Having found w2 we can move on to obtaining  $\sigma_2$

$$\mathbf{M} > \text{tmp5} \text{ d solve}(\{\text{Hook}(w_2, \sigma_2) \mathbb{K} 1, \text{Hook}(v_2, \sigma_2)\}, \{c, d\}) :$$

These coefficients will give the quadratic form Q2 uniquely

$$\begin{aligned} \mathbf{M} > Q2\text{tmp} \text{ d evalDG}(c \text{ H1} \text{ C } d \text{ H2}) \\ Q2\text{tmp} \text{ d } (c x_{1,1} \text{ C } d y_{1,1}) \text{ dt dt} \text{ C } (c x_{1,2} \text{ C } d y_{1,2}) \text{ dt ds} \text{ C } (c x_{1,2} \text{ C } d y_{1,2}) \text{ ds dt} \\ \text{ C } (c x_{2,2} \text{ C } d y_{2,2}) \text{ ds ds} \end{aligned} \quad (3.11)$$

$$\mathbf{M} > Q_2 \text{ d subs}(\text{tmp5}, Q2\text{tmp}) :$$

the remaining invariants are then computed as

$$\mathbf{M} > I_{2b} \text{ d Hook}([v_1, v_1], Q_2) \\ I_{2b} \text{ d } \frac{1}{(x_2 \mathbb{K} y_1)^3} (s^3 x_2 y_1^2 y_{2,2} \mathbb{K} 2 s^3 x_2 y_1 y_2 y_{1,2} \text{ C } s^3 x_2 y_2^2 y_{1,1} \mathbb{K} s^3 x_{1,1} y_2^3 \text{ C } 2 s^3 x_{1,2} y_1 \quad (3.12)$$

$$\begin{aligned} & y_2^2 \mathbb{K} s^3 x_{2,2} y_1^2 y_2 \text{ C } 2 s^2 t x_1 x_2 y_1 y_{2,2} \mathbb{K} 2 s^2 t x_1 x_2 y_2 y_{1,2} \text{ C } 2 s^2 t x_1 x_{1,2} y_2^2 \\ & \mathbb{K} 2 s^2 t x_1 x_{2,2} y_1 y_2 \text{ C } s^2 t x_1 y_1^2 y_{2,2} \mathbb{K} 2 s^2 t x_1 y_1 y_2 y_{1,2} \text{ C } s^2 t x_1 y_2^2 y_{1,1} \mathbb{K} 2 s^2 t \\ & x_2^2 y_1 y_{1,2} \text{ C } 2 s^2 t x_2^2 y_2 y_{1,1} \mathbb{K} 2 s^2 t x_2 x_{1,1} y_2^2 \text{ C } 2 s^2 t x_2 x_{1,2} y_1 y_2 \mathbb{K} s^2 t x_{1,1} y_1 y_2^2 \\ & \text{ C } 2 s^2 t x_{1,2} y_1^2 y_2 \mathbb{K} s^2 t x_{2,2} y_1^3 \text{ C } s^2 t x_1^2 x_2 y_{2,2} \mathbb{K} s^2 t x_1^2 x_{2,2} y_2 \text{ C } 2 s^2 t x_1^2 y_1 y_{2,2} \\ & \mathbb{K} 2 s^2 t x_1^2 y_2 y_{1,2} \mathbb{K} 2 s^2 t x_1 x_2^2 y_{1,2} \text{ C } 2 s^2 t x_1 x_2 x_{1,2} y_2 \mathbb{K} 2 s^2 t x_1 x_2 y_1 y_{1,2} \\ & \text{ C } 2 s^2 t x_1 x_2 y_2 y_{1,1} \text{ C } 2 s^2 t x_1 x_{1,2} y_1 y_2 \mathbb{K} 2 s^2 t x_1 x_{2,2} y_1^2 \text{ C } s^2 t x_2^3 y_{1,1} \mathbb{K} s^2 t x_2^2 x_{1,1} y_2 \\ & \mathbb{K} 2 s^2 t x_2 x_{1,1} y_1 y_2 \text{ C } 2 s^2 t x_2 x_{1,2} y_1^2 \text{ C } t^3 x_1^3 y_{2,2} \mathbb{K} 2 t^3 x_1^2 x_2 y_{1,2} \mathbb{K} t^3 x_1^2 x_{2,2} y_1 \text{ C } t^3 x_1 \\ & x_2^2 y_{1,1} \text{ C } 2 t^3 x_1 x_2 x_{1,2} y_1 \mathbb{K} t^3 x_2^2 x_{1,1} y_1 \mathbb{K} 2 s^2 x [ ] x_2 y_1 y_{2,2} \text{ C } 2 s^2 x [ ] x_2 y_2 y_{1,2} \\ & \mathbb{K} 2 s^2 x [ ] x_{1,2} y_2^2 \text{ C } 2 s^2 x [ ] x_{2,2} y_1 y_2 \mathbb{K} s^2 x [ ] y_1^2 y_{2,2} \text{ C } 2 s^2 x [ ] y_1 y_2 y_{1,2} \mathbb{K} s^2 x [ ] \\ & y_2^2 y_{1,1} \text{ C } 2 s^2 x_2 y [ ] y_1 y_{1,2} \mathbb{K} 2 s^2 x_2 y [ ] y_2 y_{1,1} \text{ C } 3 s^2 x_{1,1} y [ ] y_2^2 \mathbb{K} 4 s^2 x_{1,2} y [ ] y_1 y_2 \\ & \text{ C } s^2 x_{2,2} y [ ] y_1^2 \mathbb{K} 2 s t x [ ] x_1 x_2 y_{2,2} \text{ C } 2 s t x [ ] x_1 x_{2,2} y_2 \mathbb{K} 4 s t x [ ] x_1 y_1 y_{2,2} \\ & \text{ C } 4 s t x [ ] x_1 y_2 y_{1,2} \text{ C } 2 s t x [ ] x_2^2 y_{1,2} \mathbb{K} 2 s t x [ ] x_2 x_{1,2} y_2 \text{ C } 2 s t x [ ] x_2 y_1 y_{1,2} \\ & \mathbb{K} 2 s t x [ ] x_2 y_2 y_{1,1} \mathbb{K} 2 s t x [ ] x_{1,2} y_1 y_2 \text{ C } 2 s t x [ ] x_{2,2} y_1^2 \text{ C } 2 s t x_1 x_2 y [ ] y_{1,2} \\ & \mathbb{K} 4 s t x_1 x_{1,2} y [ ] y_2 \text{ C } 2 s t x_1 x_{2,2} y [ ] y_1 \text{ C } 2 s t x_1 y [ ] y_1 y_{1,2} \mathbb{K} 2 s t x_1 y [ ] y_2 y_{1,1} \\ & \mathbb{K} 2 s t x_2^2 y [ ] y_{1,1} \text{ C } 4 s t x_2 x_{1,1} y [ ] y_2 \mathbb{K} 2 s t x_2 x_{1,2} y [ ] y_1 \text{ C } 2 s t x_{1,1} y [ ] y_1 y_2 \\ & \mathbb{K} 2 s t x_{1,2} y [ ] y_1^2 \mathbb{K} 3 t^2 x [ ] x_1^2 y_{2,2} \text{ C } 4 t^2 x [ ] x_1 x_2 y_{1,2} \text{ C } 2 t^2 x [ ] x_1 x_{2,2} y_1 \mathbb{K} t^2 x [ ] \\ & x_2^2 y_{1,1} \mathbb{K} 2 t^2 x [ ] x_2 x_{1,2} y_1 \text{ C } t^2 x_1^2 x_{2,2} y [ ] \text{ C } 2 t^2 x_1^2 y [ ] y_{1,2} \mathbb{K} 2 t^2 x_1 x_2 x_{1,2} y [ ] \\ & \mathbb{K} 2 t^2 x_1 x_2 y [ ] y_{1,1} \mathbb{K} 2 t^2 x_1 x_{1,2} y [ ] y_1 \text{ C } t^2 x_2^2 x_{1,1} y [ ] \text{ C } 2 t^2 x_2 x_{1,1} y [ ] y_1 \end{aligned}$$

$$\begin{aligned}
& C s x [ ]^2 x_2 y_2, 2 K s x [ ]^2 x_2, 2 y_2 C 2 s x [ ]^2 y_1 y_2, 2 K 2 s x [ ]^2 y_2 y_1, 2 \\
& K 2 s x [ ] x_2 y [ ] y_1, 2 C 4 s x [ ] x_1, 2 y [ ] y_2 K 2 s x [ ] x_2, 2 y [ ] y_1 K 2 s x [ ] y [ ] y_1 y_1, 2 \\
& C 2 s x [ ] y [ ] y_2 y_1, 1 C s x_2 y [ ]^2 y_1, 1 K 3 s x_{1, 1} y [ ]^2 y_2 C 2 s x_{1, 2} y [ ]^2 y_1 \\
& C 3 t x [ ]^2 x_1 y_2, 2 K 2 t x [ ]^2 x_2 y_1, 2 K t x [ ]^2 x_2, 2 y_1 K 2 t x [ ] x_1 x_2, 2 y [ ] \\
& K 4 t x [ ] x_1 y [ ] y_1, 2 C 2 t x [ ] x_2 x_1, 2 y [ ] C 2 t x [ ] x_2 y [ ] y_1, 1 C 2 t x [ ] x_1, 2 y [ ] y_1 \\
& C 2 t x_1 x_1, 2 y [ ]^2 C t x_1 y [ ]^2 y_1, 1 K 2 t x_2 x_1, 1 y [ ]^2 K t x_{1, 1} y [ ]^2 y_1 K x [ ]^3 y_2, 2 \\
& C x [ ]^2 x_2, 2 y [ ] C 2 x [ ]^2 y [ ] y_1, 2 K 2 x [ ] x_1, 2 y [ ]^2 K x [ ] y [ ]^2 y_1, 1 C x_{1, 1} y [ ]^3
\end{aligned}$$

**M** >  $I_{2c} \triangleleft \text{Hook}([v1, w1], Q2)$

$$\begin{aligned}
I_{2c} \triangleleft K ( & s^3 x_2 x_{1, 1} y_1^2 y_2^2, 2 K 2 s^3 x_2 x_{1, 1} y_1 y_2 y_1, 2 y_2, 2 K s^3 x_2 x_{1, 1} y_2^2 y_1, 1 y_2, 2 C 2 s^3 x_2 x_{1, 1} y_2^2 y_1^2, 2 \\
& K 2 s^3 x_2 x_{1, 2} y_1^2 y_1, 2 y_2, 2 C 4 s^3 x_2 x_{1, 2} y_1 y_2 y_1, 1 y_2, 2 K 2 s^3 x_2 x_{1, 2} y_2^2 y_1, 1 y_1, 2 \\
& K s^3 x_2 x_{2, 2} y_1^2 y_1, 1 y_2, 2 C 2 s^3 x_2 x_{2, 2} y_1^2 y_2^2, 2 K 2 s^3 x_2 x_{2, 2} y_1 y_2 y_1, 1 y_1, 2 C s^3 x_2 x_{2, 2} y_2^2 \\
& y_1^2, 1 C s^3 x_1^2, 1 y_2^3 y_2, 2 K 2 s^3 x_{1, 1} x_{1, 2} y_1 y_2^2 y_2, 2 K 2 s^3 x_{1, 1} x_{1, 2} y_2^3 y_1, 2 K s^3 x_{1, 1} x_{2, 2} \\
& y_1^2 y_2 y_2, 2 C 4 s^3 x_{1, 1} x_{2, 2} y_1 y_2^2 y_1, 2 K s^3 x_{1, 1} x_{2, 2} y_2^3 y_1, 1 C 2 s^3 x_{1, 2}^2 y_1^2 y_2 y_2, 2 C 2 s^3 x_{1, 2}^2 \\
& y_2^3 y_1, 1 K 2 s^3 x_{1, 2} x_{2, 2} y_1^2 y_2 y_1, 2 K 2 s^3 x_{1, 2} x_{2, 2} y_1 y_2^2 y_1, 1 C s^3 x_{2, 2}^2 y_1^2 y_2 y_1, 1 \\
& C 2 s^2 t x_1 x_2 x_{1, 1} y_1 y_2^2, 2 K 2 s^2 t x_1 x_2 x_{1, 1} y_2 y_1, 2 y_2, 2 K 4 s^2 t x_1 x_2 x_{1, 2} y_1 y_1, 2 y_2, 2 \\
& C 4 s^2 t x_1 x_2 x_{1, 2} y_2 y_1, 1 y_2, 2 K 2 s^2 t x_1 x_2 x_{2, 2} y_1 y_1, 1 y_2, 2 C 4 s^2 t x_1 x_2 x_{2, 2} y_1 y_1^2, 2 \\
& K 2 s^2 t x_1 x_2 x_{2, 2} y_2 y_1, 1 y_1, 2 K 2 s^2 t x_1 x_{1, 1} x_{1, 2} y_2^2 y_2, 2 K 2 s^2 t x_1 x_{1, 1} x_{2, 2} y_1 y_2 y_2, 2 \\
& C 4 s^2 t x_1 x_{1, 1} x_{2, 2} y_2^2 y_1, 2 C s^2 t x_1 x_{1, 1} y_1^2 y_2^2, 2 K 2 s^2 t x_1 x_{1, 1} y_1 y_2 y_1, 2 y_2, 2 \\
& K s^2 t x_1 x_{1, 1} y_2^2 y_1, 1 y_2, 2 C 2 s^2 t x_1 x_{1, 1} y_2^2 y_1^2, 2 C 4 s^2 t x_1 x_{1, 2}^2 y_1 y_2 y_2, 2 \\
& K 4 s^2 t x_1 x_{1, 2} x_{2, 2} y_1 y_2 y_1, 2 K 2 s^2 t x_1 x_{1, 2} x_{2, 2} y_2^2 y_1, 1 K 2 s^2 t x_1 x_{1, 2} y_1^2 y_1, 2 y_2, 2 \\
& C 4 s^2 t x_1 x_{1, 2} y_1 y_2 y_1, 1 y_2, 2 K 2 s^2 t x_1 x_{1, 2} y_2^2 y_1, 1 y_1, 2 C 2 s^2 t x_1 x_{2, 2}^2 y_1 y_2 y_1, 1 \\
& K s^2 t x_1 x_{2, 2} y_1^2 y_1, 1 y_2, 2 C 2 s^2 t x_1 x_{2, 2} y_1^2 y_2^2, 2 K 2 s^2 t x_1 x_{2, 2} y_1 y_2 y_1, 1 y_1, 2 \\
& C s^2 t x_1 x_{2, 2} y_2^2 y_1^2, 1 K 2 s^2 t x_2^2 x_{1, 1} y_1 y_1, 2 y_2, 2 K 2 s^2 t x_2^2 x_{1, 1} y_2 y_1, 1 y_2, 2 C 4 s^2 t \\
& x_2^2 x_{1, 1} y_2 y_1^2, 2 C 4 s^2 t x_2^2 x_{1, 2} y_1 y_1, 1 y_2, 2 K 4 s^2 t x_2^2 x_{1, 2} y_2 y_1, 1 y_1, 2 K 2 s^2 t \\
& x_2^2 x_{2, 2} y_1 y_1, 1 y_1, 2 C 2 s^2 t x_2^2 x_{2, 2} y_2 y_1^2, 1 C 2 s^2 t x_2 x_{1, 1}^2 y_2^2 y_2, 2 \\
& K 2 s^2 t x_2 x_{1, 1} x_{1, 2} y_1 y_2 y_2, 2 K 4 s^2 t x_2 x_{1, 1} x_{1, 2} y_2^2 y_1, 2 C 4 s^2 t x_2 x_{1, 1} x_{2, 2} y_1 y_2 y_1, 2 \\
& K 2 s^2 t x_2 x_{1, 1} x_{2, 2} y_2^2 y_1, 1 C 4 s^2 t x_2 x_{1, 2}^2 y_2^2 y_1, 1 K 2 s^2 t x_2 x_{1, 2} x_{2, 2} y_1 y_2 y_1, 1 C s^2 t \\
& x_{1, 1} y_1 y_2^2 y_2, 2 K 2 s^2 t x_{1, 1} x_{1, 2} y_1^2 y_2 y_2, 2 K 2 s^2 t x_{1, 1} x_{1, 2} y_1 y_2^2 y_1, 2 K s^2 t x_{1, 1} x_{2, 2} \\
& y_1^3 y_2, 2 C 4 s^2 t x_{1, 1} x_{2, 2} y_1^2 y_2 y_1, 2 K s^2 t x_{1, 1} x_{2, 2} y_1 y_2^2 y_1, 1 C 2 s^2 t x_{1, 2}^2 y_1^3 y_2, 2 C 2 s^2 t \\
& x_{1, 2}^2 y_1 y_2^2 y_1, 1 K 2 s^2 t x_{1, 2} x_{2, 2} y_1^3 y_1, 2 K 2 s^2 t x_{1, 2} x_{2, 2} y_1^2 y_2 y_1, 1 C s^2 t x_{2, 2}^2 y_1^3 y_1, 1 \\
& C s t^2 x_1^2 x_2 x_{1, 1} y_2^2, 2 K 2 s t^2 x_1^2 x_2 x_{1, 2} y_1, 2 y_2, 2 K s t^2 x_1^2 x_2 x_{2, 2} y_1, 1 y_2, 2 C 2 s t^2 \\
& x_1^2 x_2 x_{2, 2} y_1^2, 2 K s t^2 x_1^2 x_{1, 1} x_{2, 2} y_2 y_2, 2 C 2 s t^2 x_1^2 x_{1, 1} y_1 y_2^2, 2 K 2 s t^2 x_1^2 x_{1, 1} y_2 y_1, 2 y_2, 2
\end{aligned}
\tag{3.13}$$

$$\begin{aligned}
& C 2 s^2 x_1^2 x_{1,2}^2 y_2 y_{2,2} K 2 s^2 x_1^2 x_{1,2} x_{2,2} y_2 y_{1,2} K 4 s^2 x_1^2 x_{1,2} y_1 y_{1,2} y_{2,2} C 4 s^2 \\
& x_1^2 x_{1,2} y_2 y_{1,1} y_{2,2} C s^2 x_1^2 x_{2,2}^2 y_2 y_{1,1} K 2 s^2 x_1^2 x_{2,2} y_1 y_{1,1} y_{2,2} C 4 s^2 x_1^2 x_{2,2} y_1 y_{1,2}^2 \\
& K 2 s^2 x_1^2 x_{2,2} y_2 y_{1,1} y_{1,2} K 2 s^2 x_1 x_2^2 x_{1,1} y_{1,2} y_{2,2} C 4 s^2 x_1 x_2^2 x_{1,2} y_{1,1} y_{2,2} \\
& K 2 s^2 x_1 x_2^2 x_{2,2} y_{1,1} y_{1,2} K 2 s^2 x_1 x_2 x_{1,1} x_{1,2} y_2 y_{2,2} C 4 s^2 x_1 x_2 x_{1,1} x_{2,2} y_2 y_{1,2} \\
& K 2 s^2 x_1 x_2 x_{1,1} y_1 y_{1,2} y_{2,2} K 2 s^2 x_1 x_2 x_{1,1} y_2 y_{1,1} y_{2,2} C 4 s^2 x_1 x_2 x_{1,1} y_2 y_{1,2}^2 \\
& K 2 s^2 x_1 x_2 x_{1,2} x_{2,2} y_2 y_{1,1} C 4 s^2 x_1 x_2 x_{1,2} y_1 y_{1,1} y_{2,2} K 4 s^2 x_1 x_2 x_{1,2} y_2 y_{1,1} y_{1,2} \\
& K 2 s^2 x_1 x_2 x_{2,2} y_1 y_{1,1} y_{1,2} C 2 s^2 x_1 x_2 x_{2,2} y_2 y_{1,1}^2 K 2 s^2 x_1 x_{1,1} x_{1,2} y_1 y_2 y_{2,2} \\
& K 2 s^2 x_1 x_{1,1} x_{2,2} y_1^2 y_{2,2} C 4 s^2 x_1 x_{1,1} x_{2,2} y_1 y_2 y_{1,2} C 4 s^2 x_1 x_{1,2}^2 y_1^2 y_{2,2} \\
& K 4 s^2 x_1 x_{1,2} x_{2,2} y_1^2 y_{1,2} K 2 s^2 x_1 x_{1,2} x_{2,2} y_1 y_2 y_{1,1} C 2 s^2 x_1 x_{2,2}^2 y_1^2 y_{1,1} K s^2 \\
& x_2^3 x_{1,1} y_{1,1} y_{2,2} C 2 s^2 x_2^3 x_{1,1} y_{1,2}^2 K 2 s^2 x_2^3 x_{1,2} y_{1,1} y_{1,2} C s^2 x_2^3 x_{2,2} y_{1,1}^2 C s^2 x_2^2 \\
& x_{1,1}^2 y_2 y_{2,2} K 2 s^2 x_2^2 x_{1,1} x_{1,2} y_2 y_{1,2} K s^2 x_2^2 x_{1,1} x_{2,2} y_2 y_{1,1} C 2 s^2 x_2^2 x_{1,2}^2 y_2 y_{1,1} \\
& C 2 s^2 x_2 x_{1,1}^2 y_1 y_2 y_{2,2} K 2 s^2 x_2 x_{1,1} x_{1,2} y_1^2 y_{2,2} K 4 s^2 x_2 x_{1,1} x_{1,2} y_1 y_2 y_{1,2} \\
& C 4 s^2 x_2 x_{1,1} x_{2,2} y_1^2 y_{1,2} K 2 s^2 x_2 x_{1,1} x_{2,2} y_1 y_2 y_{1,1} C 4 s^2 x_2 x_{1,2}^2 y_1 y_2 y_{1,1} \\
& K 2 s^2 x_2 x_{1,2} x_{2,2} y_1^2 y_{1,1} C t^3 x_1^3 x_{1,1} y_{2,2}^2 K 2 t^3 x_1^3 x_{1,2} y_{1,2} y_{2,2} K t^3 x_1^3 x_{2,2} y_{1,1} y_{2,2} \\
& C 2 t^3 x_1^3 x_{2,2} y_{1,2}^2 K 2 t^3 x_1^2 x_2 x_{1,1} y_{1,2} y_{2,2} C 4 t^3 x_1^2 x_2 x_{1,2} y_{1,1} y_{2,2} K 2 t^3 \\
& x_1^2 x_2 x_{2,2} y_{1,1} y_{1,2} K t^3 x_1^2 x_{1,1} x_{2,2} y_1 y_{2,2} C 2 t^3 x_1^2 x_{1,2}^2 y_1 y_{2,2} K 2 t^3 x_1^2 x_{1,2} x_{2,2} y_1 y_{1,2} \\
& C t^3 x_1^2 x_{2,2}^2 y_1 y_{1,1} K t^3 x_1 x_2^2 x_{1,1} y_{1,1} y_{2,2} C 2 t^3 x_1 x_2^2 x_{1,1} y_{1,2}^2 K 2 t^3 x_1 x_2^2 x_{1,2} y_{1,1} y_{1,2} \\
& C t^3 x_1 x_2^2 x_{2,2} y_{1,1}^2 K 2 t^3 x_1 x_2 x_{1,1} x_{1,2} y_1 y_{2,2} C 4 t^3 x_1 x_2 x_{1,1} x_{2,2} y_1 y_{1,2} \\
& K 2 t^3 x_1 x_2 x_{1,2} x_{2,2} y_1 y_{1,1} C t^3 x_2^2 x_{1,1}^2 y_1 y_{2,2} K 2 t^3 x_2^2 x_{1,1} x_{1,2} y_1 y_{1,2} K t^3 \\
& x_2^2 x_{1,1} x_{2,2} y_1 y_{1,1} C 2 t^3 x_2^2 x_{1,2}^2 y_1 y_{1,1} K 2 s^2 x[ ] x_2 x_{1,1} y_1 y_{2,2}^2 \\
& C 2 s^2 x[ ] x_2 x_{1,1} y_2 y_{1,2} y_{2,2} C 4 s^2 x[ ] x_2 x_{1,2} y_1 y_{1,2} y_{2,2} \\
& K 4 s^2 x[ ] x_2 x_{1,2} y_2 y_{1,1} y_{2,2} C 2 s^2 x[ ] x_2 x_{2,2} y_1 y_{1,1} y_{2,2} K 4 s^2 x[ ] x_2 x_{2,2} y_1 y_{1,2}^2 \\
& C 2 s^2 x[ ] x_2 x_{2,2} y_2 y_{1,1} y_{1,2} C 2 s^2 x[ ] x_{1,1} x_{1,2} y_2^2 y_{2,2} C 2 s^2 x[ ] x_{1,1} x_{2,2} y_1 y_2 y_{2,2} \\
& K 4 s^2 x[ ] x_{1,1} x_{2,2} y_2^2 y_{1,2} K s^2 x[ ] x_{1,1} y_1^2 y_{2,2}^2 C 2 s^2 x[ ] x_{1,1} y_1 y_2 y_{1,2} y_{2,2} \\
& C s^2 x[ ] x_{1,1} y_2^2 y_{1,1} y_{2,2} K 2 s^2 x[ ] x_{1,1} y_2^2 y_{1,2}^2 K 4 s^2 x[ ] x_{1,2}^2 y_1 y_2 y_{2,2} \\
& C 4 s^2 x[ ] x_{1,2} x_{2,2} y_1 y_2 y_{1,2} C 2 s^2 x[ ] x_{1,2} x_{2,2} y_2^2 y_{1,1} C 2 s^2 x[ ] x_{1,2} y_1^2 y_{1,2} y_{2,2} \\
& K 4 s^2 x[ ] x_{1,2} y_1 y_2 y_{1,1} y_{2,2} C 2 s^2 x[ ] x_{1,2} y_2^2 y_{1,1} y_{1,2} K 2 s^2 x[ ] x_{2,2}^2 y_1 y_2 y_{1,1} \\
& C s^2 x[ ] x_{2,2} y_1^2 y_{1,1} y_{2,2} K 2 s^2 x[ ] x_{2,2} y_1^2 y_{1,2}^2 C 2 s^2 x[ ] x_{2,2} y_1 y_2 y_{1,1} y_{1,2} \\
& K s^2 x[ ] x_{2,2} y_2^2 y_{1,1}^2 C 2 s^2 x_2 x_{1,1} y[ ] y_1 y_{1,2} y_{2,2} C 2 s^2 x_2 x_{1,1} y[ ] y_2 y_{1,1} y_{2,2} \\
& K 4 s^2 x_2 x_{1,1} y[ ] y_2 y_{1,2}^2 K 4 s^2 x_2 x_{1,2} y[ ] y_1 y_{1,1} y_{2,2} C 4 s^2 x_2 x_{1,2} y[ ] y_2 y_{1,1} y_{1,2} \\
& C 2 s^2 x_2 x_{2,2} y[ ] y_1 y_{1,1} y_{1,2} K 2 s^2 x_2 x_{2,2} y[ ] y_2 y_{1,1}^2 K 3 s^2 x_{1,1}^2 y[ ] y_2^2 y_{2,2} \\
& C 4 s^2 x_{1,1} x_{1,2} y[ ] y_1 y_2 y_{2,2} C 6 s^2 x_{1,1} x_{1,2} y[ ] y_2^2 y_{1,2} C s^2 x_{1,1} x_{2,2} y[ ] y_1^2 y_{2,2}
\end{aligned}$$

$$\begin{aligned}
& K 8 s^2 x_{1,1} x_{2,2} y [ ] y_1 y_2 y_{1,2} C 3 s^2 x_{1,1} x_{2,2} y [ ] y_2^2 y_{1,1} K 2 s^2 x_{1,2}^2 y [ ] y_1^2 y_{2,2} K 6 s^2 \\
& x_{1,2}^2 y [ ] y_2^2 y_{1,1} C 2 s^2 x_{1,2} x_{2,2} y [ ] y_1^2 y_{1,2} C 4 s^2 x_{1,2} x_{2,2} y [ ] y_1 y_2 y_{1,1} K s^2 x_{2,2}^2 y [ ] \\
& y_1^2 y_{1,1} K 2 s t x [ ] x_1 x_2 x_{1,1} y_{2,2}^2 C 4 s t x [ ] x_1 x_2 x_{1,2} y_{1,2} y_{2,2} \\
& C 2 s t x [ ] x_1 x_2 x_{2,2} y_{1,1} y_{2,2} K 4 s t x [ ] x_1 x_2 x_{2,2} y_{1,2}^2 C 2 s t x [ ] x_1 x_{1,1} x_{2,2} y_2 y_{2,2} \\
& K 4 s t x [ ] x_1 x_{1,1} y_1 y_{2,2}^2 C 4 s t x [ ] x_1 x_{1,1} y_2 y_{1,2} y_{2,2} K 4 s t x [ ] x_1 x_{1,2}^2 y_2 y_{2,2} \\
& C 4 s t x [ ] x_1 x_{1,2} x_{2,2} y_2 y_{1,2} C 8 s t x [ ] x_1 x_{1,2} y_1 y_{1,2} y_{2,2} \\
& K 8 s t x [ ] x_1 x_{1,2} y_2 y_{1,1} y_{2,2} K 2 s t x [ ] x_1 x_{2,2}^2 y_2 y_{1,1} C 4 s t x [ ] x_1 x_{2,2} y_1 y_{1,1} y_{2,2} \\
& K 8 s t x [ ] x_1 x_{2,2} y_1 y_{1,2}^2 C 4 s t x [ ] x_1 x_{2,2} y_2 y_{1,1} y_{1,2} C 2 s t x [ ] x_2^2 x_{1,1} y_{1,2} y_{2,2} \\
& K 4 s t x [ ] x_2^2 x_{1,2} y_{1,1} y_{2,2} C 2 s t x [ ] x_2^2 x_{2,2} y_{1,1} y_{1,2} C 2 s t x [ ] x_2 x_{1,1} x_{1,2} y_2 y_{2,2} \\
& K 4 s t x [ ] x_2 x_{1,1} x_{2,2} y_2 y_{1,2} C 2 s t x [ ] x_2 x_{1,1} y_1 y_{1,2} y_{2,2} \\
& C 2 s t x [ ] x_2 x_{1,1} y_2 y_{1,1} y_{2,2} K 4 s t x [ ] x_2 x_{1,1} y_2 y_{1,2}^2 C 2 s t x [ ] x_2 x_{1,2} x_{2,2} y_2 y_{1,1} \\
& K 4 s t x [ ] x_2 x_{1,2} y_1 y_{1,1} y_{2,2} C 4 s t x [ ] x_2 x_{1,2} y_2 y_{1,1} y_{1,2} \\
& C 2 s t x [ ] x_2 x_{2,2} y_1 y_{1,1} y_{1,2} K 2 s t x [ ] x_2 x_{2,2} y_2 y_{1,1}^2 C 2 s t x [ ] x_{1,1} x_{1,2} y_1 y_2 y_{2,2} \\
& C 2 s t x [ ] x_{1,1} x_{2,2} y_1^2 y_{2,2} K 4 s t x [ ] x_{1,1} x_{2,2} y_1 y_2 y_{1,2} K 4 s t x [ ] x_{1,2}^2 y_1^2 y_{2,2} \\
& C 4 s t x [ ] x_{1,2} x_{2,2} y_1^2 y_{1,2} C 2 s t x [ ] x_{1,2} x_{2,2} y_1 y_2 y_{1,1} K 2 s t x [ ] x_{2,2}^2 y_1^2 y_{1,1} \\
& C 2 s t x_1 x_2 x_{1,1} y [ ] y_{1,2} y_{2,2} K 4 s t x_1 x_2 x_{1,2} y [ ] y_{1,1} y_{2,2} \\
& C 2 s t x_1 x_2 x_{2,2} y [ ] y_{1,1} y_{1,2} C 4 s t x_1 x_{1,1} x_{1,2} y [ ] y_2 y_{2,2} \\
& C 2 s t x_1 x_{1,1} x_{2,2} y [ ] y_1 y_{2,2} K 8 s t x_1 x_{1,1} x_{2,2} y [ ] y_2 y_{1,2} \\
& C 2 s t x_1 x_{1,1} y [ ] y_1 y_{1,2} y_{2,2} C 2 s t x_1 x_{1,1} y [ ] y_2 y_{1,1} y_{2,2} K 4 s t x_1 x_{1,1} y [ ] y_2 y_{1,2}^2 \\
& K 4 s t x_1 x_{1,2}^2 y [ ] y_1 y_{2,2} C 4 s t x_1 x_{1,2} x_{2,2} y [ ] y_1 y_{1,2} C 4 s t x_1 x_{1,2} x_{2,2} y [ ] y_2 y_{1,1} \\
& K 4 s t x_1 x_{1,2} y [ ] y_1 y_{1,1} y_{2,2} C 4 s t x_1 x_{1,2} y [ ] y_2 y_{1,1} y_{1,2} K 2 s t x_1 x_{2,2}^2 y [ ] y_1 y_{1,1} \\
& C 2 s t x_1 x_{2,2} y [ ] y_1 y_{1,1} y_{1,2} K 2 s t x_1 x_{2,2} y [ ] y_2 y_{1,1}^2 C 2 s t x_2^2 x_{1,1} y [ ] y_{1,1} y_{2,2} \\
& K 4 s t x_2^2 x_{1,1} y [ ] y_1^2 y_{2,2} C 4 s t x_2^2 x_{1,2} y [ ] y_{1,1} y_{1,2} K 2 s t x_2^2 x_{2,2} y [ ] y_{1,1}^2 K 4 s t x_2 \\
& x_{1,1}^2 y [ ] y_2 y_{2,2} C 2 s t x_2 x_{1,1} x_{1,2} y [ ] y_1 y_{2,2} C 8 s t x_2 x_{1,1} x_{1,2} y [ ] y_2 y_{1,2} \\
& K 4 s t x_2 x_{1,1} x_{2,2} y [ ] y_1 y_{1,2} C 4 s t x_2 x_{1,1} x_{2,2} y [ ] y_2 y_{1,1} K 8 s t x_2 x_{1,2}^2 y [ ] y_2 y_{1,1} \\
& C 2 s t x_2 x_{1,2} x_{2,2} y [ ] y_1 y_{1,1} K 2 s t x_{1,1}^2 y [ ] y_1 y_2 y_{2,2} C 2 s t x_{1,1} x_{1,2} y [ ] y_1^2 y_{2,2} \\
& C 4 s t x_{1,1} x_{1,2} y [ ] y_1 y_2 y_{1,2} K 4 s t x_{1,1} x_{2,2} y [ ] y_1^2 y_{1,2} \\
& C 2 s t x_{1,1} x_{2,2} y [ ] y_1 y_2 y_{1,1} K 4 s t x_{1,2}^2 y [ ] y_1 y_2 y_{1,1} C 2 s t x_{1,2} x_{2,2} y [ ] y_1^2 y_{1,1} \\
& K 3 t^2 x [ ] x_1^2 x_{1,1} y_{2,2}^2 C 6 t^2 x [ ] x_1^2 x_{1,2} y_{1,2} y_{2,2} C 3 t^2 x [ ] x_1^2 x_{2,2} y_{1,1} y_{2,2} \\
& K 6 t^2 x [ ] x_1^2 x_{2,2} y_{1,2}^2 C 4 t^2 x [ ] x_1 x_2 x_{1,1} y_{1,2} y_{2,2} K 8 t^2 x [ ] x_1 x_2 x_{1,2} y_{1,1} y_{2,2} \\
& C 4 t^2 x [ ] x_1 x_2 x_{2,2} y_{1,1} y_{1,2} C 2 t^2 x [ ] x_1 x_{1,1} x_{2,2} y_1 y_{2,2} K 4 t^2 x [ ] x_1 x_{1,2}^2 y_1 y_{2,2} \\
& C 4 t^2 x [ ] x_1 x_{1,2} x_{2,2} y_1 y_{1,2} K 2 t^2 x [ ] x_1 x_{2,2}^2 y_1 y_{1,1} C t^2 x [ ] x_2^2 x_{1,1} y_{1,1} y_{2,2}
\end{aligned}$$

$$\begin{aligned}
& K 2 t^2 x [ ] x_2^2 x_{1,1} y_{1,2}^2 C 2 t^2 x [ ] x_2^2 x_{1,2} y_{1,1} y_{1,2} K t^2 x [ ] x_2^2 x_{2,2} y_{1,1}^2 \\
& C 2 t^2 x [ ] x_2 x_{1,1} x_{1,2} y_1 y_{2,2} K 4 t^2 x [ ] x_2 x_{1,1} x_{2,2} y_1 y_{1,2} \\
& C 2 t^2 x [ ] x_2 x_{1,2} x_{2,2} y_1 y_{1,1} C t^2 x_1^2 x_{1,1} x_{2,2} y [ ] y_{2,2} C 2 t^2 x_1^2 x_{1,1} y [ ] y_{1,2} y_{2,2} \\
& K 2 t^2 x_1^2 x_{1,2} y [ ] y_{2,2} C 2 t^2 x_1^2 x_{1,2} x_{2,2} y [ ] y_{1,2} K 4 t^2 x_1^2 x_{1,2} y [ ] y_{1,1} y_{2,2} K t^2 x_1^2 \\
& x_{2,2} y [ ] y_{1,1} C 2 t^2 x_1^2 x_{2,2} y [ ] y_{1,1} y_{1,2} C 2 t^2 x_1 x_2 x_{1,1} x_{1,2} y [ ] y_{2,2} \\
& K 4 t^2 x_1 x_2 x_{1,1} x_{2,2} y [ ] y_{1,2} C 2 t^2 x_1 x_2 x_{1,1} y [ ] y_{1,1} y_{2,2} K 4 t^2 x_1 x_2 x_{1,1} y [ ] y_{1,1}^2 \\
& C 2 t^2 x_1 x_2 x_{1,2} x_{2,2} y [ ] y_{1,1} C 4 t^2 x_1 x_2 x_{1,2} y [ ] y_{1,1} y_{1,2} K 2 t^2 x_1 x_2 x_{2,2} y [ ] y_{1,1}^2 \\
& C 2 t^2 x_1 x_{1,1} x_{1,2} y [ ] y_1 y_{2,2} K 4 t^2 x_1 x_{1,1} x_{2,2} y [ ] y_1 y_{1,2} \\
& C 2 t^2 x_1 x_{1,2} x_{2,2} y [ ] y_1 y_{1,1} K t^2 x_2^2 x_{1,1} y [ ] y_{2,2} C 2 t^2 x_2^2 x_{1,1} x_{1,2} y [ ] y_{1,2} C t^2 \\
& x_2^2 x_{1,1} x_{2,2} y [ ] y_{1,1} K 2 t^2 x_2^2 x_{1,2} y [ ] y_{1,1} K 2 t^2 x_2 x_{1,1} y [ ] y_1 y_{2,2} \\
& C 4 t^2 x_2 x_{1,1} x_{1,2} y [ ] y_1 y_{1,2} C 2 t^2 x_2 x_{1,1} x_{2,2} y [ ] y_1 y_{1,1} K 4 t^2 x_2 x_{1,2} y [ ] y_1 y_{1,1} \\
& C s x [ ]^2 x_2 x_{1,1} y_{2,2}^2 K 2 s x [ ]^2 x_2 x_{1,2} y_{1,2} y_{2,2} K s x [ ]^2 x_2 x_{2,2} y_{1,1} y_{2,2} \\
& C 2 s x [ ]^2 x_2 x_{2,2} y_{1,2}^2 K s x [ ]^2 x_{1,1} x_{2,2} y_2 y_{2,2} C 2 s x [ ]^2 x_{1,1} y_1 y_{2,2}^2 \\
& K 2 s x [ ]^2 x_{1,1} y_2 y_{1,2} y_{2,2} C 2 s x [ ]^2 x_{1,2} y_2 y_{2,2} K 2 s x [ ]^2 x_{1,2} x_{2,2} y_2 y_{1,2} \\
& K 4 s x [ ]^2 x_{1,2} y_1 y_{1,2} y_{2,2} C 4 s x [ ]^2 x_{1,2} y_2 y_{1,1} y_{2,2} C s x [ ]^2 x_{2,2} y_2 y_{1,1} \\
& K 2 s x [ ]^2 x_{2,2} y_1 y_{1,1} y_{2,2} C 4 s x [ ]^2 x_{2,2} y_1 y_{1,2}^2 K 2 s x [ ]^2 x_{2,2} y_2 y_{1,1} y_{1,2} \\
& K 2 s x [ ] x_2 x_{1,1} y [ ] y_{1,2} y_{2,2} C 4 s x [ ] x_2 x_{1,2} y [ ] y_{1,1} y_{2,2} \\
& K 2 s x [ ] x_2 x_{2,2} y [ ] y_{1,1} y_{1,2} K 4 s x [ ] x_{1,1} x_{1,2} y [ ] y_2 y_{2,2} \\
& K 2 s x [ ] x_{1,1} x_{2,2} y [ ] y_1 y_{2,2} C 8 s x [ ] x_{1,1} x_{2,2} y [ ] y_2 y_{1,2} \\
& K 2 s x [ ] x_{1,1} y [ ] y_1 y_{1,2} y_{2,2} K 2 s x [ ] x_{1,1} y [ ] y_2 y_{1,1} y_{2,2} C 4 s x [ ] x_{1,1} y [ ] y_2 \\
& y_{1,2}^2 C 4 s x [ ] x_{1,2}^2 y [ ] y_1 y_{2,2} K 4 s x [ ] x_{1,2} x_{2,2} y [ ] y_1 y_{1,2} \\
& K 4 s x [ ] x_{1,2} x_{2,2} y [ ] y_2 y_{1,1} C 4 s x [ ] x_{1,2} y [ ] y_1 y_{1,1} y_{2,2} \\
& K 4 s x [ ] x_{1,2} y [ ] y_2 y_{1,1} y_{1,2} C 2 s x [ ] x_{2,2}^2 y [ ] y_1 y_{1,1} \\
& K 2 s x [ ] x_{2,2} y [ ] y_1 y_{1,1} y_{1,2} C 2 s x [ ] x_{2,2} y [ ] y_2 y_{1,1}^2 K s x_2 x_{1,1} y [ ]^2 y_{1,1} y_{2,2} \\
& C 2 s x_2 x_{1,1} y [ ]^2 y_{1,2}^2 K 2 s x_2 x_{1,2} y [ ]^2 y_{1,1} y_{1,2} C s x_2 x_{2,2} y [ ]^2 y_{1,1}^2 C 3 s \\
& x_{1,1} y [ ]^2 y_2 y_{2,2} K 2 s x_{1,1} x_{1,2} y [ ]^2 y_1 y_{2,2} K 6 s x_{1,1} x_{1,2} y [ ]^2 y_2 y_{1,2} \\
& C 4 s x_{1,1} x_{2,2} y [ ]^2 y_1 y_{1,2} K 3 s x_{1,1} x_{2,2} y [ ]^2 y_2 y_{1,1} C 6 s x_{1,2}^2 y [ ]^2 y_2 y_{1,1} \\
& K 2 s x_{1,2} x_{2,2} y [ ]^2 y_1 y_{1,1} C 3 t x [ ]^2 x_1 x_{1,1} y_{2,2}^2 K 6 t x [ ]^2 x_1 x_{1,2} y_{1,2} y_{2,2} \\
& K 3 t x [ ]^2 x_1 x_{2,2} y_{1,1} y_{2,2} C 6 t x [ ]^2 x_1 x_{2,2} y_{1,2}^2 K 2 t x [ ]^2 x_2 x_{1,1} y_{1,2} y_{2,2} \\
& C 4 t x [ ]^2 x_2 x_{1,2} y_{1,1} y_{2,2} K 2 t x [ ]^2 x_2 x_{2,2} y_{1,1} y_{1,2} K t x [ ]^2 x_{1,1} x_{2,2} y_1 y_{2,2} \\
& C 2 t x [ ]^2 x_{1,2}^2 y_1 y_{2,2} K 2 t x [ ]^2 x_{1,2} x_{2,2} y_1 y_{1,2} C t x [ ]^2 x_{2,2}^2 y_1 y_{1,1} \\
& K 2 t x [ ] x_1 x_{1,1} x_{2,2} y [ ] y_{2,2} K 4 t x [ ] x_1 x_{1,1} y [ ] y_{1,2} y_{2,2} C 4 t x [ ] x_1 x_{1,2}^2 y [ ] y_{2,2}
\end{aligned}$$

$$\begin{aligned}
& K 4 t x [ ] x_1 x_{1,2} x_{2,2} y [ ] y_{1,2} C 8 t x [ ] x_1 x_{1,2} y [ ] y_{1,1} y_{2,2} C 2 t x [ ] x_1 x_{2,2} y [ ] y_{1,1} \\
& K 4 t x [ ] x_1 x_{2,2} y [ ] y_{1,1} y_{1,2} K 2 t x [ ] x_2 x_{1,1} x_{1,2} y [ ] y_{2,2} \\
& C 4 t x [ ] x_2 x_{1,1} x_{2,2} y [ ] y_{1,2} K 2 t x [ ] x_2 x_{1,1} y [ ] y_{1,1} y_{2,2} C 4 t x [ ] x_2 x_{1,1} y [ ] y_{1,2}^2 \\
& K 2 t x [ ] x_2 x_{1,2} x_{2,2} y [ ] y_{1,1} K 4 t x [ ] x_2 x_{1,2} y [ ] y_{1,1} y_{1,2} C 2 t x [ ] x_2 x_{2,2} y [ ] y_{1,1}^2 \\
& K 2 t x [ ] x_{1,1} x_{1,2} y [ ] y_{1,2} y_{2,2} C 4 t x [ ] x_{1,1} x_{2,2} y [ ] y_{1,1} y_{1,2} \\
& K 2 t x [ ] x_{1,2} x_{2,2} y [ ] y_{1,1} y_{1,1} K 2 t x_1 x_{1,1} x_{1,2} y [ ] y_{2,2}^2 C 4 t x_1 x_{1,1} x_{2,2} y [ ] y_{1,2}^2 \\
& K t x_1 x_{1,1} y [ ] y_{1,1} y_{2,2}^2 C 2 t x_1 x_{1,1} y [ ] y_{1,2}^2 K 2 t x_1 x_{1,2} x_{2,2} y [ ] y_{1,1} \\
& K 2 t x_1 x_{1,2} y [ ] y_{1,1} y_{1,2} C t x_1 x_{2,2} y [ ] y_{1,1}^2 C 2 t x_2 x_{1,1} y [ ] y_{2,2}^2 \\
& K 4 t x_2 x_{1,1} x_{1,2} y [ ] y_{1,2} K 2 t x_2 x_{1,1} x_{2,2} y [ ] y_{1,1} C 4 t x_2 x_{1,2} y [ ] y_{1,1} C t \\
& x_{1,1} y [ ] y_{1,2} y_{2,2} K 2 t x_{1,1} x_{1,2} y [ ] y_{1,1} y_{1,2} K t x_{1,1} x_{2,2} y [ ] y_{1,1} y_{1,1} C 2 t \\
& x_{1,2} y [ ] y_{1,1} y_{1,1} K x [ ] x_{1,1} y_{2,2}^2 C 2 x [ ] x_{1,2} y_{1,2} y_{2,2} C x [ ] x_{2,2} y_{1,1} y_{2,2} \\
& K 2 x [ ] x_{2,2} y_{1,2}^2 C x [ ] x_{1,1} x_{2,2} y [ ] y_{2,2} C 2 x [ ] x_{1,1} y [ ] y_{1,2} y_{2,2} K 2 x [ ] y_{1,2}^2 \\
& x_{1,2} y [ ] y_{2,2} C 2 x [ ] x_{1,2} x_{2,2} y [ ] y_{1,2} K 4 x [ ] x_{1,2} y [ ] y_{1,1} y_{2,2} K x [ ] y_{2,2}^2 \\
& x_{2,2} y [ ] y_{1,1} C 2 x [ ] x_{2,2} y [ ] y_{1,1} y_{1,2} C 2 x [ ] x_{1,1} x_{1,2} y [ ] y_{2,2} \\
& K 4 x [ ] x_{1,1} x_{2,2} y [ ] y_{1,2} C x [ ] x_{1,1} y [ ] y_{1,1} y_{2,2} K 2 x [ ] x_{1,1} y [ ] y_{1,2}^2 \\
& C 2 x [ ] x_{1,2} x_{2,2} y [ ] y_{1,1} C 2 x [ ] x_{1,2} y [ ] y_{1,1} y_{1,2} K x [ ] x_{2,2} y [ ] y_{1,1}^2 K \\
& x_{1,1} y [ ] y_{2,2}^2 C 2 x_{1,1} x_{1,2} y [ ] y_{1,2} C x_{1,1} x_{2,2} y [ ] y_{1,1} K 2 x_{1,2} y [ ] y_{1,1} / \\
& ( 2 ( s^2 x_{1,1} y_1 y_2 y_{2,2} K s^2 x_{1,1} y_{2,2}^2 K s^2 x_{1,2} y_{2,2}^2 C s^2 x_{1,2} y_{2,2}^2 y_{1,1} C s^2 x_{2,2} y_{1,1}^2 y_{1,2} \\
& K s^2 x_{2,2} y_1 y_2 y_{1,1} C s t x_1 x_{1,1} y_2 y_{2,2} K 2 s t x_1 x_{1,2} y_1 y_{2,2} C 2 s t x_1 x_{2,2} y_1 y_{1,2} \\
& K s t x_1 x_{2,2} y_2 y_{1,1} C s t x_2 x_{1,1} y_1 y_{2,2} K 2 s t x_2 x_{1,1} y_2 y_{1,2} C 2 s t x_2 x_{1,2} y_2 y_{1,1} \\
& K s t x_2 x_{2,2} y_1 y_{1,1} K t^2 x_1^2 x_{1,2} y_{2,2} C t^2 x_1^2 x_{2,2} y_{1,2} C t^2 x_1 x_2 x_{1,1} y_{2,2} \\
& K t^2 x_1 x_2 x_{2,2} y_{1,1} K t^2 x_2^2 x_{1,1} y_{1,2} C t^2 x_2^2 x_{1,2} y_{1,1} K s x [ ] x_{1,1} y_2 y_{2,2} \\
& C 2 s x [ ] x_{1,2} y_1 y_{2,2} K 2 s x [ ] x_{2,2} y_1 y_{1,2} C s x [ ] x_{2,2} y_2 y_{1,1} K s x_{1,1} y [ ] y_1 y_{2,2} \\
& C 2 s x_{1,1} y [ ] y_2 y_{1,2} K 2 s x_{1,2} y [ ] y_2 y_{1,1} C s x_{2,2} y [ ] y_1 y_{1,1} C 2 t x [ ] x_1 x_{1,2} y_{2,2} \\
& K 2 t x [ ] x_1 x_{2,2} y_{1,2} K t x [ ] x_2 x_{1,1} y_{2,2} C t x [ ] x_2 x_{2,2} y_{1,1} K t x_1 x_{1,1} y [ ] y_{2,2} \\
& C t x_1 x_{2,2} y [ ] y_{1,1} C 2 t x_2 x_{1,1} y [ ] y_{1,2} K 2 t x_2 x_{1,2} y [ ] y_{1,1} K x [ ] x_{1,2} y_{2,2}^2 \\
& C x [ ] x_{2,2} y_{1,2} C x [ ] x_{1,1} y [ ] y_{2,2} K x [ ] x_{2,2} y [ ] y_{1,1} K x_{1,1} y [ ] y_{1,2}^2 \\
& C x_{1,2} y [ ] y_{1,1} ) ( x_2 K y_1 )^2 )
\end{aligned}$$

**M** >  $I_{2d} \text{d Hook}([w1, w1], Q2)$

$$\begin{aligned}
I_{2d} \text{d} & ( s^3 x_2 x_{1,1} y_1^2 y_{2,2}^3 K 2 s^3 x_2 x_{1,1} y_1 y_2 y_{1,2} y_{2,2}^2 C s^3 x_2 x_{1,1} y_2^2 y_{1,1} y_{2,2}^2 \\
& K 4 s^3 x_2 x_{1,1} x_{1,2} y_1^2 y_{1,2} y_{2,2}^2 C 8 s^3 x_2 x_{1,1} x_{1,2} y_1 y_2 y_{1,2} y_{2,2}^2 K 4 s^3 x_2 x_{1,1} x_{1,2} \\
& y_2^2 y_{1,1} y_{1,2} y_{2,2} K 2 s^3 x_2 x_{1,1} x_{2,2} y_1^2 y_{1,1} y_{2,2}^2 C 4 s^3 x_2 x_{1,1} x_{2,2} y_1^2 y_{1,2} y_{2,2}^2
\end{aligned}$$

(3.14)

$$\begin{aligned}
& C 4 s^3 x_2 x_{1,1} x_{2,2} y_1 y_2 y_{1,1} y_{1,2} y_{2,2} K 8 s^3 x_2 x_{1,1} x_{2,2} y_1 y_2 y_{1,2}^3 K 2 s^3 x_2 x_{1,1} x_{2,2} y_2^2 \\
& y_{1,1}^2 y_{2,2} C 4 s^3 x_2 x_{1,1} x_{2,2} y_2^2 y_{1,1} y_{1,2}^2 C 4 s^3 x_2 x_{1,2}^2 y_1^2 y_{1,1} y_{2,2}^2 K 8 s^3 x_2 \\
& x_{1,2}^2 y_1 y_2 y_{1,1} y_{1,2} y_{2,2} C 4 s^3 x_2 x_{1,2}^2 y_2^2 y_{1,1}^2 y_{2,2} K 4 s^3 x_2 x_{1,2} x_{2,2} y_1^2 y_{1,1} y_{1,2} y_{2,2} \\
& C 8 s^3 x_2 x_{1,2} x_{2,2} y_1 y_2 y_{1,1} y_{1,2}^2 K 4 s^3 x_2 x_{1,2} x_{2,2} y_2^2 y_{1,1}^2 y_{1,2} C s^3 x_2 x_{2,2}^2 y_1^2 y_{1,1}^2 y_{2,2} \\
& K 2 s^3 x_2 x_{2,2}^2 y_1 y_2 y_{1,1} y_{1,2} C s^3 x_2 x_{2,2}^2 y_2^3 y_{1,1} K s^3 x_{1,1}^3 y_2^3 y_{2,2}^2 C 2 s^3 x_{1,1}^2 x_{1,2} y_1 y_2^2 \\
& y_{2,2}^2 C 4 s^3 x_{1,1}^2 x_{1,2} y_2^3 y_{1,2} y_{2,2} K s^3 x_{1,1}^2 x_{2,2} y_1^2 y_2^2 y_{2,2}^2 C 2 s^3 x_{1,1}^2 x_{2,2} y_2^3 y_{1,1} y_{2,2} \\
& K 4 s^3 x_{1,1}^2 x_{2,2} y_2^3 y_{1,2}^2 K 8 s^3 x_{1,1} x_{1,2}^2 y_1 y_2^2 y_{1,2} y_{2,2} K 4 s^3 x_{1,1} x_{1,2}^2 y_2^3 y_{1,1} y_{2,2} \\
& C 4 s^3 x_{1,1} x_{1,2} x_{2,2} y_1^2 y_2 y_{1,2} y_{2,2} K 4 s^3 x_{1,1} x_{1,2} x_{2,2} y_1 y_2^2 y_{1,1} y_{2,2} \\
& C 8 s^3 x_{1,1} x_{1,2} x_{2,2} y_1 y_2^2 y_{1,2}^2 C 4 s^3 x_{1,1} x_{1,2} x_{2,2} y_2^3 y_{1,1} y_{1,2} C 2 s^3 x_{1,1} x_{2,2}^2 \\
& y_1^2 y_2 y_{1,1} y_{2,2} K 4 s^3 x_{1,1} x_{2,2}^2 y_1^2 y_2 y_{1,2}^2 K s^3 x_{1,1} x_{2,2}^2 y_2^3 y_{1,1}^2 C 8 s^3 x_{1,2}^3 y_1 y_2^2 y_{1,1} y_{2,2} \\
& K 4 s^3 x_{1,2}^2 x_{2,2} y_1^2 y_2 y_{1,1} y_{2,2} K 8 s^3 x_{1,2}^2 x_{2,2} y_1 y_2^2 y_{1,1} y_{1,2} C 4 s^3 x_{1,2} x_{2,2}^2 \\
& y_1^2 y_2 y_{1,1} y_{1,2} C 2 s^3 x_{1,2} x_{2,2}^2 y_1 y_2^2 y_{1,1} K s^3 x_{2,2}^3 y_1^2 y_2 y_{1,1}^2 C 2 s^2 t x_1 x_2 x_{1,1}^2 y_1 y_2^3 \\
& K 2 s^2 t x_1 x_2 x_{1,1}^2 y_2 y_{1,2} y_{2,2} K 8 s^2 t x_1 x_2 x_{1,1} x_{1,2} y_1 y_{1,2} y_{2,2}^2 \\
& C 8 s^2 t x_1 x_2 x_{1,1} x_{1,2} y_2 y_{1,2}^2 y_{2,2} K 4 s^2 t x_1 x_2 x_{1,1} x_{2,2} y_1 y_{1,1} y_{2,2}^2 \\
& C 8 s^2 t x_1 x_2 x_{1,1} x_{2,2} y_1 y_{1,2}^2 y_{2,2} C 4 s^2 t x_1 x_2 x_{1,1} x_{2,2} y_2 y_{1,1} y_{1,2} y_{2,2} \\
& K 8 s^2 t x_1 x_2 x_{1,1} x_{2,2} y_2 y_{1,2}^3 C 8 s^2 t x_1 x_2 x_{1,2}^2 y_1 y_{1,1} y_{2,2}^2 K 8 s^2 t x_1 x_2 \\
& x_{1,2}^2 y_2 y_{1,1} y_{1,2} y_{2,2} K 8 s^2 t x_1 x_2 x_{1,2} x_{2,2} y_1 y_{1,1} y_{1,2} y_{2,2} C 8 s^2 t x_1 x_2 x_{1,2} x_{2,2} y_2 y_{1,1} \\
& y_{1,2}^2 C 2 s^2 t x_1 x_2 x_{2,2}^2 y_1 y_{1,1} y_{2,2} K 2 s^2 t x_1 x_2 x_{2,2}^2 y_2 y_{1,1} y_{1,2} C 2 s^2 t x_1 x_{1,1}^2 x_{1,2} y_2^2 \\
& y_{2,2}^2 K 2 s^2 t x_1 x_{1,1}^2 x_{2,2} y_1 y_2 y_{2,2}^2 C s^2 t x_1 x_{1,1}^2 y_1^3 y_{2,2}^2 K 2 s^2 t x_1 x_{1,1}^2 y_1 y_2 y_{1,2} y_{2,2}^2 \\
& C s^2 t x_1 x_{1,1}^2 y_2^2 y_{1,1} y_{2,2}^2 K 8 s^2 t x_1 x_{1,1} x_{1,2}^2 y_2^2 y_{1,2} y_{2,2} \\
& C 8 s^2 t x_1 x_{1,1} x_{1,2} x_{2,2} y_1 y_2 y_{1,2} y_{2,2} K 4 s^2 t x_1 x_{1,1} x_{1,2} x_{2,2} y_2^2 y_{1,1} y_{2,2} \\
& C 8 s^2 t x_1 x_{1,1} x_{1,2} x_{2,2} y_2^2 y_{1,2}^2 K 4 s^2 t x_1 x_{1,1} x_{1,2} y_1^2 y_{1,2} y_{2,2} C 8 s^2 t x_1 x_{1,1} x_{1,2} y_1 y_2 \\
& y_{1,2}^2 y_{2,2} K 4 s^2 t x_1 x_{1,1} x_{1,2} y_2^2 y_{1,1} y_{1,2} y_{2,2} C 4 s^2 t x_1 x_{1,1} x_{2,2}^2 y_1 y_2 y_{1,1} y_{2,2} \\
& K 8 s^2 t x_1 x_{1,1} x_{2,2}^2 y_1 y_2 y_{1,2}^2 K 2 s^2 t x_1 x_{1,1} x_{2,2} y_1^2 y_{1,1} y_{2,2}^2 C 4 s^2 t x_1 x_{1,1} x_{2,2} y_1^2 \\
& y_{1,2}^2 y_{2,2} C 4 s^2 t x_1 x_{1,1} x_{2,2} y_1 y_2 y_{1,1} y_{1,2} y_{2,2} K 8 s^2 t x_1 x_{1,1} x_{2,2} y_1 y_2 y_{1,2}^3 \\
& K 2 s^2 t x_1 x_{1,1} x_{2,2} y_2^2 y_{1,1}^2 y_{2,2} C 4 s^2 t x_1 x_{1,1} x_{2,2} y_2^2 y_{1,1} y_{1,2}^2 C 8 s^2 t x_1 x_{1,2}^3 \\
& y_2^2 y_{1,1} y_{2,2} K 8 s^2 t x_1 x_{1,2}^2 x_{2,2} y_1 y_2 y_{1,1} y_{2,2} K 8 s^2 t x_1 x_{1,2}^2 x_{2,2} y_2^2 y_{1,1} y_{1,2} C 4 s^2 t x_1 \\
& x_{1,2}^2 y_1^2 y_{1,1} y_{2,2}^2 K 8 s^2 t x_1 x_{1,2}^2 y_1 y_2 y_{1,1} y_{1,2} y_{2,2} C 4 s^2 t x_1 x_{1,2}^2 y_2^2 y_{1,1}^2 y_{2,2} \\
& C 8 s^2 t x_1 x_{1,2} x_{2,2}^2 y_1 y_2 y_{1,1} y_{1,2} C 2 s^2 t x_1 x_{1,2} x_{2,2}^2 y_2^2 y_{1,1}^2 K 4 s^2 t x_1 x_{1,2} x_{2,2} \\
& y_1^2 y_{1,1} y_{1,2} y_{2,2} C 8 s^2 t x_1 x_{1,2} x_{2,2} y_1 y_2 y_{1,1} y_{1,2}^2 K 4 s^2 t x_1 x_{1,2} x_{2,2} y_2^2 y_{1,1}^2 y_{1,2} \\
& K 2 s^2 t x_1 x_{2,2}^3 y_1 y_2 y_{1,1} C s^2 t x_1 x_{2,2}^2 y_1^2 y_{1,1}^2 y_{2,2} K 2 s^2 t x_1 x_{2,2}^2 y_1 y_2 y_{1,1} y_{1,2} C s^2 t x_1 \\
& x_{2,2}^2 y_2^2 y_{1,1}^2 K 2 s^2 t x_2^2 x_{1,1}^2 y_1 y_{1,2} y_{2,2}^2 C 2 s^2 t x_2^2 x_{1,1}^2 y_2 y_{1,1} y_{2,2}^2 C 8 s^2 t x_2^2 x_{1,1} x_{1,2} y_1
\end{aligned}$$

$$\begin{aligned}
& y_{1,2}^2 y_{2,2} K 8 s^2 t x_2^2 x_{1,1} x_{1,2} y_2 y_{1,1} y_{1,2} y_{2,2} C 4 s^2 t x_2^2 x_{1,1} x_{2,2} y_1 y_{1,1} y_{1,2} y_{2,2} \\
& K 8 s^2 t x_2^2 x_{1,1} x_{2,2} y_1 y_{1,2}^3 K 4 s^2 t x_2^2 x_{1,1} x_{2,2} y_2 y_{1,1} y_{2,2} C 8 s^2 t x_2^2 x_{1,1} x_{2,2} y_2 y_{1,1} \\
& y_{1,2}^2 K 8 s^2 t x_2^2 x_{1,2}^2 y_1 y_{1,1} y_{1,2} y_{2,2} C 8 s^2 t x_2^2 x_{1,2}^2 y_2 y_{1,1} y_{2,2} C 8 s^2 t \\
& x_2^2 x_{1,2} x_{2,2} y_1 y_{1,1} y_{1,2}^2 K 8 s^2 t x_2^2 x_{1,2} x_{2,2} y_2 y_{1,1} y_{1,2} K 2 s^2 t x_2^2 x_{2,2}^2 y_1 y_{1,1} y_{1,2} \\
& C 2 s^2 t x_2^2 x_{2,2}^2 y_2 y_{1,1}^3 K 2 s^2 t x_2 x_{1,1}^3 y_2^2 y_{2,2}^2 C 2 s^2 t x_2 x_{1,1}^2 x_{1,2} y_1 y_2 y_{2,2}^2 C 8 s^2 t x_2 \\
& x_{1,1}^2 x_{1,2} y_2^2 y_{1,2} y_{2,2} C 4 s^2 t x_2 x_{1,1}^2 x_{2,2} y_2^2 y_{1,1} y_{2,2} K 8 s^2 t x_2 x_{1,1}^2 x_{2,2} y_2^2 y_{1,2}^2 \\
& K 8 s^2 t x_2 x_{1,1} x_{1,2}^2 y_1 y_2 y_{1,2} y_{2,2} K 8 s^2 t x_2 x_{1,1} x_{1,2}^2 y_2^2 y_{1,1} y_{2,2} \\
& K 4 s^2 t x_2 x_{1,1} x_{1,2} x_{2,2} y_1 y_2 y_{1,1} y_{2,2} C 8 s^2 t x_2 x_{1,1} x_{1,2} x_{2,2} y_1 y_2 y_{1,2}^2 \\
& C 8 s^2 t x_2 x_{1,1} x_{1,2} x_{2,2} y_2^2 y_{1,1} y_{1,2} K 2 s^2 t x_2 x_{1,1} x_{2,2}^2 y_2^2 y_{1,1}^2 C 8 s^2 t x_2 \\
& x_{1,2}^3 y_1 y_2 y_{1,1} y_{2,2} K 8 s^2 t x_2 x_{1,2}^2 x_{2,2} y_1 y_2 y_{1,1} y_{1,2} C 2 s^2 t x_2 x_{1,2} x_{2,2}^2 y_1 y_2 y_{1,1}^2 K s^2 t \\
& x_{1,1}^3 y_1 y_2^2 y_{2,2}^2 C 2 s^2 t x_{1,1}^2 x_{1,2} y_1^2 y_2^2 y_{2,2}^2 C 4 s^2 t x_{1,1}^2 x_{1,2} y_1 y_2^2 y_{1,2} y_{2,2} K s^2 t x_{1,1}^2 x_{2,2} \\
& y_1^3 y_{2,2}^2 C 2 s^2 t x_{1,1}^2 x_{2,2} y_1 y_2^2 y_{1,1} y_{2,2} K 4 s^2 t x_{1,1}^2 x_{2,2} y_1 y_2^2 y_{1,2} K 8 s^2 t x_{1,1} x_{1,2}^2 \\
& y_1^2 y_2 y_{1,2} y_{2,2} K 4 s^2 t x_{1,1} x_{1,2}^2 y_1 y_2^2 y_{1,1} y_{2,2} C 4 s^2 t x_{1,1} x_{1,2} x_{2,2} y_1^3 y_{1,2} y_{2,2} \\
& K 4 s^2 t x_{1,1} x_{1,2} x_{2,2} y_1^2 y_2 y_{1,1} y_{2,2} C 8 s^2 t x_{1,1} x_{1,2} x_{2,2} y_1^2 y_2 y_{1,2}^2 \\
& C 4 s^2 t x_{1,1} x_{1,2} x_{2,2} y_1 y_2^2 y_{1,1} y_{1,2} C 2 s^2 t x_{1,1} x_{2,2}^2 y_1^3 y_{1,1} y_{2,2} K 4 s^2 t x_{1,1} x_{2,2}^2 y_1^3 \\
& y_{1,2}^2 K s^2 t x_{1,1} x_{2,2}^2 y_1 y_2^2 y_{1,1}^2 C 8 s^2 t x_{1,2}^3 y_1^2 y_2 y_{1,1} y_{2,2} K 4 s^2 t x_{1,2}^2 x_{2,2}^2 y_1^3 y_{1,1} y_{2,2} \\
& K 8 s^2 t x_{1,2}^2 x_{2,2}^2 y_1^2 y_2 y_{1,1} y_{1,2} C 4 s^2 t x_{1,2} x_{2,2}^2 y_1^3 y_{1,1} y_{1,2} C 2 s^2 t x_{1,2} x_{2,2}^2 y_1^2 y_2 y_{1,1}^2 \\
& K s^2 t x_{2,2}^3 y_1^3 y_{1,1}^2 C s^2 t x_1^2 x_2 x_{1,1}^2 y_{2,2}^3 K 4 s^2 t x_1^2 x_2 x_{1,1} x_{1,2} y_{1,2} y_{2,2}^2 K 2 s^2 t \\
& x_1^2 x_2 x_{1,1} x_{2,2} y_{1,1} y_{2,2}^2 C 4 s^2 t x_1^2 x_2 x_{1,1} x_{2,2} y_{1,2}^2 y_{2,2} C 4 s^2 t x_1^2 x_2 x_{1,2}^2 y_{1,1} y_{2,2}^2 \\
& K 4 s^2 t x_1^2 x_2 x_{1,2} x_{2,2} y_{1,1} y_{1,2} y_{2,2} C s^2 t x_1^2 x_2 x_{2,2}^2 y_{1,1}^2 y_{2,2} K s^2 t x_1^2 x_{1,1}^2 x_{2,2} y_2 y_{2,2}^2 \\
& C 2 s^2 t x_1^2 x_{1,1}^2 y_1 y_{2,2}^3 K 2 s^2 t x_1^2 x_{1,1}^2 y_2 y_{1,2} y_{2,2}^2 C 4 s^2 t x_1^2 x_{1,1} x_{1,2} x_{2,2} y_2 y_{1,2} y_{2,2} \\
& K 8 s^2 t x_1^2 x_{1,1} x_{1,2} y_1 y_{1,2} y_{2,2}^2 C 8 s^2 t x_1^2 x_{1,1} x_{1,2} y_2 y_{1,2} y_{2,2} C 2 s^2 t x_1^2 x_{1,1} \\
& x_{2,2}^2 y_2 y_{1,1} y_{2,2} K 4 s^2 t x_1^2 x_{1,1} x_{2,2}^2 y_2 y_{1,2}^2 K 4 s^2 t x_1^2 x_{1,1} x_{2,2} y_1 y_{1,1} y_{2,2}^2 C 8 s^2 t \\
& x_1^2 x_{1,1} x_{2,2} y_1 y_{1,2} y_{2,2} C 4 s^2 t x_1^2 x_{1,1} x_{2,2} y_2 y_{1,1} y_{1,2} y_{2,2} K 8 s^2 t x_1^2 x_{1,1} x_{2,2} y_2 y_{1,2}^3 \\
& K 4 s^2 t x_1^2 x_{1,2}^2 x_{2,2} y_2 y_{1,1} y_{2,2} C 8 s^2 t x_1^2 x_{1,2}^2 y_1 y_{1,1} y_{2,2} K 8 s^2 t x_1^2 \\
& x_{1,2}^2 y_2 y_{1,1} y_{1,2} y_{2,2} C 4 s^2 t x_1^2 x_{1,2} x_{2,2}^2 y_2 y_{1,1} y_{1,2} K 8 s^2 t x_1^2 x_{1,2} x_{2,2} y_1 y_{1,1} y_{1,2} y_{2,2} \\
& C 8 s^2 t x_1^2 x_{1,2} x_{2,2} y_2 y_{1,1} y_{1,2}^2 K s^2 t x_1^2 x_{2,2}^3 y_2 y_{1,1}^2 C 2 s^2 t x_1^2 x_{2,2}^2 y_1 y_{1,2}^2 y_{2,2} K 2 s^2 t \\
& x_1^2 x_{2,2}^2 y_2 y_{1,1} y_{1,2} K 2 s^2 t x_1 x_2^2 x_{1,1}^2 y_{1,2} y_{2,2}^2 C 8 s^2 t x_1 x_2^2 x_{1,1} x_{1,2} y_{1,2} y_{2,2} C 4 s^2 t x_1 \\
& x_2^2 x_{1,1} x_{2,2} y_{1,1} y_{1,2} y_{2,2} K 8 s^2 t x_1 x_2^2 x_{1,1} x_{2,2} y_{1,2}^3 K 8 s^2 t x_1 x_2^2 x_{1,2}^2 y_{1,1} y_{1,2} y_{2,2} \\
& C 8 s^2 t x_1 x_2^2 x_{1,2} x_{2,2} y_{1,1} y_{1,2}^2 K 2 s^2 t x_1 x_2^2 x_{2,2}^2 y_{1,1}^2 y_{1,2} C 2 s^2 t x_1 x_2 x_{1,1}^2 x_{1,2} y_2 y_{2,2}^2 \\
& K 2 s^2 t x_1 x_2 x_{1,1}^2 y_1 y_{1,2} y_{2,2}^2 C 2 s^2 t x_1 x_2 x_{1,1}^2 y_2 y_{1,1} y_{2,2}^2 K 8 s^2 t x_1 x_2 x_{1,1} \\
& x_{1,2}^2 y_2 y_{1,2} y_{2,2} K 4 s^2 t x_1 x_2 x_{1,1} x_{1,2} x_{2,2} y_2 y_{1,1} y_{2,2} C 8 s^2 t x_1 x_2 x_{1,1} x_{1,2} x_{2,2} y_2 y_{1,2}^2
\end{aligned}$$

$$\begin{aligned}
& C 8 s^2 x_1 x_2 x_{1,1} x_{1,2} y_1 y_{1,2} y_2 K 8 s^2 x_1 x_2 x_{1,1} x_{1,2} y_2 y_{1,1} y_{1,2} y_2 \\
& C 4 s^2 x_1 x_2 x_{1,1} x_{2,2} y_1 y_{1,1} y_{1,2} y_2 K 8 s^2 x_1 x_2 x_{1,1} x_{2,2} y_1 y_{1,2}^3 \\
& K 4 s^2 x_1 x_2 x_{1,1} x_{2,2} y_2 y_{1,1} y_2 C 8 s^2 x_1 x_2 x_{1,1} x_{2,2} y_2 y_{1,1} y_{1,2}^2 C 8 s^2 x_1 x_2 \\
& x_{1,2}^3 y_2 y_{1,1} y_2 K 8 s^2 x_1 x_2 x_{1,2}^2 x_{2,2} y_2 y_{1,1} y_{1,2} K 8 s^2 x_1 x_2 x_{1,2}^2 y_1 y_{1,1} y_{1,2} y_2 \\
& C 8 s^2 x_1 x_2 x_{1,2}^2 y_2 y_{1,1} y_2 C 2 s^2 x_1 x_2 x_{1,2} x_{2,2}^2 y_2 y_{1,1}^2 \\
& C 8 s^2 x_1 x_2 x_{1,2} x_{2,2} y_1 y_{1,1} y_{1,2}^2 K 8 s^2 x_1 x_2 x_{1,2} x_{2,2} y_2 y_{1,1} y_{1,2} K 2 s^2 x_1 x_2 \\
& x_{2,2}^2 y_1 y_{1,1} y_{1,2} C 2 s^2 x_1 x_2 x_{2,2}^2 y_2 y_{1,1}^3 C 2 s^2 x_1 x_{1,1} x_{1,2} y_1 y_2 y_{1,2}^2 K 2 s^2 x_1 \\
& x_{1,1}^2 x_{2,2} y_1^2 y_{1,2}^2 K 8 s^2 x_1 x_{1,1} x_{1,2}^2 y_1 y_2 y_{1,2} y_2 C 8 s^2 x_1 x_{1,1} x_{1,2} x_{2,2} y_1^2 y_{1,2} y_2 \\
& K 4 s^2 x_1 x_{1,1} x_{1,2} x_{2,2} y_1 y_2 y_{1,1} y_2 C 8 s^2 x_1 x_{1,1} x_{1,2} x_{2,2} y_1 y_2 y_{1,2}^2 C 4 s^2 x_1 x_{1,1} \\
& x_{2,2}^2 y_1^2 y_{1,1} y_2 K 8 s^2 x_1 x_{1,1} x_{2,2}^2 y_1^2 y_{1,2}^2 C 8 s^2 x_1 x_{1,2}^3 y_1 y_2 y_{1,1} y_2 K 8 s^2 x_1 \\
& x_{1,2}^2 x_{2,2} y_1^2 y_{1,1} y_2 K 8 s^2 x_1 x_{1,2}^2 x_{2,2} y_1 y_2 y_{1,1} y_{1,2} C 8 s^2 x_1 x_{1,2} x_{2,2}^2 y_1^2 y_{1,1} y_{1,2} \\
& C 2 s^2 x_1 x_{1,2} x_{2,2}^2 y_1 y_2 y_{1,1} K 2 s^2 x_1 x_{2,2}^2 y_1^2 y_{1,1} C s^2 x_2^3 x_{1,1}^2 y_{1,1} y_{1,2}^2 K 4 s^2 \\
& x_2^3 x_{1,1} x_{1,2} y_1 y_{1,1} y_{1,2} y_2 K 2 s^2 x_2^3 x_{1,1} x_{2,2} y_1^2 y_{1,1} y_2 C 4 s^2 x_2^3 x_{1,1} x_{2,2} y_1 y_{1,1} y_{1,2}^2 \\
& C 4 s^2 x_2^3 x_{1,2}^2 y_{1,1} y_2 K 4 s^2 x_2^3 x_{1,2} x_{2,2} y_{1,1} y_{1,2} C s^2 x_2^3 x_{2,2}^2 y_{1,1}^3 K s^2 x_2^2 x_{1,1}^3 y_2 \\
& y_{1,2}^2 C 4 s^2 x_2^2 x_{1,1}^2 x_{1,2} y_2 y_{1,2} y_2 C 2 s^2 x_2^2 x_{1,1}^2 x_{2,2} y_2 y_{1,1} y_2 K 4 s^2 x_2^2 \\
& x_{1,1}^2 x_{2,2} y_2 y_{1,2}^2 K 4 s^2 x_2^2 x_{1,1} x_{1,2}^2 y_2 y_{1,1} y_2 C 4 s^2 x_2^2 x_{1,1} x_{1,2} x_{2,2} y_2 y_{1,1} y_{1,2} \\
& K s^2 x_2^2 x_{1,1} x_{2,2}^2 y_2 y_{1,1} K 2 s^2 x_2 x_{1,1}^3 y_1 y_2 y_{1,2}^2 C 2 s^2 x_2 x_{1,1}^2 x_{1,2} y_1^2 y_{1,2}^2 C 8 s^2 x_2 \\
& x_{1,1}^2 x_{1,2} y_1 y_2 y_{1,2} y_2 C 4 s^2 x_2 x_{1,1}^2 x_{2,2} y_1 y_2 y_{1,1} y_2 K 8 s^2 x_2 x_{1,1}^2 x_{2,2} y_1 y_2 y_{1,2}^2 \\
& K 8 s^2 x_2 x_{1,1} x_{1,2}^2 y_1^2 y_{1,2} y_2 K 8 s^2 x_2 x_{1,1} x_{1,2}^2 y_1 y_2 y_{1,1} y_2 \\
& K 4 s^2 x_2 x_{1,1} x_{1,2} x_{2,2} y_1^2 y_{1,1} y_2 C 8 s^2 x_2 x_{1,1} x_{1,2} x_{2,2} y_1^2 y_{1,2}^2 \\
& C 8 s^2 x_2 x_{1,1} x_{1,2} x_{2,2} y_1 y_2 y_{1,1} y_{1,2} K 2 s^2 x_2 x_{1,1} x_{2,2}^2 y_1 y_2 y_{1,1}^2 C 8 s^2 x_2 x_{1,2}^3 \\
& y_{1,1}^2 y_{1,2} K 8 s^2 x_2 x_{1,2}^2 x_{2,2} y_1^2 y_{1,1} y_{1,2} C 2 s^2 x_2 x_{1,2} x_{2,2}^2 y_1^2 y_{1,1}^2 C t^3 x_1^3 x_{1,1}^2 y_{1,2}^3 \\
& K 4 t^3 x_1^3 x_{1,1} x_{1,2} y_1 y_{1,2} y_2 K 2 t^3 x_1^3 x_{1,1} x_{2,2} y_1 y_{1,2}^2 C 4 t^3 x_1^3 x_{1,1} x_{2,2} y_{1,2}^2 y_2 \\
& C 4 t^3 x_1^3 x_{1,2}^2 y_{1,1} y_2 K 4 t^3 x_1^3 x_{1,2} x_{2,2} y_{1,1} y_{1,2} y_2 C t^3 x_1^3 x_{2,2}^2 y_{1,1} y_2 K 2 t^3 x_1^2 x_2 \\
& x_{1,1}^2 y_{1,2} y_2 C 8 t^3 x_1^2 x_2 x_{1,1} x_{1,2} y_{1,2} y_2 C 4 t^3 x_1^2 x_2 x_{1,1} x_{2,2} y_{1,1} y_{1,2} y_2 K 8 t^3 \\
& x_1^2 x_2 x_{1,1} x_{2,2} y_{1,2}^3 K 8 t^3 x_1^2 x_2 x_{1,2}^2 y_{1,1} y_{1,2} y_2 C 8 t^3 x_1^2 x_2 x_{1,2} x_{2,2} y_{1,1} y_{1,2}^2 K 2 t^3 \\
& x_1^2 x_2 x_{2,2}^2 y_{1,1} y_{1,2} K t^3 x_1^2 x_{1,1}^2 x_{2,2} y_1 y_2^2 C 4 t^3 x_1^2 x_{1,1} x_{1,2} x_{2,2} y_1 y_{1,2} y_2 C 2 t^3 \\
& x_1^2 x_{1,1} x_{2,2}^2 y_1 y_{1,1} y_2 K 4 t^3 x_1^2 x_{1,1} x_{2,2}^2 y_1 y_{1,2} K 4 t^3 x_1^2 x_{1,2}^2 x_{2,2} y_1 y_{1,1} y_2 C 4 t^3 \\
& x_1^2 x_{1,2} x_{2,2}^2 y_1 y_{1,1} y_2 K t^3 x_1^2 x_{2,2}^3 y_1 y_{1,1} C t^3 x_1 x_2^2 x_{1,1}^2 y_{1,1} y_{1,2}^2 K 4 t^3 x_1 \\
& x_2^2 x_{1,1} x_{1,2} y_1 y_{1,1} y_{1,2} y_2 K 2 t^3 x_1 x_2^2 x_{1,1} x_{2,2} y_{1,1} y_2 C 4 t^3 x_1 x_2^2 x_{1,1} x_{2,2} y_{1,1} y_{1,2}^2 \\
& C 4 t^3 x_1 x_2^2 x_{1,2}^2 y_{1,1} y_2 K 4 t^3 x_1 x_2^2 x_{1,2} x_{2,2} y_{1,1} y_2 C t^3 x_1 x_2^2 x_{2,2}^2 y_{1,1}^3 C 2 t^3 x_1 x_2 \\
& x_{1,1}^2 x_{1,2} y_1 y_{1,2}^2 K 8 t^3 x_1 x_2 x_{1,1} x_{1,2}^2 y_1 y_{1,2} y_2 K 4 t^3 x_1 x_2 x_{1,1} x_{1,2} x_{2,2} y_1 y_{1,1} y_2
\end{aligned}$$

$$\begin{aligned}
& \mathbb{C} 8 t^3 x_1 x_2 x_{1,1} x_{1,2} x_{2,2} y_1 y_{1,2}^2 \mathbb{C} 8 t^3 x_1 x_2 x_{1,2}^3 y_1 y_{1,1} y_{2,2} \mathbb{K} 8 t^3 x_1 x_2 \\
& x_{1,2}^2 x_{2,2} y_1 y_{1,1} y_{1,2} \mathbb{C} 2 t^3 x_1 x_2 x_{1,2} x_{2,2}^2 y_1 y_{1,1}^2 \mathbb{K} t^3 x_2^2 x_{1,1}^3 y_1 y_{2,2}^2 \mathbb{C} 4 t^3 x_2^2 \\
& x_{1,1}^2 x_{1,2} y_1 y_{1,2} y_{2,2} \mathbb{C} 2 t^3 x_2^2 x_{1,1}^2 x_{2,2} y_1 y_{1,1} y_{2,2} \mathbb{K} 4 t^3 x_2^2 x_{1,1}^2 x_{2,2} y_1 y_{1,2}^2 \mathbb{K} 4 t^3 \\
& x_2^2 x_{1,1} x_{1,2}^2 y_1 y_{1,1} y_{2,2} \mathbb{C} 4 t^3 x_2^2 x_{1,1} x_{1,2} x_{2,2} y_1 y_{1,1} y_{1,2} \mathbb{K} t^3 x_2^2 x_{1,1} x_{2,2}^2 y_1 y_{1,1}^2 \\
& \mathbb{K} 2 s^2 x[ ] x_2 x_{1,1}^2 y_1 y_{2,2}^3 \mathbb{C} 2 s^2 x[ ] x_2 x_{1,1}^2 y_2 y_{1,2} y_{2,2}^2 \mathbb{C} 8 s^2 x[ ] x_2 x_{1,1} x_{1,2} y_1 y_{1,2} \\
& y_{2,2}^2 \mathbb{K} 8 s^2 x[ ] x_2 x_{1,1} x_{1,2} y_2 y_{1,2}^2 y_{2,2} \mathbb{C} 4 s^2 x[ ] x_2 x_{1,1} x_{2,2} y_1 y_{1,1} y_{2,2}^2 \\
& \mathbb{K} 8 s^2 x[ ] x_2 x_{1,1} x_{2,2} y_1 y_{1,2}^2 y_{2,2} \mathbb{K} 4 s^2 x[ ] x_2 x_{1,1} x_{2,2} y_2 y_{1,1} y_{1,2} y_{2,2} \\
& \mathbb{C} 8 s^2 x[ ] x_2 x_{1,1} x_{2,2} y_2 y_{1,2}^3 \mathbb{K} 8 s^2 x[ ] x_2 x_{1,2}^2 y_1 y_{1,1} y_{2,2}^2 \mathbb{C} 8 s^2 x[ ] x_2 \\
& x_{1,2}^2 y_2 y_{1,1} y_{1,2} y_{2,2} \mathbb{C} 8 s^2 x[ ] x_2 x_{1,2} x_{2,2} y_1 y_{1,1} y_{1,2} y_{2,2} \\
& \mathbb{K} 8 s^2 x[ ] x_2 x_{1,2} x_{2,2} y_2 y_{1,1} y_{1,2}^2 \mathbb{K} 2 s^2 x[ ] x_2 x_{2,2}^2 y_1 y_{1,1} y_{2,2} \mathbb{C} 2 s^2 x[ ] x_2 x_{2,2}^2 y_2 \\
& y_{1,1} y_{1,2} \mathbb{K} 2 s^2 x[ ] x_{1,1}^2 x_{1,2} y_2^2 y_{2,2}^2 \mathbb{C} 2 s^2 x[ ] x_{1,1}^2 x_{2,2} y_1 y_2 y_{2,2}^2 \mathbb{K} s^2 x[ ] x_{1,1}^2 y_1^2 y_{2,2}^3 \\
& \mathbb{C} 2 s^2 x[ ] x_{1,1}^2 y_1 y_2 y_{1,2} y_{2,2}^2 \mathbb{K} s^2 x[ ] x_{1,1}^2 y_2^2 y_{1,1} y_{2,2}^2 \mathbb{C} 8 s^2 x[ ] x_{1,1} x_{1,2}^2 y_2^2 y_{1,2} y_{2,2} \\
& \mathbb{K} 8 s^2 x[ ] x_{1,1} x_{1,2} x_{2,2} y_1 y_2 y_{1,2} y_{2,2} \mathbb{C} 4 s^2 x[ ] x_{1,1} x_{1,2} x_{2,2} y_2^2 y_{1,1} y_{2,2} \\
& \mathbb{K} 8 s^2 x[ ] x_{1,1} x_{1,2} x_{2,2} y_2^2 y_{1,2}^2 \mathbb{C} 4 s^2 x[ ] x_{1,1} x_{1,2} y_1^2 y_{1,2} y_{2,2}^2 \\
& \mathbb{K} 8 s^2 x[ ] x_{1,1} x_{1,2} y_1 y_2 y_{1,2}^2 y_{2,2} \mathbb{C} 4 s^2 x[ ] x_{1,1} x_{1,2} y_2^2 y_{1,1} y_{1,2} y_{2,2} \mathbb{K} 4 s^2 x[ ] x_{1,1} \\
& x_{2,2}^2 y_1 y_2 y_{1,1} y_{2,2} \mathbb{C} 8 s^2 x[ ] x_{1,1} x_{2,2}^2 y_1 y_2 y_{1,2}^2 \mathbb{C} 2 s^2 x[ ] x_{1,1} x_{2,2}^2 y_1^2 y_{1,1} y_{2,2}^2 \\
& \mathbb{K} 4 s^2 x[ ] x_{1,1} x_{2,2}^2 y_1^2 y_{1,2}^2 y_{2,2} \mathbb{K} 4 s^2 x[ ] x_{1,1} x_{2,2} y_1 y_2 y_{1,1} y_{1,2} y_{2,2} \\
& \mathbb{C} 8 s^2 x[ ] x_{1,1} x_{2,2} y_1 y_2 y_{1,2}^3 \mathbb{C} 2 s^2 x[ ] x_{1,1} x_{2,2} y_2^2 y_{1,1} y_{2,2} \mathbb{K} 4 s^2 x[ ] x_{1,1} x_{2,2} \\
& y_2^2 y_{1,1} y_{1,2}^2 \mathbb{K} 8 s^2 x[ ] x_{1,2}^3 y_2^2 y_{1,1} y_{2,2} \mathbb{C} 8 s^2 x[ ] x_{1,2}^2 x_{2,2} y_1 y_2 y_{1,1} y_{2,2} \mathbb{C} 8 s^2 x[ ] \\
& x_{1,2}^2 x_{2,2} y_2^2 y_{1,1} y_{1,2} \mathbb{K} 4 s^2 x[ ] x_{1,2}^2 y_1^2 y_{1,1} y_{2,2}^2 \mathbb{C} 8 s^2 x[ ] x_{1,2}^2 y_1 y_2 y_{1,1} y_{1,2} y_{2,2} \\
& \mathbb{K} 4 s^2 x[ ] x_{1,2}^2 y_2^2 y_{1,1} y_{2,2} \mathbb{K} 8 s^2 x[ ] x_{1,2} x_{2,2}^2 y_1 y_2 y_{1,1} y_{1,2} \mathbb{K} 2 s^2 x[ ] x_{1,2} x_{2,2}^2 y_2^2 \\
& y_{1,1}^2 \mathbb{C} 4 s^2 x[ ] x_{1,2} x_{2,2} y_1^2 y_{1,1} y_{1,2} y_{2,2} \mathbb{K} 8 s^2 x[ ] x_{1,2} x_{2,2} y_1 y_2 y_{1,1} y_{1,2}^2 \\
& \mathbb{C} 4 s^2 x[ ] x_{1,2} x_{2,2} y_2^2 y_{1,1}^2 y_{1,2} \mathbb{C} 2 s^2 x[ ] x_{2,2}^3 y_1 y_2 y_{1,1}^2 \mathbb{K} s^2 x[ ] x_{2,2}^2 y_1^2 y_{1,1} y_{2,2} \\
& \mathbb{C} 2 s^2 x[ ] x_{2,2}^2 y_1 y_2 y_{1,1}^2 y_{1,2} \mathbb{K} s^2 x[ ] x_{2,2}^2 y_2^3 y_{1,1} \mathbb{C} 2 s^2 x_2 x_{1,1}^2 y[ ] y_1 y_{1,2} y_{2,2}^2 \\
& \mathbb{K} 2 s^2 x_2 x_{1,1}^2 y[ ] y_2 y_{1,1} y_{2,2}^2 \mathbb{K} 8 s^2 x_2 x_{1,1} x_{1,2} y[ ] y_1 y_{1,2}^2 y_{2,2} \\
& \mathbb{C} 8 s^2 x_2 x_{1,1} x_{1,2} y[ ] y_2 y_{1,1} y_{1,2} y_{2,2} \mathbb{K} 4 s^2 x_2 x_{1,1} x_{2,2} y[ ] y_1 y_{1,1} y_{1,2} y_{2,2} \\
& \mathbb{C} 8 s^2 x_2 x_{1,1} x_{2,2} y[ ] y_1 y_{1,2}^3 \mathbb{C} 4 s^2 x_2 x_{1,1} x_{2,2} y[ ] y_2 y_{1,1}^2 y_{2,2} \\
& \mathbb{K} 8 s^2 x_2 x_{1,1} x_{2,2} y[ ] y_2 y_{1,1} y_{1,2}^2 \mathbb{C} 8 s^2 x_2 x_{1,2}^2 y[ ] y_1 y_{1,1} y_{1,2} y_{2,2} \mathbb{K} 8 s^2 x_2 \\
& x_{1,2}^2 y[ ] y_2 y_{1,1}^2 y_{2,2} \mathbb{K} 8 s^2 x_2 x_{1,2} x_{2,2} y[ ] y_1 y_{1,1} y_{1,2}^2 \mathbb{C} 8 s^2 x_2 x_{1,2} x_{2,2} y[ ] y_2 \\
& y_{1,1}^2 y_{1,2} \mathbb{C} 2 s^2 x_2 x_{2,2}^2 y[ ] y_1 y_{1,1}^2 y_{1,2} \mathbb{K} 2 s^2 x_2 x_{2,2}^2 y[ ] y_2 y_{1,1}^3 \mathbb{C} 3 s^2 x_{1,1}^3 y[ ] y_2^2 y_{2,2}^2 \\
& \mathbb{K} 4 s^2 x_{1,1}^2 x_{1,2} y[ ] y_1 y_2 y_{2,2}^2 \mathbb{K} 12 s^2 x_{1,1}^2 x_{1,2} y[ ] y_2^2 y_{1,2} y_{2,2} \mathbb{C} s^2 x_{1,1}^2 x_{2,2} y[ ] y_1^2 \\
& y_{2,2}^2 \mathbb{K} 6 s^2 x_{1,1}^2 x_{2,2} y[ ] y_2^2 y_{1,1} y_{2,2} \mathbb{C} 12 s^2 x_{1,1}^2 x_{2,2} y[ ] y_2^2 y_{1,2}^2 \mathbb{C} 16 s^2 x_{1,1}
\end{aligned}$$

$$\begin{aligned}
& x_{1,2}^2 y [ ] y_1 y_2 y_{1,2} y_{2,2} \mathbf{C} 12 s^2 x_{1,1} x_{1,2}^2 y [ ] y_2^2 y_{1,1} y_{2,2} \mathbf{K} 4 s^2 x_{1,1} x_{1,2} x_{2,2} y [ ] \\
& y_1^2 y_{1,2} y_{2,2} \mathbf{C} 8 s^2 x_{1,1} x_{1,2} x_{2,2} y [ ] y_1 y_2 y_{1,1} y_{2,2} \mathbf{K} 16 s^2 x_{1,1} x_{1,2} x_{2,2} y [ ] y_1 y_2 y_{1,2}^2 \\
& \mathbf{K} 12 s^2 x_{1,1} x_{1,2} x_{2,2} y [ ] y_2^2 y_{1,1} y_{1,2} \mathbf{K} 2 s^2 x_{1,1} x_{2,2}^2 y [ ] y_1^2 y_{1,1} y_{2,2} \mathbf{C} 4 s^2 x_{1,1} \\
& x_{2,2}^2 y [ ] y_1^2 y_{1,2}^2 \mathbf{C} 3 s^2 x_{1,1} x_{2,2}^2 y [ ] y_2^2 y_{1,1}^2 \mathbf{K} 16 s^2 x_{1,2}^3 y [ ] y_1 y_2 y_{1,1} y_{2,2} \mathbf{C} 4 s^2 \\
& x_{1,2}^2 x_{2,2} y [ ] y_1^2 y_{1,1} y_{2,2} \mathbf{C} 16 s^2 x_{1,2}^2 x_{2,2} y [ ] y_1 y_2 y_{1,1} y_{1,2} \mathbf{K} 4 s^2 x_{1,2} x_{2,2}^2 y [ ] \\
& y_1^2 y_{1,1} y_{1,2} \mathbf{K} 4 s^2 x_{1,2} x_{2,2}^2 y [ ] y_1 y_2 y_{1,1}^2 \mathbf{C} s^2 x_{2,2}^3 y [ ] y_1^2 y_{1,1}^2 \mathbf{K} 2 s t x [ ] x_1 x_2 x_{1,1}^2 y_{2,2}^3 \\
& \mathbf{C} 8 s t x [ ] x_1 x_2 x_{1,1} x_{1,2} y_{1,2} y_{2,2}^2 \mathbf{C} 4 s t x [ ] x_1 x_2 x_{1,1} x_{2,2} y_{1,1} y_{2,2}^2 \\
& \mathbf{K} 8 s t x [ ] x_1 x_2 x_{1,1} x_{2,2} y_{1,2} y_{2,2}^2 \mathbf{K} 8 s t x [ ] x_1 x_2 x_{1,2}^2 y_{1,1} y_{2,2}^2 \\
& \mathbf{C} 8 s t x [ ] x_1 x_2 x_{1,2} x_{2,2} y_{1,1} y_{1,2} y_{2,2} \mathbf{K} 2 s t x [ ] x_1 x_2 x_{2,2}^2 y_{1,1} y_{2,2} \mathbf{C} 2 s t x [ ] x_1 \\
& x_{1,1}^2 x_{2,2} y_{2,2}^2 \mathbf{K} 4 s t x [ ] x_1 x_{1,1}^2 y_1 y_{2,2}^3 \mathbf{C} 4 s t x [ ] x_1 x_{1,1}^2 y_2 y_{1,2} y_{2,2}^2 \\
& \mathbf{K} 8 s t x [ ] x_1 x_{1,1} x_{1,2} x_{2,2} y_2 y_{1,2} y_{2,2} \mathbf{C} 16 s t x [ ] x_1 x_{1,1} x_{1,2} y_1 y_{1,2} y_{2,2}^2 \\
& \mathbf{K} 16 s t x [ ] x_1 x_{1,1} x_{1,2} y_2 y_{1,2} y_{2,2} \mathbf{K} 4 s t x [ ] x_1 x_{1,1} x_{2,2}^2 y_2 y_{1,1} y_{2,2} \\
& \mathbf{C} 8 s t x [ ] x_1 x_{1,1} x_{2,2}^2 y_2 y_{1,2}^2 \mathbf{C} 8 s t x [ ] x_1 x_{1,1} x_{2,2} y_1 y_{1,1} y_{2,2}^2 \\
& \mathbf{K} 16 s t x [ ] x_1 x_{1,1} x_{2,2} y_1 y_{1,2} y_{2,2} \mathbf{K} 8 s t x [ ] x_1 x_{1,1} x_{2,2} y_2 y_{1,1} y_{1,2} y_{2,2} \\
& \mathbf{C} 16 s t x [ ] x_1 x_{1,1} x_{2,2} y_2 y_{1,2}^3 \mathbf{C} 8 s t x [ ] x_1 x_{1,2}^2 x_{2,2} y_2 y_{1,1} y_{2,2} \mathbf{K} 16 s t x [ ] x_1 \\
& x_{1,2}^2 y_1 y_{1,1} y_{2,2}^2 \mathbf{C} 16 s t x [ ] x_1 x_{1,2}^2 y_2 y_{1,1} y_{1,2} y_{2,2} \mathbf{K} 8 s t x [ ] x_1 x_{1,2} x_{2,2}^2 y_2 y_{1,1} y_{1,2} \\
& \mathbf{C} 16 s t x [ ] x_1 x_{1,2} x_{2,2} y_1 y_{1,1} y_{1,2} y_{2,2} \mathbf{K} 16 s t x [ ] x_1 x_{1,2} x_{2,2} y_2 y_{1,1} y_{1,2}^2 \\
& \mathbf{C} 2 s t x [ ] x_1 x_{2,2}^3 y_2 y_{1,1}^2 \mathbf{K} 4 s t x [ ] x_1 x_{2,2}^2 y_1 y_{1,1}^2 y_{2,2} \mathbf{C} 4 s t x [ ] x_1 x_{2,2}^2 y_2 y_{1,1}^2 y_{1,2} \\
& \mathbf{C} 2 s t x [ ] x_2^2 x_{1,1}^2 y_{1,2} y_{2,2}^2 \mathbf{K} 8 s t x [ ] x_2^2 x_{1,1} x_{1,2} y_{1,2}^2 y_{2,2} \mathbf{K} 4 s t x [ ] \\
& x_2^2 x_{1,1} x_{2,2} y_{1,1} y_{1,2} y_{2,2} \mathbf{C} 8 s t x [ ] x_2^2 x_{1,1} x_{2,2} y_{1,2}^3 \mathbf{C} 8 s t x [ ] x_2^2 x_{1,2}^2 y_{1,1} y_{1,2} y_{2,2} \\
& \mathbf{K} 8 s t x [ ] x_2^2 x_{1,2} x_{2,2} y_{1,1} y_{1,2}^2 \mathbf{C} 2 s t x [ ] x_2^2 x_{2,2}^2 y_{1,1}^2 y_{1,2} \mathbf{K} 2 s t x [ ] x_2 x_{1,1}^2 x_{1,2} y_2 \\
& y_{2,2}^2 \mathbf{C} 2 s t x [ ] x_2 x_{1,1}^2 y_1 y_{1,2} y_{2,2}^2 \mathbf{K} 2 s t x [ ] x_2 x_{1,1}^2 y_2 y_{1,1} y_{2,2}^2 \mathbf{C} 8 s t x [ ] x_2 x_{1,1} \\
& x_{1,2}^2 y_2 y_{1,2} y_{2,2} \mathbf{C} 4 s t x [ ] x_2 x_{1,1} x_{1,2} x_{2,2} y_2 y_{1,1} y_{2,2} \mathbf{K} 8 s t x [ ] x_2 x_{1,1} x_{1,2} x_{2,2} y_2 \\
& y_{1,2}^2 \mathbf{K} 8 s t x [ ] x_2 x_{1,1} x_{1,2} y_1 y_{1,2} y_{2,2} \mathbf{C} 8 s t x [ ] x_2 x_{1,1} x_{1,2} y_2 y_{1,1} y_{1,2} y_{2,2} \\
& \mathbf{K} 4 s t x [ ] x_2 x_{1,1} x_{2,2} y_1 y_{1,1} y_{1,2} y_{2,2} \mathbf{C} 8 s t x [ ] x_2 x_{1,1} x_{2,2} y_1 y_{1,2}^3 \\
& \mathbf{C} 4 s t x [ ] x_2 x_{1,1} x_{2,2} y_2 y_{1,1} y_{2,2} \mathbf{K} 8 s t x [ ] x_2 x_{1,1} x_{2,2} y_2 y_{1,1} y_{1,2}^2 \mathbf{K} 8 s t x [ ] x_2 \\
& x_{1,2}^3 y_2 y_{1,1} y_{2,2} \mathbf{C} 8 s t x [ ] x_2 x_{1,2}^2 x_{2,2} y_2 y_{1,1} y_{1,2} \mathbf{C} 8 s t x [ ] x_2 x_{1,2}^2 y_1 y_{1,1} y_{1,2} y_{2,2} \\
& \mathbf{K} 8 s t x [ ] x_2 x_{1,2}^2 y_2 y_{1,1} y_{2,2} \mathbf{K} 2 s t x [ ] x_2 x_{1,2}^2 y_2 y_{1,1}^2 \\
& \mathbf{K} 8 s t x [ ] x_2 x_{1,2} x_{2,2} y_1 y_{1,1} y_{1,2}^2 \mathbf{C} 8 s t x [ ] x_2 x_{1,2} x_{2,2} y_2 y_{1,1} y_{1,2} \mathbf{C} 2 s t x [ ] x_2 \\
& x_{2,2}^2 y_1 y_{1,1}^2 y_{1,2} \mathbf{K} 2 s t x [ ] x_2 x_{2,2}^2 y_2 y_{1,1}^3 \mathbf{K} 2 s t x [ ] x_{1,1}^2 x_{1,2} y_1 y_2 y_{2,2}^2 \mathbf{C} 2 s t x [ ] \\
& x_{1,1}^2 x_{2,2} y_1^2 y_{2,2}^2 \mathbf{C} 8 s t x [ ] x_{1,1} x_{1,2}^2 y_1 y_2 y_{1,2} y_{2,2} \mathbf{K} 8 s t x [ ] x_{1,1} x_{1,2} x_{2,2} y_{1,1}^2 y_{1,2} y_{2,2} \\
& \mathbf{C} 4 s t x [ ] x_{1,1} x_{1,2} x_{2,2} y_1 y_2 y_{1,1} y_{2,2} \mathbf{K} 8 s t x [ ] x_{1,1} x_{1,2} x_{2,2} y_1 y_2 y_{1,1}^2 y_{2,2}
\end{aligned}$$

$K 4 stx [ ] x_{1,1} x_{2,2}^2 y_{1,1}^2 y_{2,2} C 8 stx [ ] x_{1,1} x_{2,2}^2 y_{1,1}^2 y_{2,2} K 8 stx [ ]$   
 $x_{1,2}^3 y_{1,2} y_{2,2} C 8 stx [ ] x_{1,2}^2 x_{2,2} y_{1,1}^2 y_{2,2} C 8 stx [ ] x_{1,2}^2 x_{2,2} y_{1,2} y_{2,2} y_{1,1} y_{2,2}$   
 $K 8 stx [ ] x_{1,2} x_{2,2}^2 y_{1,1}^2 y_{2,2} K 2 stx [ ] x_{1,2} x_{2,2}^2 y_{1,2} y_{2,2}^2 C 2 stx [ ] x_{2,2}^3 y_{1,1}^2 y_{2,2}^2$   
 $C 2 stx_1 x_2 x_{1,1}^2 y [ ] y_{1,2} y_{2,2}^2 K 8 stx_1 x_2 x_{1,1} x_{1,2} y [ ] y_{1,2}^2 y_{2,2}$   
 $K 4 stx_1 x_2 x_{1,1} x_{2,2} y [ ] y_{1,1} y_{1,2} y_{2,2} C 8 stx_1 x_2 x_{1,1} x_{2,2} y [ ] y_{1,2}^3 C 8 stx_1 x_2$   
 $x_{1,2}^2 y [ ] y_{1,1} y_{1,2} y_{2,2} K 8 stx_1 x_2 x_{1,2} x_{2,2} y [ ] y_{1,1} y_{1,2}^2 C 2 stx_1 x_2 x_{2,2}^2 y [ ] y_{1,1}^2 y_{1,2}$   
 $K 4 stx_1 x_{1,1}^2 x_{1,2} y [ ] y_{2,2}^2 C 2 stx_1 x_{1,1}^2 x_{2,2} y [ ] y_{1,2}^2 C 2 stx_1 x_{1,1}^2 y [ ] y_{1,2} y_{2,2}$   
 $y_{2,2}^2 K 2 stx_1 x_{1,1}^2 y [ ] y_{2,2} y_{1,1} y_{2,2}^2 C 16 stx_1 x_{1,1} x_{1,2}^2 y [ ] y_{2,2} y_{1,2} y_{2,2}$   
 $K 8 stx_1 x_{1,1} x_{1,2} x_{2,2} y [ ] y_{1,2} y_{1,2} y_{2,2} C 8 stx_1 x_{1,1} x_{1,2} x_{2,2} y [ ] y_{2,2} y_{1,1} y_{2,2}$   
 $K 16 stx_1 x_{1,1} x_{1,2} x_{2,2} y [ ] y_{2,2} y_{1,2}^2 K 8 stx_1 x_{1,1} x_{1,2} y [ ] y_{1,2} y_{1,2}^2 y_{2,2}$   
 $C 8 stx_1 x_{1,1} x_{1,2} y [ ] y_{2,2} y_{1,1} y_{1,2} y_{2,2} K 4 stx_1 x_{1,1} x_{2,2}^2 y [ ] y_{1,2} y_{1,1} y_{2,2}$   
 $C 8 stx_1 x_{1,1} x_{2,2}^2 y [ ] y_{1,2} y_{1,2}^2 K 4 stx_1 x_{1,1} x_{2,2} y [ ] y_{1,2} y_{1,1} y_{1,2} y_{2,2}$   
 $C 8 stx_1 x_{1,1} x_{2,2} y [ ] y_{1,2} y_{1,2}^3 C 4 stx_1 x_{1,1} x_{2,2} y [ ] y_{2,2} y_{1,1} y_{2,2}$   
 $K 8 stx_1 x_{1,1} x_{2,2} y [ ] y_{2,2} y_{1,1} y_{1,2}^2 K 16 stx_1 x_{1,2}^3 y [ ] y_{2,2} y_{1,1} y_{2,2} C 8 stx_1$   
 $x_{1,2}^2 x_{2,2} y [ ] y_{1,2} y_{1,1} y_{2,2} C 16 stx_1 x_{1,2}^2 x_{2,2} y [ ] y_{2,2} y_{1,1} y_{1,2} C 8 stx_1$   
 $x_{1,2}^2 y [ ] y_{1,2} y_{1,1} y_{1,2} y_{2,2} K 8 stx_1 x_{1,2}^2 y [ ] y_{2,2} y_{1,1} y_{2,2} K 8 stx_1 x_{1,2}$   
 $x_{2,2}^2 y [ ] y_{1,2} y_{1,1} y_{1,2} K 4 stx_1 x_{1,2} x_{2,2}^2 y [ ] y_{2,2} y_{1,1}^2 K 8 stx_1 x_{1,2} x_{2,2} y [ ] y_{1,2} y_{1,1} y_{1,2}^2$   
 $C 8 stx_1 x_{1,2} x_{2,2} y [ ] y_{2,2} y_{1,1} y_{1,2} C 2 stx_1 x_{2,2}^3 y [ ] y_{1,2} y_{1,1}^2 C 2 stx_1 x_{2,2}^2 y [ ] y_{1,2}$   
 $y_{1,1} y_{1,2} K 2 stx_1 x_{2,2}^2 y [ ] y_{2,2} y_{1,1}^3 K 2 stx_2^2 x_{1,1}^2 y [ ] y_{1,1} y_{1,2}^2 C 8 st$   
 $x_2^2 x_{1,1} x_{1,2} y [ ] y_{1,1} y_{1,2} y_{2,2} C 4 stx_2^2 x_{1,1} x_{2,2} y [ ] y_{1,1}^2 y_{2,2} K 8 st$   
 $x_2^2 x_{1,1} x_{2,2} y [ ] y_{1,1} y_{1,2}^2 K 8 stx_2^2 x_{1,2}^2 y [ ] y_{1,1}^2 y_{2,2} C 8 stx_2^2 x_{1,2} x_{2,2} y [ ] y_{1,1}^2 y_{1,2}$   
 $K 2 stx_2^2 x_{2,2}^2 y [ ] y_{1,1}^3 C 4 stx_2 x_{1,1}^3 y [ ] y_{2,2} y_{2,2}^2 K 2 stx_2 x_{1,1}^2 x_{1,2} y [ ] y_{1,2} y_{2,2}^2$   
 $K 16 stx_2 x_{1,1}^2 x_{1,2} y [ ] y_{2,2} y_{1,2} y_{2,2} K 8 stx_2 x_{1,1}^2 x_{2,2} y [ ] y_{2,2} y_{1,1} y_{2,2} C 16 stx_2$   
 $x_{1,1}^2 x_{2,2} y [ ] y_{2,2} y_{1,2}^2 C 8 stx_2 x_{1,1} x_{1,2}^2 y [ ] y_{1,2} y_{1,2} y_{2,2} C 16 stx_2 x_{1,1}$   
 $x_{1,2}^2 y [ ] y_{2,2} y_{1,1} y_{2,2} C 4 stx_2 x_{1,1} x_{1,2} x_{2,2} y [ ] y_{1,2} y_{1,1} y_{2,2}$   
 $K 8 stx_2 x_{1,1} x_{1,2} x_{2,2} y [ ] y_{1,2} y_{1,2}^2 K 16 stx_2 x_{1,1} x_{1,2} x_{2,2} y [ ] y_{2,2} y_{1,1} y_{1,2}$   
 $C 4 stx_2 x_{1,1} x_{2,2}^2 y [ ] y_{2,2} y_{1,1}^2 K 8 stx_2 x_{1,2}^3 y [ ] y_{1,2} y_{1,1} y_{2,2} C 8 stx_2$   
 $x_{1,2}^2 x_{2,2} y [ ] y_{1,2} y_{1,1} y_{1,2} K 2 stx_2 x_{1,2} x_{2,2}^2 y [ ] y_{1,2} y_{1,1}^2 C 2 stx_2^3 y [ ] y_{1,2} y_{2,2}^2$   
 $K 2 stx_2^2 x_{1,1} x_{1,2} y [ ] y_{1,2} y_{2,2}^2 K 8 stx_2^2 x_{1,1} x_{1,2} y [ ] y_{1,2} y_{2,2} y_{1,2} y_{2,2} K 4 st$   
 $x_{1,1}^2 x_{2,2} y [ ] y_{1,2} y_{2,2} y_{1,1} y_{2,2} C 8 stx_2^2 x_{1,1} x_{2,2} y [ ] y_{1,2} y_{2,2} y_{1,2}^2 C 8 stx_2 x_{1,1} x_{1,2}^2 y [ ]$   
 $y_{1,2} y_{1,2} y_{2,2} C 8 stx_2 x_{1,1} x_{1,2}^2 y [ ] y_{1,2} y_{2,2} y_{1,1} y_{2,2} C 4 stx_2 x_{1,1} x_{1,2} x_{2,2} y [ ] y_{1,2} y_{1,1} y_{2,2}$   
 $K 8 stx_2 x_{1,1} x_{1,2} x_{2,2} y [ ] y_{1,2} y_{1,2}^2 K 8 stx_2 x_{1,1} x_{1,2} x_{2,2} y [ ] y_{1,2} y_{2,2} y_{1,1} y_{1,2} C 2 stx_2 x_{1,1}$

$$\begin{aligned}
& x_{2,2}^2 y [ ] y_1 y_2 y_{1,1}^2 K 8 s t x_{1,2}^3 y [ ] y_1^2 y_{1,1} y_2 C 8 s t x_{1,2}^2 x_{2,2} y [ ] y_1^2 y_{1,1} y_1, 2 \\
& K 2 s t x_{1,2} x_{2,2}^2 y [ ] y_1^2 y_{1,1}^2 K 3 t^2 x [ ] x_1^2 x_{1,1}^2 y_{2,2}^3 C 12 t^2 x [ ] x_1^2 x_{1,1} x_{1,2} y_{1,2} y_{2,2}^2 \\
& C 6 t^2 x [ ] x_1^2 x_{1,1} x_{2,2} y_{1,1} y_{2,2}^2 K 12 t^2 x [ ] x_1^2 x_{1,1} x_{2,2} y_{1,2} y_{2,2} K 12 t^2 x [ ] x_1^2 \\
& x_{1,2}^2 y_{1,1} y_{2,2}^2 C 12 t^2 x [ ] x_1^2 x_{1,2} x_{2,2} y_{1,1} y_{1,2} y_{2,2} K 3 t^2 x [ ] x_1^2 x_{2,2}^2 y_{1,1} y_2, 2 \\
& C 4 t^2 x [ ] x_1 x_2 x_{1,1}^2 y_{1,2} y_{2,2}^2 K 16 t^2 x [ ] x_1 x_2 x_{1,1} x_{1,2} y_{1,2} y_{2,2} \\
& K 8 t^2 x [ ] x_1 x_2 x_{1,1} x_{2,2} y_{1,1} y_{1,2} y_{2,2} C 16 t^2 x [ ] x_1 x_2 x_{1,1} x_{2,2} y_{1,2}^3 C 16 t^2 x [ ] x_1 x_2 \\
& x_{1,2}^2 y_{1,1} y_{1,2} y_{2,2} K 16 t^2 x [ ] x_1 x_2 x_{1,2} x_{2,2} y_{1,1} y_{1,2}^2 C 4 t^2 x [ ] x_1 x_2 x_{2,2}^2 y_{1,1} y_1, 2 \\
& C 2 t^2 x [ ] x_1 x_{1,1}^2 x_{2,2} y_1 y_{2,2}^2 K 8 t^2 x [ ] x_1 x_{1,1} x_{1,2} x_{2,2} y_1 y_{1,2} y_{2,2} K 4 t^2 x [ ] x_1 x_{1,1} \\
& x_{2,2}^2 y_1 y_{1,1} y_2, 2 C 8 t^2 x [ ] x_1 x_{1,1} x_{2,2}^2 y_1 y_{1,2}^2 C 8 t^2 x [ ] x_1 x_{1,2} x_{2,2} y_1 y_{1,1} y_2, 2 \\
& K 8 t^2 x [ ] x_1 x_{1,2} x_{2,2}^2 y_1 y_{1,1} y_2 C 2 t^2 x [ ] x_1 x_{2,2}^3 y_1 y_{1,1}^2 K t^2 x [ ] x_{2,2}^2 x_{1,1}^2 y_{1,1} y_{2,2}^2 \\
& C 4 t^2 x [ ] x_{2,2}^2 x_{1,1} x_{1,2} y_{1,1} y_{1,2} y_{2,2} C 2 t^2 x [ ] x_{2,2}^2 x_{1,1} x_{2,2} y_{1,1} y_2, 2 K 4 t^2 x [ ] \\
& x_{2,2}^2 x_{1,1} x_{2,2} y_{1,1} y_{1,2}^2 K 4 t^2 x [ ] x_{2,2}^2 x_{1,2}^2 y_{1,1} y_2, 2 C 4 t^2 x [ ] x_{2,2}^2 x_{1,2} x_{2,2} y_{1,1} y_1, 2 \\
& K t^2 x [ ] x_{2,2}^2 x_{2,2}^2 y_{1,1}^3 K 2 t^2 x [ ] x_{2,2} x_{1,1}^2 x_{1,2} y_1 y_{2,2}^2 C 8 t^2 x [ ] x_{2,2} x_{1,1} x_{1,2}^2 y_1 y_{1,2} y_{2,2} \\
& C 4 t^2 x [ ] x_{2,2} x_{1,1} x_{1,2} x_{2,2} y_1 y_{1,1} y_2, 2 K 8 t^2 x [ ] x_{2,2} x_{1,1} x_{1,2} x_{2,2} y_1 y_{1,2}^2 K 8 t^2 x [ ] x_{2,2} \\
& x_{1,2}^3 y_1 y_{1,1} y_2, 2 C 8 t^2 x [ ] x_{2,2} x_{1,2}^2 x_{2,2} y_1 y_{1,1} y_2 K 2 t^2 x [ ] x_{2,2} x_{1,2} x_{2,2}^2 y_1 y_{1,1}^2 C t^2 x_{1,1}^2 \\
& x_{1,1}^2 x_{2,2} y [ ] y_{2,2}^2 C 2 t^2 x_{1,1}^2 x_{1,1} y [ ] y_{1,2} y_{2,2}^2 K 4 t^2 x_{1,1}^2 x_{1,1} x_{1,2} x_{2,2} y [ ] y_{1,2} y_{2,2} K 8 t^2 \\
& x_{1,1}^2 x_{1,1} x_{1,2} y [ ] y_{1,2} y_{2,2} K 2 t^2 x_{1,1}^2 x_{1,1} x_{2,2} y [ ] y_{1,1} y_2, 2 C 4 t^2 x_{1,1}^2 x_{1,1} x_{2,2} y [ ] y_{1,2}^2 \\
& K 4 t^2 x_{1,1}^2 x_{1,1} x_{2,2} y [ ] y_{1,1} y_{1,2} y_{2,2} C 8 t^2 x_{1,1}^2 x_{1,1} x_{2,2} y [ ] y_{1,2}^3 C 4 t^2 x_{1,1}^2 \\
& x_{1,2}^2 x_{2,2} y [ ] y_{1,1} y_2, 2 C 8 t^2 x_{1,1}^2 x_{1,2}^2 y [ ] y_{1,1} y_{1,2} y_{2,2} K 4 t^2 x_{1,1}^2 x_{1,2} x_{2,2}^2 y [ ] y_{1,1} y_1, 2 \\
& K 8 t^2 x_{1,1}^2 x_{1,2} x_{2,2} y [ ] y_{1,1} y_{1,2}^2 C t^2 x_{1,1}^2 x_{2,2}^3 y [ ] y_{1,1}^2 C 2 t^2 x_{1,1}^2 x_{2,2}^2 y [ ] y_{1,1}^2 y_1, 2 \\
& K 2 t^2 x_1 x_2 x_{1,1}^2 x_{1,2} y [ ] y_{2,2}^2 K 2 t^2 x_1 x_2 x_{1,1}^2 y [ ] y_{1,1} y_{2,2}^2 C 8 t^2 x_1 x_2 x_{1,1} \\
& x_{1,2}^2 y [ ] y_{1,2} y_{2,2} C 4 t^2 x_1 x_2 x_{1,1} x_{1,2} x_{2,2} y [ ] y_{1,1} y_2, 2 K 8 t^2 x_1 x_2 x_{1,1} x_{1,2} x_{2,2} y [ ] \\
& y_{1,2}^2 C 8 t^2 x_1 x_2 x_{1,1} x_{1,2} y [ ] y_{1,1} y_{1,2} y_{2,2} C 4 t^2 x_1 x_2 x_{1,1} x_{2,2} y [ ] y_{1,1}^2 y_2, 2 \\
& K 8 t^2 x_1 x_2 x_{1,1} x_{2,2} y [ ] y_{1,1} y_{1,2}^2 K 8 t^2 x_1 x_2 x_{1,2}^3 y [ ] y_{1,1} y_2, 2 C 8 t^2 x_1 x_2 \\
& x_{1,2}^2 x_{2,2} y [ ] y_{1,1} y_1, 2 K 8 t^2 x_1 x_2 x_{1,2}^2 y [ ] y_{1,1}^2 y_2, 2 K 2 t^2 x_1 x_2 x_{1,2} x_{2,2}^2 y [ ] y_{1,1}^2 \\
& C 8 t^2 x_1 x_2 x_{1,2} x_{2,2} y [ ] y_{1,1}^2 y_1, 2 K 2 t^2 x_1 x_2 x_{2,2}^2 y [ ] y_{1,1}^3 K 2 t^2 x_1 x_{1,1}^2 x_{1,2} y [ ] y_1 \\
& y_{2,2}^2 C 8 t^2 x_1 x_{1,1} x_{1,2}^2 y [ ] y_1 y_{1,2} y_{2,2} C 4 t^2 x_1 x_{1,1} x_{1,2} x_{2,2} y [ ] y_1 y_{1,1} y_2, 2 \\
& K 8 t^2 x_1 x_{1,1} x_{1,2} x_{2,2} y [ ] y_1 y_{1,2}^2 K 8 t^2 x_1 x_{1,2}^3 y [ ] y_1 y_{1,1} y_2, 2 C 8 t^2 x_1 \\
& x_{1,2}^2 x_{2,2} y [ ] y_1 y_{1,1} y_1, 2 K 2 t^2 x_1 x_{1,2} x_{2,2}^2 y [ ] y_1 y_{1,1}^2 C t^2 x_{1,1}^2 x_{1,1}^3 y [ ] y_{2,2}^2 K 4 t^2 x_{1,1}^2 \\
& x_{1,1}^2 x_{1,2} y [ ] y_{1,2} y_{2,2} K 2 t^2 x_{1,1}^2 x_{1,1} x_{2,2} y [ ] y_{1,1} y_2, 2 C 4 t^2 x_{1,1}^2 x_{1,1}^2 x_{2,2} y [ ] y_{1,2}^2 C 4 t^2 \\
& x_{2,2}^2 x_{1,1} x_{1,2}^2 y [ ] y_{1,1} y_2, 2 K 4 t^2 x_{2,2}^2 x_{1,1} x_{1,2} x_{2,2} y [ ] y_{1,1} y_1, 2 C t^2 x_{2,2}^2 x_{1,1} x_{2,2}^2 y [ ] y_{1,1}^2 \\
& C 2 t^2 x_{2,2}^3 x_{1,1} y [ ] y_1 y_{2,2}^2 K 8 t^2 x_{2,2}^2 x_{1,1} x_{1,2} y [ ] y_1 y_{1,2} y_{2,2} K 4 t^2 x_{2,2}
\end{aligned}$$

$$\begin{aligned}
& x_{1,1}^2 x_{2,2} y [ ] y_1 y_{1,1} y_{2,2} \text{C} 8 t^2 x_2 x_{1,1}^2 x_{2,2} y [ ] y_1 y_{1,1}^2 \text{C} 8 t^2 x_2 x_{1,1} x_{1,2}^2 y [ ] y_1 y_{1,1} y_{2,2} \\
& \text{K} 8 t^2 x_2 x_{1,1} x_{1,2} x_{2,2} y [ ] y_1 y_{1,1} y_{1,2} \text{C} 2 t^2 x_2 x_{1,1} x_{2,2}^2 y [ ] y_1 y_{1,1}^2 \text{C} s x [ ]^2 x_2 x_{1,1}^2 \\
& y_{2,2}^3 \text{K} 4 s x [ ]^2 x_2 x_{1,1} x_{1,2} y_{1,2} y_{2,2}^2 \text{K} 2 s x [ ]^2 x_2 x_{1,1} x_{2,2} y_{1,1} y_{2,2}^2 \\
& \text{C} 4 s x [ ]^2 x_2 x_{1,1} x_{2,2} y_{1,2} y_{2,2}^2 \text{C} 4 s x [ ]^2 x_2 x_{1,2}^2 y_{1,1} y_{2,2}^2 \\
& \text{K} 4 s x [ ]^2 x_2 x_{1,2} x_{2,2} y_{1,1} y_{1,2} y_{2,2} \text{C} s x [ ]^2 x_2 x_{2,2}^2 y_{1,1} y_{2,2}^2 \text{K} s x [ ]^2 x_{1,1}^2 x_{2,2} y_{2,2} y_{2,2}^2 \\
& \text{C} 2 s x [ ]^2 x_{1,1}^2 y_1 y_{2,2}^3 \text{K} 2 s x [ ]^2 x_{1,1}^2 y_2 y_{1,2} y_{2,2}^2 \text{C} 4 s x [ ]^2 x_{1,1} x_{1,2} x_{2,2} y_2 y_{1,2} y_{2,2} \\
& \text{K} 8 s x [ ]^2 x_{1,1} x_{1,2} y_1 y_{1,2} y_{2,2}^2 \text{C} 8 s x [ ]^2 x_{1,1} x_{1,2} y_2 y_{1,2} y_{2,2}^2 \text{C} 2 s x [ ]^2 x_{1,1} \\
& x_{2,2}^2 y_2 y_{1,1} y_{2,2} \text{K} 4 s x [ ]^2 x_{1,1} x_{2,2}^2 y_2 y_{1,2}^2 \text{K} 4 s x [ ]^2 x_{1,1} x_{2,2} y_1 y_{1,1} y_{2,2}^2 \\
& \text{C} 8 s x [ ]^2 x_{1,1} x_{2,2} y_1 y_{1,2} y_{2,2}^2 \text{C} 4 s x [ ]^2 x_{1,1} x_{2,2} y_2 y_{1,1} y_{1,2} y_{2,2} \\
& \text{K} 8 s x [ ]^2 x_{1,1} x_{2,2} y_2 y_{1,2}^3 \text{K} 4 s x [ ]^2 x_{1,2}^2 x_{2,2} y_2 y_{1,1} y_{2,2} \text{C} 8 s x [ ]^2 x_{1,2}^2 y_1 y_{1,1} y_{2,2}^2 \\
& \text{K} 8 s x [ ]^2 x_{1,2}^2 y_2 y_{1,1} y_{1,2} y_{2,2} \text{C} 4 s x [ ]^2 x_{1,2} x_{2,2}^2 y_2 y_{1,1} y_{1,2} \\
& \text{K} 8 s x [ ]^2 x_{1,2} x_{2,2} y_1 y_{1,1} y_{1,2} y_{2,2} \text{C} 8 s x [ ]^2 x_{1,2} x_{2,2} y_2 y_{1,1} y_{1,2}^2 \text{K} s x [ ]^2 x_{2,2}^3 y_2 \\
& y_{1,1}^2 \text{C} 2 s x [ ]^2 x_{2,2}^2 y_1 y_{1,1}^2 y_{2,2} \text{K} 2 s x [ ]^2 x_{2,2}^2 y_2 y_{1,1}^2 y_{2,2} \text{K} 2 s x [ ] x_2 x_{1,1}^2 y [ ] y_1, 2 \\
& y_{2,2}^2 \text{C} 8 s x [ ] x_2 x_{1,1} x_{1,2} y [ ] y_{1,2}^2 y_{2,2} \text{C} 4 s x [ ] x_2 x_{1,1} x_{2,2} y [ ] y_{1,1} y_{1,2} y_{2,2} \\
& \text{K} 8 s x [ ] x_2 x_{1,1} x_{2,2} y [ ] y_{1,2}^3 \text{K} 8 s x [ ] x_2 x_{1,2}^2 y [ ] y_{1,1} y_{1,2} y_{2,2} \\
& \text{C} 8 s x [ ] x_2 x_{1,2} x_{2,2} y [ ] y_{1,1} y_{1,2}^2 \text{K} 2 s x [ ] x_2 x_{2,2}^2 y [ ] y_{1,1}^2 y_{1,2} \text{C} 4 s x [ ] \\
& x_{1,1}^2 x_{1,2} y [ ] y_2 y_{2,2}^2 \text{K} 2 s x [ ] x_{1,1}^2 x_{2,2} y [ ] y_1 y_{2,2}^2 \text{K} 2 s x [ ] x_{1,1}^2 y [ ] y_1 y_{1,2} y_{2,2}^2 \\
& \text{C} 2 s x [ ] x_{1,1}^2 y [ ] y_2 y_{1,1} y_{2,2}^2 \text{K} 16 s x [ ] x_{1,1} x_{1,2}^2 y [ ] y_2 y_{1,2} y_{2,2} \\
& \text{C} 8 s x [ ] x_{1,1} x_{1,2} x_{2,2} y [ ] y_1 y_{1,2} y_{2,2} \text{K} 8 s x [ ] x_{1,1} x_{1,2} x_{2,2} y [ ] y_2 y_{1,1} y_{2,2} \\
& \text{C} 16 s x [ ] x_{1,1} x_{1,2} x_{2,2} y [ ] y_2 y_{1,2}^2 \text{C} 8 s x [ ] x_{1,1} x_{1,2} y [ ] y_1 y_{1,2}^2 y_{2,2} \\
& \text{K} 8 s x [ ] x_{1,1} x_{1,2} y [ ] y_2 y_{1,1} y_{1,2} y_{2,2} \text{C} 4 s x [ ] x_{1,1} x_{2,2}^2 y [ ] y_1 y_{1,1} y_{2,2} \\
& \text{K} 8 s x [ ] x_{1,1} x_{2,2}^2 y [ ] y_1 y_{1,2}^2 \text{C} 4 s x [ ] x_{1,1} x_{2,2} y [ ] y_1 y_{1,1} y_{1,2} y_{2,2} \\
& \text{K} 8 s x [ ] x_{1,1} x_{2,2} y [ ] y_1 y_{1,2}^3 \text{K} 4 s x [ ] x_{1,1} x_{2,2} y [ ] y_2 y_{1,1}^2 y_{2,2} \\
& \text{C} 8 s x [ ] x_{1,1} x_{2,2} y [ ] y_2 y_{1,1} y_{1,2}^2 \text{C} 16 s x [ ] x_{1,2}^3 y [ ] y_2 y_{1,1} y_{2,2} \text{K} 8 s x [ ] \\
& x_{1,2}^2 x_{2,2} y [ ] y_1 y_{1,1} y_{2,2} \text{K} 16 s x [ ] x_{1,2}^2 x_{2,2} y [ ] y_2 y_{1,1} y_{1,2} \text{K} 8 s x [ ] \\
& x_{1,2}^2 y [ ] y_1 y_{1,1} y_{1,2} y_{2,2} \text{C} 8 s x [ ] x_{1,2}^2 y [ ] y_2 y_{1,1}^2 y_{2,2} \text{C} 8 s x [ ] x_{1,2} \\
& x_{2,2}^2 y [ ] y_1 y_{1,1} y_{1,2} \text{C} 4 s x [ ] x_{1,2} x_{2,2}^2 y [ ] y_2 y_{1,1}^2 \text{C} 8 s x [ ] x_{1,2} x_{2,2} y [ ] y_1 y_{1,1} y_{1,2}^2 \\
& \text{K} 8 s x [ ] x_{1,2} x_{2,2} y [ ] y_2 y_{1,1}^2 y_{1,2} \text{K} 2 s x [ ] x_{2,2}^3 y [ ] y_1 y_{1,1}^2 \text{K} 2 s x [ ] x_{2,2}^2 y [ ] y_1 \\
& y_{1,1}^2 y_{1,2} \text{C} 2 s x [ ] x_{2,2}^2 y [ ] y_2 y_{1,1}^3 \text{C} s x_2 x_{1,1}^2 y [ ]^2 y_{1,1} y_{2,2}^2 \\
& \text{K} 4 s x_2 x_{1,1} x_{1,2} y [ ]^2 y_{1,1} y_{1,2} y_{2,2} \text{K} 2 s x_2 x_{1,1} x_{2,2} y [ ]^2 y_{1,1}^2 y_{2,2} \\
& \text{C} 4 s x_2 x_{1,1} x_{2,2} y [ ]^2 y_{1,1} y_{1,2}^2 \text{C} 4 s x_2 x_{1,2}^2 y [ ]^2 y_{1,1}^2 y_{2,2} \text{K} 4 s x_2 x_{1,2} x_{2,2} y [ ]^2 \\
& y_{1,1}^2 y_{1,2} \text{C} s x_2 x_{2,2}^2 y [ ]^2 y_{1,1}^3 \text{K} 3 s x_{1,1}^3 y [ ]^2 y_2 y_{2,2}^2 \text{C} 2 s x_{1,1}^2 x_{1,2} y [ ]^2 y_1 y_{2,2}^2 \text{C} 12 s
\end{aligned}$$

$$\begin{aligned}
& x_{1,1}^2 x_{1,2} y [ ]^2 y_2 y_{1,2} y_{2,2} \mathbf{C} 6 s x_{1,1}^2 x_{2,2} y [ ]^2 y_2 y_{1,1} y_{2,2} \mathbf{K} 12 s x_{1,1}^2 x_{2,2} y [ ]^2 y_2 y_{1,2}^2 \\
& \mathbf{K} 8 s x_{1,1} x_{1,2}^2 y [ ]^2 y_1 y_{1,2} y_{2,2} \mathbf{K} 12 s x_{1,1} x_{1,2}^2 y [ ]^2 y_2 y_{1,1} y_{2,2} \\
& \mathbf{K} 4 s x_{1,1} x_{1,2} x_{2,2} y [ ]^2 y_1 y_{1,1} y_{2,2} \mathbf{C} 8 s x_{1,1} x_{1,2} x_{2,2} y [ ]^2 y_1 y_{1,2}^2 \\
& \mathbf{C} 12 s x_{1,1} x_{1,2} x_{2,2} y [ ]^2 y_2 y_{1,1} y_{1,2} \mathbf{K} 3 s x_{1,1} x_{2,2}^2 y [ ]^2 y_2 y_{1,1}^2 \mathbf{C} 8 s \\
& x_{1,2}^3 y [ ]^2 y_1 y_{1,1} y_{2,2} \mathbf{K} 8 s x_{1,2}^2 x_{2,2} y [ ]^2 y_1 y_{1,1} y_{1,2} \mathbf{C} 2 s x_{1,2} x_{2,2}^2 y [ ]^2 y_1 y_{1,1}^2 \\
& \mathbf{C} 3 t x [ ]^2 x_1 x_{1,1}^2 y_{2,2}^3 \mathbf{K} 12 t x [ ]^2 x_1 x_{1,1} x_{1,2} y_{1,2} y_{2,2}^2 \mathbf{K} 6 t x [ ]^2 x_1 x_{1,1} x_{2,2} y_{1,1} y_{2,2}^2 \\
& \mathbf{C} 12 t x [ ]^2 x_1 x_{1,1} x_{2,2} y_{1,2}^2 y_{2,2} \mathbf{C} 12 t x [ ]^2 x_1 x_{1,2}^2 y_{1,1} y_{2,2}^2 \\
& \mathbf{K} 12 t x [ ]^2 x_1 x_{1,2} x_{2,2} y_{1,1} y_{1,2} y_{2,2} \mathbf{C} 3 t x [ ]^2 x_1 x_{2,2}^2 y_{1,1} y_{2,2} \mathbf{K} 2 t x [ ]^2 x_2 x_{1,1}^2 y_{1,2} \\
& y_{2,2}^2 \mathbf{C} 8 t x [ ]^2 x_2 x_{1,1} x_{1,2} y_{1,2}^2 y_{2,2} \mathbf{C} 4 t x [ ]^2 x_2 x_{1,1} x_{2,2} y_{1,1} y_{1,2} y_{2,2} \\
& \mathbf{K} 8 t x [ ]^2 x_2 x_{1,1} x_{2,2} y_{1,2}^3 \mathbf{K} 8 t x [ ]^2 x_2 x_{1,2}^2 y_{1,1} y_{1,2} y_{2,2} \mathbf{C} 8 t x [ ]^2 x_2 x_{1,2} x_{2,2} y_{1,1} \\
& y_{1,2}^2 \mathbf{K} 2 t x [ ]^2 x_2 x_{2,2}^2 y_{1,1} y_{1,2} \mathbf{K} t x [ ]^2 x_{1,1}^2 x_{2,2} y_{1,2} y_{2,2}^2 \\
& \mathbf{C} 4 t x [ ]^2 x_{1,1} x_{1,2} x_{2,2} y_{1,1} y_{1,2} y_{2,2} \mathbf{C} 2 t x [ ]^2 x_{1,1} x_{2,2}^2 y_{1,1} y_{1,2} y_{2,2} \mathbf{K} 4 t x [ ]^2 x_{1,1} \\
& x_{2,2}^2 y_{1,1} y_{1,2}^2 \mathbf{K} 4 t x [ ]^2 x_{1,2}^2 x_{2,2} y_{1,1} y_{1,2} y_{2,2} \mathbf{C} 4 t x [ ]^2 x_{1,2} x_{2,2}^2 y_{1,1} y_{1,2} \mathbf{K} t x [ ]^2 \\
& x_{2,2}^3 y_{1,1} y_{1,2}^2 \mathbf{K} 2 t x [ ] x_1 x_{1,1}^2 x_{2,2} y [ ] y_{2,2}^2 \mathbf{K} 4 t x [ ] x_1 x_{1,1}^2 y [ ] y_{1,2} y_{2,2}^2 \\
& \mathbf{C} 8 t x [ ] x_1 x_{1,1} x_{1,2} x_{2,2} y [ ] y_{1,2} y_{2,2} \mathbf{C} 16 t x [ ] x_1 x_{1,1} x_{1,2} y [ ] y_{1,2}^2 y_{2,2} \\
& \mathbf{C} 4 t x [ ] x_1 x_{1,1} x_{2,2}^2 y [ ] y_{1,1} y_{2,2} \mathbf{K} 8 t x [ ] x_1 x_{1,1} x_{2,2}^2 y [ ] y_{1,2}^2 \\
& \mathbf{C} 8 t x [ ] x_1 x_{1,1} x_{2,2} y [ ] y_{1,1} y_{1,2} y_{2,2} \mathbf{K} 16 t x [ ] x_1 x_{1,1} x_{2,2} y [ ] y_{1,2}^3 \mathbf{K} 8 t x [ ] x_1 \\
& x_{1,2}^2 x_{2,2} y [ ] y_{1,1} y_{2,2} \mathbf{K} 16 t x [ ] x_1 x_{1,2}^2 y [ ] y_{1,1} y_{1,2} y_{2,2} \mathbf{C} 8 t x [ ] x_1 x_{1,2} \\
& x_{2,2}^2 y [ ] y_{1,1} y_{1,2} \mathbf{C} 16 t x [ ] x_1 x_{1,2} x_{2,2} y [ ] y_{1,1} y_{1,2}^2 \mathbf{K} 2 t x [ ] x_1 x_{2,2}^3 y [ ] y_{1,1}^2 \\
& \mathbf{K} 4 t x [ ] x_1 x_{2,2}^2 y [ ] y_{1,1} y_{1,2} \mathbf{C} 2 t x [ ] x_2 x_{1,1}^2 x_{1,2} y [ ] y_{2,2}^2 \mathbf{C} 2 t x [ ] x_2 \\
& x_{1,1}^2 y [ ] y_{1,1} y_{2,2}^2 \mathbf{K} 8 t x [ ] x_2 x_{1,1} x_{1,2}^2 y [ ] y_{1,2} y_{2,2} \\
& \mathbf{K} 4 t x [ ] x_2 x_{1,1} x_{1,2} x_{2,2} y [ ] y_{1,1} y_{2,2} \mathbf{C} 8 t x [ ] x_2 x_{1,1} x_{1,2} x_{2,2} y [ ] y_{1,2}^2 \\
& \mathbf{K} 8 t x [ ] x_2 x_{1,1} x_{1,2} y [ ] y_{1,1} y_{1,2} y_{2,2} \mathbf{K} 4 t x [ ] x_2 x_{1,1} x_{2,2} y [ ] y_{1,1} y_{2,2} \\
& \mathbf{C} 8 t x [ ] x_2 x_{1,1} x_{2,2} y [ ] y_{1,1} y_{1,2}^2 \mathbf{C} 8 t x [ ] x_2 x_{1,2}^3 y [ ] y_{1,1} y_{2,2} \mathbf{K} 8 t x [ ] x_2 \\
& x_{1,2}^2 x_{2,2} y [ ] y_{1,1} y_{1,2} \mathbf{C} 8 t x [ ] x_2 x_{1,2}^2 y [ ] y_{1,1} y_{2,2} \mathbf{C} 2 t x [ ] x_2 x_{1,2} x_{2,2}^2 y [ ] y_{1,1}^2 \\
& \mathbf{K} 8 t x [ ] x_2 x_{1,2} x_{2,2} y [ ] y_{1,1} y_{1,2} \mathbf{C} 2 t x [ ] x_2 x_{2,2}^2 y [ ] y_{1,1}^3 \mathbf{C} 2 t x [ ] \\
& x_{1,1}^2 x_{1,2} y [ ] y_{1,1} y_{2,2}^2 \mathbf{K} 8 t x [ ] x_{1,1} x_{1,2}^2 y [ ] y_{1,1} y_{1,2} y_{2,2} \\
& \mathbf{K} 4 t x [ ] x_{1,1} x_{1,2} x_{2,2} y [ ] y_{1,1} y_{1,2} y_{2,2} \mathbf{C} 8 t x [ ] x_{1,1} x_{1,2} x_{2,2} y [ ] y_{1,1} y_{1,2}^2 \mathbf{C} 8 t x [ ] \\
& x_{1,2}^3 y [ ] y_{1,1} y_{1,2} y_{2,2} \mathbf{K} 8 t x [ ] x_{1,2}^2 x_{2,2} y [ ] y_{1,1} y_{1,2} y_{1,2} \mathbf{C} 2 t x [ ] x_{1,2} x_{2,2}^2 y [ ] y_{1,1} y_{1,1}^2 \\
& \mathbf{C} 2 t x x_{1,1} x_{1,2} y [ ]^2 y_{2,2}^2 \mathbf{C} t x x_{1,1}^2 y [ ]^2 y_{1,1} y_{2,2}^2 \mathbf{K} 8 t x x_{1,1} x_{1,2}^2 y [ ]^2 y_{1,2} y_{2,2} \\
& \mathbf{K} 4 t x x_{1,1} x_{1,2} x_{2,2} y [ ]^2 y_{1,1} y_{2,2} \mathbf{C} 8 t x x_{1,1} x_{1,2} x_{2,2} y [ ]^2 y_{1,2}^2 \\
& \mathbf{K} 4 t x x_{1,1} x_{1,2} y [ ]^2 y_{1,1} y_{1,2} y_{2,2} \mathbf{K} 2 t x x_{1,1} x_{2,2} y [ ]^2 y_{1,1} y_{2,2}
\end{aligned}$$

$$\begin{aligned}
& C4tx_1x_{1,1}x_{2,2}y[\ ]^2y_{1,1}y_{1,2}^2C8tx_1x_{1,2}^3y[\ ]^2y_{1,1}y_{2,2}K8tx_1 \\
& x_{1,2}^2x_{2,2}y[\ ]^2y_{1,1}y_{1,2}C4tx_1x_{1,2}^2y[\ ]^2y_{1,1}y_{2,2}C2tx_1x_{1,2}x_{2,2}^2y[\ ]^2y_{1,1}^2 \\
& K4tx_1x_{1,2}x_{2,2}y[\ ]^2y_{1,1}^2y_{1,2}Ctx_1x_{2,2}^2y[\ ]^2y_{1,1}^3K2tx_2x_{1,1}^3y[\ ]^2y_{2,2}^2C8tx_2 \\
& x_{1,1}^2x_{1,2}y[\ ]^2y_{1,2}y_{2,2}C4tx_2x_{1,1}^2x_{2,2}y[\ ]^2y_{1,1}y_{2,2}K8tx_2x_{1,1}^2x_{2,2}y[\ ]^2y_{1,2}^2 \\
& K8tx_2x_{1,1}x_{1,2}^2y[\ ]^2y_{1,1}y_{2,2}C8tx_2x_{1,1}x_{1,2}x_{2,2}y[\ ]^2y_{1,1}y_{1,2}K2tx_2x_{1,1} \\
& x_{2,2}^2y[\ ]^2y_{1,1}^2Ktx_1^3y[\ ]^2y_{1,1}y_{2,2}^2C4tx_1^2x_{1,2}y[\ ]^2y_{1,1}y_{1,2}y_{2,2}C2t \\
& x_{1,1}^2x_{2,2}y[\ ]^2y_{1,1}y_{1,2}y_{2,2}K4tx_1^2x_{2,2}y[\ ]^2y_{1,1}y_{2,2}^2K4tx_{1,1}x_{1,2}^2y[\ ]^2y_{1,1}y_{1,2}y_{2,2} \\
& C4tx_{1,1}x_{1,2}x_{2,2}y[\ ]^2y_{1,1}y_{1,2}Ktx_{1,1}x_{2,2}^2y[\ ]^2y_{1,1}y_{1,2}^2Kx[\ ]^3x_{1,1}^2y_{2,2}^3 \\
& C4x[\ ]^3x_{1,1}x_{1,2}y_{1,2}y_{2,2}^2C2x[\ ]^3x_{1,1}x_{2,2}y_{1,1}y_{2,2}^2K4x[\ ]^3x_{1,1}x_{2,2}y_{1,2}y_{2,2} \\
& K4x[\ ]^3x_{1,2}^2y_{1,1}y_{2,2}^2C4x[\ ]^3x_{1,2}x_{2,2}y_{1,1}y_{1,2}y_{2,2}Kx[\ ]^3x_{2,2}^2y_{1,1}y_{2,2}^2Cx[\ ]^2 \\
& x_{1,1}^2x_{2,2}y[\ ]y_{2,2}^2C2x[\ ]^2x_{1,1}^2y[\ ]y_{1,2}y_{2,2}^2K4x[\ ]^2x_{1,1}x_{1,2}x_{2,2}y[\ ]y_{1,2}y_{2,2} \\
& K8x[\ ]^2x_{1,1}x_{1,2}y[\ ]y_{1,2}y_{2,2}^2K2x[\ ]^2x_{1,1}x_{2,2}^2y[\ ]y_{1,1}y_{2,2}C4x[\ ]^2x_{1,1} \\
& x_{2,2}^2y[\ ]y_{1,2}^2K4x[\ ]^2x_{1,1}x_{2,2}y[\ ]y_{1,1}y_{1,2}y_{2,2}C8x[\ ]^2x_{1,1}x_{2,2}y[\ ]y_{1,2}^3C4x[\ ]^2 \\
& x_{1,2}^2x_{2,2}y[\ ]y_{1,1}y_{2,2}C8x[\ ]^2x_{1,2}^2y[\ ]y_{1,1}y_{1,2}y_{2,2}K4x[\ ]^2x_{1,2}x_{2,2}^2y[\ ]y_{1,1}y_{1,2} \\
& K8x[\ ]^2x_{1,2}x_{2,2}y[\ ]y_{1,1}y_{1,2}^2Cx[\ ]^2x_{2,2}^3y[\ ]y_{1,1}^2C2x[\ ]^2x_{2,2}^2y[\ ]y_{1,1}y_{1,2} \\
& K2x[\ ]x_{1,1}^2x_{1,2}y[\ ]^2y_{2,2}^2Kx[\ ]x_{1,1}^2y[\ ]^2y_{1,1}y_{2,2}^2C8x[\ ]x_{1,1}x_{1,2}^2y[\ ]^2y_{1,2}y_{2,2} \\
& C4x[\ ]x_{1,1}x_{1,2}x_{2,2}y[\ ]^2y_{1,1}y_{2,2}K8x[\ ]x_{1,1}x_{1,2}x_{2,2}y[\ ]^2y_{1,2}^2 \\
& C4x[\ ]x_{1,1}x_{1,2}y[\ ]^2y_{1,1}y_{1,2}y_{2,2}C2x[\ ]x_{1,1}x_{2,2}y[\ ]^2y_{1,1}y_{2,2} \\
& K4x[\ ]x_{1,1}x_{2,2}y[\ ]^2y_{1,1}y_{1,2}^2K8x[\ ]x_{1,2}^3y[\ ]^2y_{1,1}y_{2,2}C8x[\ ] \\
& x_{1,2}^2x_{2,2}y[\ ]^2y_{1,1}y_{1,2}K4x[\ ]x_{1,2}^2y[\ ]^2y_{1,1}y_{2,2}^2K2x[\ ]x_{1,2}x_{2,2}^2y[\ ]^2y_{1,1}^2 \\
& C4x[\ ]x_{1,2}x_{2,2}y[\ ]^2y_{1,1}y_{1,2}Kx[\ ]x_{2,2}^2y[\ ]^2y_{1,1}^3Cx_{1,1}^3y[\ ]^3y_{2,2}^2K4 \\
& x_{1,1}^2x_{1,2}y[\ ]^3y_{1,2}y_{2,2}K2x_{1,1}^2x_{2,2}y[\ ]^3y_{1,1}y_{2,2}C4x_{1,1}^2x_{2,2}y[\ ]^3y_{1,2}^2C4x_{1,1} \\
& x_{1,2}^2y[\ ]^3y_{1,1}y_{2,2}K4x_{1,1}x_{1,2}x_{2,2}y[\ ]^3y_{1,1}y_{1,2}Cx_{1,1}x_{2,2}^2y[\ ]^3y_{1,2}^2) / \\
& (4(s^2x_{1,1}y_1y_2y_{2,2}Ks^2x_{1,1}y_{1,2}^2y_{2,2}Ks^2x_{1,2}y_{1,2}^2y_{2,2}Cs^2x_{1,2}y_{1,2}^2y_{1,1}Cs^2x_{2,2} \\
& y_{1,2}^2y_{1,2}Ks^2x_{2,2}y_1y_2y_{1,1}Cstx_1x_{1,1}y_2y_{2,2}K2stx_1x_{1,2}y_1y_{2,2}C2stx_1x_{2,2}y_1y_{1,2} \\
& Kstx_1x_{2,2}y_2y_{1,1}Cstx_2x_{1,1}y_1y_{2,2}K2stx_2x_{1,1}y_2y_{1,2}C2stx_2x_{1,2}y_2y_{1,1} \\
& Kstx_2x_{2,2}y_1y_{1,1}Kt^2x_1^2x_{1,2}y_{2,2}Ct^2x_1^2x_{2,2}y_{1,2}Ct^2x_1x_2x_{1,1}y_{2,2} \\
& Kt^2x_1x_2x_{2,2}y_{1,1}Kt^2x_2^2x_{1,1}y_{1,2}Ct^2x_2^2x_{1,2}y_{1,1}Ksx[\ ]x_{1,1}y_2y_{2,2} \\
& C2sx[\ ]x_{1,2}y_1y_{2,2}K2sx[\ ]x_{2,2}y_1y_{1,2}Csx[\ ]x_{2,2}y_2y_{1,1}Ksx_{1,1}y[\ ]y_1y_{2,2} \\
& C2sx_{1,1}y[\ ]y_2y_{1,2}K2sx_{1,2}y[\ ]y_2y_{1,1}Csx_{2,2}y[\ ]y_1y_{1,1}C2tx[\ ]x_1x_{1,2}y_{2,2}
\end{aligned}$$

$$\begin{aligned}
& K^2 t x [ ] x_1 x_{2,2} y_{1,2} K t x [ ] x_2 x_{1,1} y_{2,2} C t x [ ] x_2 x_{2,2} y_{1,1} K t x_1 x_{1,1} y [ ] y_{2,2} \\
& C t x_1 x_{2,2} y [ ] y_{1,1} C^2 t x_2 x_{1,1} y [ ] y_{1,2} K^2 t x_2 x_{1,2} y [ ] y_{1,1} K x [ ]^2 x_{1,2} y_{2,2} \\
& C x [ ]^2 x_{2,2} y_{1,2} C x [ ] x_{1,1} y [ ] y_{2,2} K x [ ] x_{2,2} y [ ] y_{1,1} K x_{1,1} y [ ]^2 y_{1,2} \\
& C x_{1,2} y [ ]^2 y_{1,1} )^2 (x_2 K y_1)
\end{aligned}$$
